# Supplementary material for: Certified spectral approximation of transfer operators and the Gauss map
Source: arXiv:2602.19435 ancillary file (2026-03-01)
Supplement: Supplementary file 1 [file supplementary_material.pdf]

# Supplementary Material: Certified spectral approximation of transfer operators and the Gauss map

Isaia Nisoli

## Notation

Throughout this supplement we work exclusively on the Hardy space  $H^2(D_1)$  and with the endomorphism  $L := S\mathcal{L} : H^2(D_1) \rightarrow H^2(D_1)$  (see §2 of the main paper). All operator norms  $\|\cdot\|$  are the  $H^2(D_1)$  operator norm; since the shifted monomials  $\{(w-1)^n\}$  form an orthonormal basis in  $H^2(D_1)$ , the matrix norm coincides with the Euclidean spectral norm  $\|\cdot\|_2$ . We write  $L_K := \Pi_K L$  for the Galerkin truncation of rank  $K+1$ , and  $\varepsilon_K := \|L - L_K\| \leq C_2(2/3)^{K+1}$  for the truncation error.

## Computational environment

All computations were performed on a single workstation with the following specifications:

- **Processor:** AMD Ryzen 9 5950X (16 cores, 32 threads via SMT, base 3.4 GHz / boost 4.9 GHz)
- **Memory:** 128 GB DDR4
- **OS:** Ubuntu 22.04.5 LTS (kernel 6.8.0-79)
- **Software:** Julia 1.12.4 with 32 threads; packages: `GKWExperiments.jl`, `BallArithmetic.jl`, `GenericSchur.jl`, `ArbNumerics.jl`

## Data availability

All certified spectral data (eigenvalue enclosures, eigenvector coefficients, Riesz projector norms, and spectral expansion coefficients) are available in machine-readable form at the Harvard DataVerse: <https://doi.org/10.7910/DVN/HKM3Y2>. The full source code for the certification pipeline is available at <https://github.com/orkolorko/GKWExperiments.jl>.

## Computational methodology

The certification pipeline is implemented in two Julia packages: `GKWExperiments.jl` (operator-specific discretization and lift) and `BallArithmetic.jl` (validated linear algebra: Schur certification, resolvent bounds, spectral norm enclosures). Below we describe the role of each script and the main functions it calls.

Table S1: Computational timings for each stage of the certification pipeline. Timings with “(cached)” indicate that the BallMatrix or Schur decomposition was loaded from a previous run.

| Phase                                                                        | Description                                                                 | Wall time |
|------------------------------------------------------------------------------|-----------------------------------------------------------------------------|-----------|
| <i>Script 1: Resolvent certification (full_certification_50eigs.jl)</i>      |                                                                             |           |
| 1a                                                                           | CertifScripts on full $L_{48}$ ( $j = 1\text{--}15$ )                       | < 1 min   |
| 1b                                                                           | Block Schur + CertifScripts on $T_{22}$ , $K = 256$ ( $j = 21\text{--}50$ ) | < 1 min   |
| 1c                                                                           | Fallback: block Schur + CertifScripts, $K = 256$ ( $j = 16\text{--}20$ )    | ~ 2 min   |
| 2                                                                            | Truncation bound + projector errors                                         | < 1 min   |
| 3                                                                            | Tail resolvent on separating circle                                         | ~ 32 s    |
| Total                                                                        |                                                                             | ~ 2.5 min |
| <i>Script 2: Spectral coefficients (spectral_data_50eigs.jl)</i>             |                                                                             |           |
| Schur                                                                        | BigFloat Schur, $K = 256$ , 512-bit (Generic-Schur)                         | ~ 20 min  |
| ordschur                                                                     | $\ell_j(\mathbf{1})$ via ordschur + triangular Sylvester (50 eigs)          | ~ 2 min   |
| <i>Script 3: <math>K = 1024</math> spectral (bigfloat_spectral_K1024.jl)</i> |                                                                             |           |
| Build                                                                        | ArbNumerics matrix, $K = 1024$ , 2048-bit                                   | ~ 25 min  |
| Schur                                                                        | $1025 \times 1025$ GenericSchur at 2048-bit                                 | ~ 18 hr   |
| Quality                                                                      | Residual + orthogonality norms                                              | ~ 2 hr    |
| ordschur                                                                     | $50 \times$ ordschur + Sylvester + perturbation                             | ~ 1 hr    |
| Total                                                                        |                                                                             | ~ 21 hr   |

**Script 1: Resolvent certification (full\_certification\_50eigs.jl).** This script certifies the resolvent of the infinite-dimensional operator on 50 excluding circles  $\Gamma_j$  via the two-stage strategy of §3.3 of the main paper, and computes the Riesz projector errors.

**Phase 0: Matrix construction.** `gkw_matrix_direct(s; K=K)` builds the  $(K+1) \times (K+1)$  Galerkin matrix in Arb arithmetic (ArbNumerics.jl). The truncation error  $\varepsilon_K = C_2 (2/3)^{K+1}$  is computed by `compute_C2` and `compute_Δ`. The Arb matrix is converted to `BallMatrix(BigFloat, M.arb)` for validated linear algebra.

**Phase 1a: Circle sampling at  $K = 48$ .** For  $j = 1, \dots, 15$ , the resolvent  $\|(zI - L_{48})^{-1}\|$  is sampled at 256 equally-spaced points on  $\Gamma_j$  using `CertifScripts.run_certification`. This function computes a certified Schur decomposition  $L_K = QTQ^*$  (`compute_schur_and_error`), bounds the resolvent via Theorem 3.4 of the main paper (`schur_to_original_resolvent`), and returns the supremum  $\sup_{z \in \Gamma_j} \|R_{L_K}(z)\|$ . The small-gain factor  $\alpha_j = \varepsilon_{48} \cdot \sup \|R_{L_{48}}\|$  is computed with directed rounding (`setrounding(Float64, RoundUp)`).

**Phase 1b: Block Schur at  $K = 256$ .** For  $j = 16, \dots, 50$ , the resolvent of  $L_{48}$  is too large. Instead, `certify_eigenvalue_schur_direct` computes a BigFloat Schur form  $L_{256} = QTQ^*$  (GenericSchur.jl), partitions  $T$  around  $\lambda_j$  (Lemma 3.5), and certifies the resolvent supremum on  $\Gamma_j$  via Proposition 3.7. The Schur similarity defect is bounded by Lemma 3.1.

**Phase 2: Infinite-dimensional lift.** For each eigenvalue, the certified finite-dimensional resolvent is lifted to  $L$  via the Neumann perturbation bound  $M_{\infty,j} = \|R_{L_K}\|/(1 - \alpha_j)$ . The

Riesz projector error  $\vartheta_j$  is computed by `projector_approximation_error_rigorous`, and the eigenvalue enclosure follows from Lemma 2.12:  $|\lambda_j - \hat{\lambda}_j| \leq (\varepsilon_K(1+\vartheta_j) + 2C\vartheta_j)/(1-\vartheta_j)$ .

**Phase 3: Tail resolvent.** A separating circle  $|z| = \rho$  in the eigenvalue gap  $|\lambda_{51}| < \rho < |\lambda_{50}|$  is chosen, and the resolvent  $\|R_L\|$  on this circle is certified by the same block Schur method, giving the tail bound constant  $M_\infty$ .

**Script 3: Spectral coefficients** (`bigfloat_spectral_K1024.jl`). This script computes the spectral coefficients  $\ell_j(\mathbf{1})$  at  $K = 1024$  with 2048-bit precision, following the certified Schur pipeline of §3.4 of the main paper.

**Step 1: BallMatrix construction.** `gkw_matrix_direct_fast(s; K=1024, threaded=true)` builds the Arb matrix in  $O(K^3)$  operations. Conversion via `BallMatrix(BigFloat, M_arb)` preserves all 2048 bits of center precision (no Float64 truncation).

**Step 2: BigFloat Schur decomposition.** `GenericSchur.schur` computes  $L_K = QTQ^*$  at 2048-bit precision. The Schur residual  $\|L_K - QTQ^*\|$  and orthogonality defect  $\|Q^*Q - I\|$  are certified via `upper_bound_L2_opnorm(BallMatrix(...))`, giving the total enclosure error  $\|E\|$  (Lemma 3.1).

**Step 3: Ordered Schur and triangular solve.** For each  $j = 1, \dots, 50$ , `bigfloat_ordschur` reorders the Schur form to place  $\lambda_j$  in position  $(1,1)$  via Givens rotations. The spectral coefficient is extracted by the direct triangular solve:  $q = \overline{Q_{\text{ord},1,:}}$ ,  $z = (T_{22} - \lambda_j I)^{-1} q_{\text{rest}}$ ,  $\ell_j(\mathbf{1}) = \text{Re}(q_1 - \sum_i T_{12,i} z_i)$ . The ordschur quality (reordering residual and orthogonality) is tracked via `upper_bound_L2_opnorm`.

**Step 4: Perturbation bound.** The total certified error  $\delta$  on  $\ell_j(\mathbf{1})$  is dominated by the Schur similarity defect  $\|E\|$ ; the triangular solve residual is negligible ( $\sim 10^{-309}$  at 1024-bit). Sign certification holds when  $|\ell_j(\mathbf{1})| > \delta$ .

An analogous script `bigfloat_spectral_K1024.jl` performs the same computation at  $K = 1024$  with 2048-bit precision for cross-validation.

**Tail bound** (`compute_tail_bound_N50.jl`). This script computes the rigorous tail bound for the spectral remainder  $R_{50}(n)$ . It loads the certified spectral data from Script 3 and the tail resolvent from Script 1, constructs componentwise ball vectors for each Riesz projector  $P_j(\mathbf{1})$  ( $j = 1, \dots, 50$ ), computes the tail projection  $Q_{50}\mathbf{1} = \mathbf{1} - \sum_j P_j\mathbf{1}$  using interval arithmetic with directed rounding (triangle inequality), and adds an infinite-dimensional correction  $\sum_j \varepsilon_K / \text{sep}_j$  to lift from the Galerkin approximation  $L_K$  to the full operator  $L$ . The final output is  $\|R_{50}(n)\| \leq \rho^{n+1} \cdot M_\infty \cdot \|Q_{50}\mathbf{1}\|$ .

Table S2: Two-stage certification parameters

| Parameter              | Value                                                |
|------------------------|------------------------------------------------------|
| $K_{\text{low}}$       | 48 (eigenvalues 1–15), 256 (eigenvalues 16–50)       |
| $K_{\text{high}}$      | 256                                                  |
| $C_2$                  | $1.005810 \times 10^1$                               |
| $\varepsilon_{48}$     | $2.366161 \times 10^{-8}$                            |
| $\varepsilon_{256}$    | $5.585504 \times 10^{-45}$                           |
| Circle samples         | 256                                                  |
| Method ( $j = 1$ –15)  | CertifScripts circle certification on full $L_{48}$  |
| Method ( $j = 16$ –50) | Block Schur at $K = 256$ + CertifScripts on $T_{22}$ |

Table S3: Two-stage certification results for the first 50 eigenvalues of the GKW operator ( $s = 1$ ). The column  $\alpha_1 = \varepsilon_{K_{\text{low}}} \cdot \|R_{L_{K_{\text{low}}}}(z)\|$  is the small-gain factor on the excluding circle  $\Gamma_j$ . All 50 eigenvalues satisfy  $\alpha_1 < 1$ , proving simplicity and giving certified resolvent bounds. The “Eval. encl.” column gives the eigenvalue error radius from projector control (Lemma 2.12). For  $j = 1$ –15, resolvent sampling on the full  $L_{48}$ ; for  $j = 16$ –50, block Schur at  $K = 256$  with certified resolvent on  $T_{22}$ .

| $j$ | $\hat{\lambda}_j$ | $K_{\text{low}}$ | $\alpha_1$             | Circle $r$             | Eval. encl.            | Riesz proj. err        |
|-----|-------------------|------------------|------------------------|------------------------|------------------------|------------------------|
| 1   | +1.0000000000     | 48               | $1.01 \times 10^{-5}$  | $1.00 \times 10^{-2}$  | $7.40 \times 10^{-45}$ | $1.01 \times 10^{-41}$ |
| 2   | −0.3036630029     | 48               | $3.53 \times 10^{-5}$  | $3.04 \times 10^{-3}$  | $2.33 \times 10^{-44}$ | $3.77 \times 10^{-41}$ |
| 3   | +0.1008845093     | 48               | $1.11 \times 10^{-4}$  | $1.01 \times 10^{-3}$  | $7.32 \times 10^{-44}$ | $1.23 \times 10^{-40}$ |
| 4   | −0.0354961590     | 48               | $3.24 \times 10^{-4}$  | $3.55 \times 10^{-4}$  | $2.17 \times 10^{-43}$ | $3.73 \times 10^{-40}$ |
| 5   | +0.0128437904     | 48               | $9.15 \times 10^{-4}$  | $1.28 \times 10^{-4}$  | $6.22 \times 10^{-43}$ | $1.08 \times 10^{-39}$ |
| 6   | −4.7177775e − 03  | 48               | $2.52 \times 10^{-3}$  | $4.72 \times 10^{-5}$  | $1.75 \times 10^{-42}$ | $3.01 \times 10^{-39}$ |
| 7   | +1.7486751e − 03  | 48               | $6.85 \times 10^{-3}$  | $1.75 \times 10^{-5}$  | $4.85 \times 10^{-42}$ | $8.29 \times 10^{-39}$ |
| 8   | −6.5202086e − 04  | 48               | $1.84 \times 10^{-2}$  | $6.52 \times 10^{-6}$  | $1.33 \times 10^{-41}$ | $2.29 \times 10^{-38}$ |
| 9   | +2.4413147e − 04  | 48               | $4.91 \times 10^{-2}$  | $2.44 \times 10^{-6}$  | $3.63 \times 10^{-41}$ | $6.49 \times 10^{-38}$ |
| 10  | −9.1689084e − 05  | 48               | $1.30 \times 10^{-1}$  | $9.17 \times 10^{-7}$  | $9.85 \times 10^{-41}$ | $2.05 \times 10^{-37}$ |
| 11  | +3.4516546e − 05  | 48               | $3.44 \times 10^{-1}$  | $3.45 \times 10^{-7}$  | $2.66 \times 10^{-40}$ | $9.48 \times 10^{-37}$ |
| 12  | −1.3017698e − 05  | 48               | $4.99 \times 10^{-1}$  | $2.37 \times 10^{-7}$  | $7.16 \times 10^{-40}$ | $2.34 \times 10^{-36}$ |
| 13  | +4.9167823e − 06  | 48               | $4.97 \times 10^{-1}$  | $2.37 \times 10^{-7}$  | $1.92 \times 10^{-39}$ | $2.31 \times 10^{-36}$ |
| 14  | −1.8593074e − 06  | 48               | $5.01 \times 10^{-1}$  | $2.37 \times 10^{-7}$  | $5.15 \times 10^{-39}$ | $2.38 \times 10^{-36}$ |
| 15  | +7.0381134e − 07  | 48               | $6.21 \times 10^{-1}$  | $2.01 \times 10^{-7}$  | $1.38 \times 10^{-38}$ | $5.36 \times 10^{-36}$ |
| 16  | −2.6664134e − 07  | 256              | $8.11 \times 10^{-32}$ | $1.14 \times 10^{-7}$  | $3.67 \times 10^{-38}$ | $1.34 \times 10^{-25}$ |
| 17  | +1.0109055e − 07  | 256              | $5.48 \times 10^{-31}$ | $4.33 \times 10^{-8}$  | $9.78 \times 10^{-38}$ | $2.33 \times 10^{-24}$ |
| 18  | −3.8349698e − 08  | 256              | $3.70 \times 10^{-30}$ | $1.64 \times 10^{-8}$  | $2.60 \times 10^{-37}$ | $4.02 \times 10^{-23}$ |
| 19  | +1.4556138e − 08  | 256              | $2.50 \times 10^{-29}$ | $6.23 \times 10^{-9}$  | $6.91 \times 10^{-37}$ | $6.96 \times 10^{-22}$ |
| 20  | −5.5275679e − 09  | 256              | $1.69 \times 10^{-28}$ | $2.36 \times 10^{-9}$  | $1.84 \times 10^{-36}$ | $1.20 \times 10^{-20}$ |
| 21  | +2.0999136e − 09  | 256              | $1.14 \times 10^{-27}$ | $8.98 \times 10^{-10}$ | $4.87 \times 10^{-36}$ | $2.08 \times 10^{-19}$ |
| 22  | −7.9804577e − 10  | 256              | $7.68 \times 10^{-27}$ | $3.41 \times 10^{-10}$ | $1.29 \times 10^{-35}$ | $3.60 \times 10^{-18}$ |
| 23  | +3.0338629e − 10  | 256              | $5.18 \times 10^{-26}$ | $1.30 \times 10^{-10}$ | $3.41 \times 10^{-35}$ | $6.23 \times 10^{-17}$ |

continued

| $j$ | $\hat{\lambda}_j$  | $K_{\text{low}}$ | $\alpha_1$             | Circle $r$             | Eval. encl.            | Riesz proj. err        |
|-----|--------------------|------------------|------------------------|------------------------|------------------------|------------------------|
| 24  | $-1.1536954e - 10$ | 256              | $3.49 \times 10^{-25}$ | $4.93 \times 10^{-11}$ | $9.02 \times 10^{-35}$ | $1.08 \times 10^{-15}$ |
| 25  | $+4.3883450e - 11$ | 256              | $2.36 \times 10^{-24}$ | $1.88 \times 10^{-11}$ | $2.38 \times 10^{-34}$ | $1.87 \times 10^{-14}$ |
| 26  | $-1.6696052e - 11$ | 256              | $1.59 \times 10^{-23}$ | $7.14 \times 10^{-12}$ | $6.29 \times 10^{-34}$ | $3.25 \times 10^{-13}$ |
| 27  | $+6.3536124e - 12$ | 256              | $1.08 \times 10^{-22}$ | $2.72 \times 10^{-12}$ | $1.66 \times 10^{-33}$ | $5.67 \times 10^{-12}$ |
| 28  | $-2.4183168e - 12$ | 256              | $7.38 \times 10^{-22}$ | $1.03 \times 10^{-12}$ | $4.38 \times 10^{-33}$ | $1.01 \times 10^{-10}$ |
| 29  | $+9.2062742e - 13$ | 256              | $5.15 \times 10^{-21}$ | $3.94 \times 10^{-13}$ | $1.16 \times 10^{-32}$ | $1.87 \times 10^{-9}$  |
| 30  | $-3.5053094e - 13$ | 256              | $3.83 \times 10^{-20}$ | $1.50 \times 10^{-13}$ | $3.06 \times 10^{-32}$ | $3.93 \times 10^{-8}$  |
| 31  | $+1.3348571e - 13$ | 256              | $3.52 \times 10^{-19}$ | $5.71 \times 10^{-14}$ | $8.08 \times 10^{-32}$ | $1.26 \times 10^{-6}$  |
| 32  | $-5.0839831e - 14$ | 256              | $5.08 \times 10^{-17}$ | $2.17 \times 10^{-14}$ | $2.14 \times 10^{-31}$ | $1.00 \times 10^{-2}$  |
| 33  | $+1.9365544e - 14$ | 256              | $2.58 \times 10^{-18}$ | $8.28 \times 10^{-15}$ | $5.63 \times 10^{-31}$ | $9.86 \times 10^{-6}$  |
| 34  | $-7.3774705e - 15$ | 256              | $1.74 \times 10^{-17}$ | $3.15 \times 10^{-15}$ | $1.52 \times 10^{-30}$ | $1.71 \times 10^{-4}$  |
| 35  | $+2.8108246e - 15$ | 256              | $1.17 \times 10^{-16}$ | $1.20 \times 10^{-15}$ | $5.55 \times 10^{-30}$ | $2.96 \times 10^{-3}$  |
| 36  | $-1.0710387e - 15$ | 256              | $7.90 \times 10^{-16}$ | $4.58 \times 10^{-16}$ | $\infty$               | $5.12 \times 10^{-2}$  |
| 37  | $+4.0814893e - 16$ | 256              | $5.33 \times 10^{-15}$ | $1.74 \times 10^{-16}$ | $\infty$               | $8.86 \times 10^{-1}$  |
| 38  | $-1.5555055e - 16$ | 256              | $3.59 \times 10^{-14}$ | $6.65 \times 10^{-17}$ | $\infty$               | $> 1$                  |
| 39  | $+5.9287246e - 17$ | 256              | $2.42 \times 10^{-13}$ | $2.53 \times 10^{-17}$ | $\infty$               | $> 1$                  |
| 40  | $-2.2598811e - 17$ | 256              | $1.63 \times 10^{-12}$ | $9.66 \times 10^{-18}$ | $\infty$               | $> 1$                  |
| 41  | $+8.6147444e - 18$ | 256              | $1.10 \times 10^{-11}$ | $3.68 \times 10^{-18}$ | $\infty$               | $> 1$                  |
| 42  | $-3.2842013e - 18$ | 256              | $7.41 \times 10^{-11}$ | $1.40 \times 10^{-18}$ | $\infty$               | $> 1$                  |
| 43  | $+1.2521200e - 18$ | 256              | $4.99 \times 10^{-10}$ | $5.35 \times 10^{-19}$ | $\infty$               | $> 1$                  |
| 44  | $-4.7740757e - 19$ | 256              | $3.36 \times 10^{-9}$  | $2.04 \times 10^{-19}$ | $\infty$               | $> 1$                  |
| 45  | $+1.8203644e - 19$ | 256              | $2.27 \times 10^{-8}$  | $7.78 \times 10^{-20}$ | $\infty$               | $> 1$                  |
| 46  | $-6.9414738e - 20$ | 256              | $1.53 \times 10^{-7}$  | $2.97 \times 10^{-20}$ | $\infty$               | $> 1$                  |
| 47  | $+2.6470860e - 20$ | 256              | $1.03 \times 10^{-6}$  | $1.13 \times 10^{-20}$ | $\infty$               | $> 1$                  |
| 48  | $-1.0094998e - 20$ | 256              | $6.93 \times 10^{-6}$  | $4.31 \times 10^{-21}$ | $\infty$               | $> 1$                  |
| 49  | $+3.8500394e - 21$ | 256              | $4.66 \times 10^{-5}$  | $1.64 \times 10^{-21}$ | $\infty$               | $> 1$                  |
| 50  | $-1.4683981e - 21$ | 256              | $3.14 \times 10^{-4}$  | $6.27 \times 10^{-22}$ | $\infty$               | $> 1$                  |

Table S4: Certified resolvent bounds.  $\|R_{L_{K_{\text{low}}}}\|$  is the resolvent of the finite-dimensional Galerkin matrix on the excluding circle  $\Gamma_j$ , certified via resolvent sampling (Phase 1a) or Schur direct method (Phase 1b/c).  $M_\infty = \|R_L(z)\|$  is the certified resolvent bound for the infinite-dimensional operator via Neumann perturbation:  $M_\infty \leq \|R_{L_{K_{\text{low}}}}\|/(1 - \alpha_1)$ . The transfer columns give  $\|R_{L_{K_{\text{high}}}}\|$  via reverse perturbation at  $K_{\text{high}} = 256$ .

| $j$ | $K_{\text{low}}$ | $\ R_{L_{K_{\text{low}}}}\ $ | $M_\infty = \ R_L\ $ | $\alpha_{\text{high}}$ | $\ R_{L_{K_{\text{high}}}}\ $ |
|-----|------------------|------------------------------|----------------------|------------------------|-------------------------------|
| 1   | 48               | $4.25 \times 10^2$           | $4.25 \times 10^2$   | $2.37 \times 10^{-42}$ | $4.25 \times 10^2$            |
| 2   | 48               | $1.49 \times 10^3$           | $1.49 \times 10^3$   | $8.33 \times 10^{-42}$ | $1.49 \times 10^3$            |
| 3   | 48               | $4.67 \times 10^3$           | $4.67 \times 10^3$   | $2.61 \times 10^{-41}$ | $4.67 \times 10^3$            |
| 4   | 48               | $1.37 \times 10^4$           | $1.37 \times 10^4$   | $7.66 \times 10^{-41}$ | $1.37 \times 10^4$            |
| 5   | 48               | $3.87 \times 10^4$           | $3.87 \times 10^4$   | $2.16 \times 10^{-40}$ | $3.87 \times 10^4$            |

*continued*

| $j$ | $K_{\text{low}}$ | $\ R_{L_{K_{\text{low}}}}\ $ | $M_{\infty} = \ R_L\ $ | $\alpha_{\text{high}}$ | $\ R_{L_{K_{\text{high}}}}\ $ |
|-----|------------------|------------------------------|------------------------|------------------------|-------------------------------|
| 6   | 48               | $1.07 \times 10^5$           | $1.07 \times 10^5$     | $5.97 \times 10^{-40}$ | $1.07 \times 10^5$            |
| 7   | 48               | $2.89 \times 10^5$           | $2.91 \times 10^5$     | $1.63 \times 10^{-39}$ | $2.91 \times 10^5$            |
| 8   | 48               | $7.78 \times 10^5$           | $7.92 \times 10^5$     | $4.43 \times 10^{-39}$ | $7.92 \times 10^5$            |
| 9   | 48               | $2.07 \times 10^6$           | $2.18 \times 10^6$     | $1.22 \times 10^{-38}$ | $2.18 \times 10^6$            |
| 10  | 48               | $5.50 \times 10^6$           | $6.33 \times 10^6$     | $3.53 \times 10^{-38}$ | $6.33 \times 10^6$            |
| 11  | 48               | $1.45 \times 10^7$           | $2.22 \times 10^7$     | $1.24 \times 10^{-37}$ | $2.22 \times 10^7$            |
| 12  | 48               | $2.11 \times 10^7$           | $4.21 \times 10^7$     | $2.35 \times 10^{-37}$ | $4.21 \times 10^7$            |
| 13  | 48               | $2.10 \times 10^7$           | $4.18 \times 10^7$     | $2.34 \times 10^{-37}$ | $4.18 \times 10^7$            |
| 14  | 48               | $2.12 \times 10^7$           | $4.24 \times 10^7$     | $2.37 \times 10^{-37}$ | $4.24 \times 10^7$            |
| 15  | 48               | $2.62 \times 10^7$           | $6.91 \times 10^7$     | $3.86 \times 10^{-37}$ | $6.91 \times 10^7$            |
| 16  | 256              | $1.45 \times 10^{13}$        | $1.45 \times 10^{13}$  | $8.11 \times 10^{-32}$ | $1.45 \times 10^{13}$         |
| 17  | 256              | $9.81 \times 10^{13}$        | $9.81 \times 10^{13}$  | $5.48 \times 10^{-31}$ | $9.81 \times 10^{13}$         |
| 18  | 256              | $6.63 \times 10^{14}$        | $6.63 \times 10^{14}$  | $3.70 \times 10^{-30}$ | $6.63 \times 10^{14}$         |
| 19  | 256              | $4.47 \times 10^{15}$        | $4.47 \times 10^{15}$  | $2.50 \times 10^{-29}$ | $4.47 \times 10^{15}$         |
| 20  | 256              | $3.02 \times 10^{16}$        | $3.02 \times 10^{16}$  | $1.69 \times 10^{-28}$ | $3.02 \times 10^{16}$         |
| 21  | 256              | $2.04 \times 10^{17}$        | $2.04 \times 10^{17}$  | $1.14 \times 10^{-27}$ | $2.04 \times 10^{17}$         |
| 22  | 256              | $1.37 \times 10^{18}$        | $1.37 \times 10^{18}$  | $7.68 \times 10^{-27}$ | $1.37 \times 10^{18}$         |
| 23  | 256              | $9.27 \times 10^{18}$        | $9.27 \times 10^{18}$  | $5.18 \times 10^{-26}$ | $9.27 \times 10^{18}$         |
| 24  | 256              | $6.26 \times 10^{19}$        | $6.26 \times 10^{19}$  | $3.49 \times 10^{-25}$ | $6.26 \times 10^{19}$         |
| 25  | 256              | $4.22 \times 10^{20}$        | $4.22 \times 10^{20}$  | $2.36 \times 10^{-24}$ | $4.22 \times 10^{20}$         |
| 26  | 256              | $2.85 \times 10^{21}$        | $2.85 \times 10^{21}$  | $1.59 \times 10^{-23}$ | $2.85 \times 10^{21}$         |
| 27  | 256              | $1.93 \times 10^{22}$        | $1.93 \times 10^{22}$  | $1.08 \times 10^{-22}$ | $1.93 \times 10^{22}$         |
| 28  | 256              | $1.32 \times 10^{23}$        | $1.32 \times 10^{23}$  | $7.38 \times 10^{-22}$ | $1.32 \times 10^{23}$         |
| 29  | 256              | $9.22 \times 10^{23}$        | $9.22 \times 10^{23}$  | $5.15 \times 10^{-21}$ | $9.22 \times 10^{23}$         |
| 30  | 256              | $6.85 \times 10^{24}$        | $6.85 \times 10^{24}$  | $3.83 \times 10^{-20}$ | $6.85 \times 10^{24}$         |
| 31  | 256              | $6.30 \times 10^{25}$        | $6.30 \times 10^{25}$  | $3.52 \times 10^{-19}$ | $6.30 \times 10^{25}$         |
| 32  | 256              | $9.09 \times 10^{27}$        | $9.09 \times 10^{27}$  | $5.08 \times 10^{-17}$ | $9.09 \times 10^{27}$         |
| 33  | 256              | $4.62 \times 10^{26}$        | $4.62 \times 10^{26}$  | $2.58 \times 10^{-18}$ | $4.62 \times 10^{26}$         |
| 34  | 256              | $3.11 \times 10^{27}$        | $3.11 \times 10^{27}$  | $1.74 \times 10^{-17}$ | $3.11 \times 10^{27}$         |
| 35  | 256              | $2.10 \times 10^{28}$        | $2.10 \times 10^{28}$  | $1.17 \times 10^{-16}$ | $2.10 \times 10^{28}$         |
| 36  | 256              | $1.41 \times 10^{29}$        | $1.41 \times 10^{29}$  | $7.90 \times 10^{-16}$ | $1.41 \times 10^{29}$         |
| 37  | 256              | $9.54 \times 10^{29}$        | $9.54 \times 10^{29}$  | $5.33 \times 10^{-15}$ | $9.54 \times 10^{29}$         |
| 38  | 256              | $6.43 \times 10^{30}$        | $6.43 \times 10^{30}$  | $3.59 \times 10^{-14}$ | $6.43 \times 10^{30}$         |
| 39  | 256              | $4.33 \times 10^{31}$        | $4.33 \times 10^{31}$  | $2.42 \times 10^{-13}$ | $4.33 \times 10^{31}$         |
| 40  | 256              | $2.92 \times 10^{32}$        | $2.92 \times 10^{32}$  | $1.63 \times 10^{-12}$ | $2.92 \times 10^{32}$         |
| 41  | 256              | $1.97 \times 10^{33}$        | $1.97 \times 10^{33}$  | $1.10 \times 10^{-11}$ | $1.97 \times 10^{33}$         |
| 42  | 256              | $1.33 \times 10^{34}$        | $1.33 \times 10^{34}$  | $7.41 \times 10^{-11}$ | $1.33 \times 10^{34}$         |
| 43  | 256              | $8.93 \times 10^{34}$        | $8.93 \times 10^{34}$  | $4.99 \times 10^{-10}$ | $8.94 \times 10^{34}$         |
| 44  | 256              | $6.02 \times 10^{35}$        | $6.02 \times 10^{35}$  | $3.36 \times 10^{-9}$  | $6.02 \times 10^{35}$         |
| 45  | 256              | $4.06 \times 10^{36}$        | $4.06 \times 10^{36}$  | $2.27 \times 10^{-8}$  | $4.06 \times 10^{36}$         |
| 46  | 256              | $2.73 \times 10^{37}$        | $2.73 \times 10^{37}$  | $1.53 \times 10^{-7}$  | $2.73 \times 10^{37}$         |
| 47  | 256              | $1.84 \times 10^{38}$        | $1.84 \times 10^{38}$  | $1.03 \times 10^{-6}$  | $1.84 \times 10^{38}$         |
| 48  | 256              | $1.24 \times 10^{39}$        | $1.24 \times 10^{39}$  | $6.93 \times 10^{-6}$  | $1.24 \times 10^{39}$         |
| 49  | 256              | $8.35 \times 10^{39}$        | $8.35 \times 10^{39}$  | $4.66 \times 10^{-5}$  | $8.35 \times 10^{39}$         |

continued

| $j$ | $K_{\text{low}}$ | $\ R_{L_{K_{\text{low}}}}\ $ | $M_{\infty} = \ R_L\ $ | $\alpha_{\text{high}}$ | $\ R_{L_{K_{\text{high}}}}\ $ |
|-----|------------------|------------------------------|------------------------|------------------------|-------------------------------|
| 50  | 256              | $5.62 \times 10^{40}$        | $5.63 \times 10^{40}$  | $3.14 \times 10^{-4}$  | $5.63 \times 10^{40}$         |

**Theorem S1** (Rigorous spectral certification of the GKW operator). *Let  $L := S\mathcal{L} : H^2(D_1) \rightarrow H^2(D_1)$  be the GKW transfer operator for  $s = 1$  (see §2 of the main paper). The first 50 eigenvalues  $\lambda_1, \dots, \lambda_{50}$  (ordered by decreasing modulus) are simple: all 50 excluding circles  $\Gamma_j \subset \rho(L)$  are certified via the two-stage resolvent method (Table S3). For all 50 eigenvalues, projector control (Lemma 2.12) at  $K = 1024$  (2048-bit precision) yields eigenvalue enclosures  $|\lambda_j - \hat{\lambda}_j| \leq \delta_{\lambda,j}$ , with full-precision centers  $\hat{\lambda}_j$  and certified radii  $\delta_{\lambda,j}$  listed in Table S5. Projector errors satisfy  $\vartheta_j := \|P_L(\Gamma_j) - P_{L_{1024}}(\Gamma_j)\| \leq \frac{|\Gamma_j|}{2\pi} \cdot \frac{M_{\infty,j}^2 \cdot \varepsilon_{1024}}{1 - \alpha_j}$ , ranging from  $\vartheta_1 \leq 5.84 \times 10^{-177}$  to  $\vartheta_{50} \leq 6.41 \times 10^{-120}$ . Here  $\Gamma_j$  is the excluding circle of radius listed in Table S3 centered at  $\hat{\lambda}_j$ .*

**Method.** For  $j = 1, \dots, 15$ , Stage 1 certifies that  $\Gamma_j \subset \rho(L)$  by verifying  $\alpha_j = \varepsilon_{K_{\text{low}}} \cdot \sup_{z \in \Gamma_j} \|R_{L_{K_{\text{low}}}}(z)\| < 1$  via resolvent sampling with 256 points on  $\Gamma_j$ , using the Galerkin matrix  $L_{48}$  of size  $K_{\text{low}} + 1 = 49$ . For  $j = 16, \dots, 50$ , the Schur direct method at  $K = 256$  provides resolvent certification via block triangular structure of the certified Schur form, without resolvent sampling. Eigenvalue enclosures are obtained from projector control (Lemma 2.12) at  $K = 1024$ : since each  $\lambda_j$  is certified simple and  $\vartheta_j < 1$ , the eigenvalue error satisfies  $|\lambda_j - \hat{\lambda}_j| \leq (\varepsilon_K(1 + \vartheta_j) + 2C\vartheta_j)/(1 - \vartheta_j)$ , where  $C = \|L_K\| \leq \|L\| \leq C_2$  and  $\vartheta_j$  is the Riesz projector error. The Riesz projector error is bounded via  $\vartheta_j \leq \frac{|\Gamma_j|}{2\pi} \cdot \frac{M_{\infty,j}^2 \cdot \varepsilon_K}{1 - \alpha_j}$ , where  $M_{\infty,j}$  is the certified infinite-dimensional resolvent and  $\varepsilon_K = \varepsilon_{1024}$  is the truncation error at  $K = 1024$ . The tail resolvent on the separating circle gives  $\|R_L\|_{(\Gamma_{\text{tail}})} \leq 6.06 \times 10^{41}$  with effective spectral radius  $\rho_{\text{tail}} \approx 1.01 \times 10^{-21}$ . All scalar bounds use directed rounding to ensure rigor.

# Rigorous Spectral Expansion

Since all 50 eigenvalues are certified to be simple (Theorem S1), each eigenvalue  $\lambda_j$  has a rank-one Riesz projector  $P_j = v_j \otimes \ell_j$ , where  $v_j$  is the right eigenvector ( $\|v_j\| = 1$ ) and  $\ell_j$  the left (dual) eigenvector, normalized so that  $\ell_j(v_j) = 1$ . The spectral expansion of  $L^n$  applied to the constant function  $\mathbf{1}$  is

$$L^n \mathbf{1} = \sum_{j=1}^N \lambda_j^n \ell_j(\mathbf{1}) v_j + R_N(n), \quad (\text{S1})$$

where  $\ell_j(\mathbf{1}) = \langle P_j(\mathbf{1}), v_j \rangle$  is the spectral coefficient and  $R_N(n)$  is bounded by  $|\lambda_{N+1}|^n$  times the tail projector norm.

**Computation of  $\ell_j(\mathbf{1})$  at  $K = 256$ .** The Galerkin matrix  $L_{256}$  is built in high-precision arithmetic (ArbNumerics, 512 bits) and rigorously converted to a `BallMatrix` with `BigFloat` centers. A direct `BigFloat` Schur decomposition  $L_{256} = QTQ'$  is computed via `GenericSchur.jl`, achieving residual  $\|L_{256} - QTQ'\| \leq 2.82 \times 10^{-24}$  (before refinement) and orthogonality defect  $\|Q'Q - I\| \leq 1.75 \times 10^{-153}$ . The total Schur enclosure error is  $\|E\| = \|L_{256} - QTQ'\| \leq 4.96 \times 10^{-154}$ . For each eigenvalue  $\lambda_j$ , a `BigFloat` `ordschur` reorders the target eigenvalue to position (1, 1), and the left eigenvector functional  $\ell_j$  is recovered via Sylvester equation: with  $T = \begin{bmatrix} \lambda_j & T_{12} \\ 0 & T_{22} \end{bmatrix}$ , the solution  $z_0 = (T_{22} - \lambda_j I)^{-1} q_{\text{rest}}$  gives  $\ell_j(\mathbf{1}) = q_1 - T_{12} \cdot z_0$ , where  $q = \overline{Q_{\text{ord},1,:}}$  ( $= Q_{\text{ord}}^* e_1$ ). The certified error  $\delta$  is dominated by the Schur similarity defect  $\|E\| \leq r_{\text{sch}} \sqrt{1 + \delta_{\text{orth}}} + C_A \delta_{\text{orth}}$  (Lemma 3.1); the triangular solve residual is negligible ( $\sim 10^{-309}$  at 1024-bit). All 35 coefficients ( $j = 1, \dots, 35$ ) are certified with  $|\ell_j(\mathbf{1})| > \delta$  at  $K = 256$ .

**Computation of  $\ell_j(\mathbf{1})$  at  $K = 1024$ .** At  $K = 1024$  with 2048-bit precision ( $\approx 616$  decimal digits), the Schur enclosure error drops to  $\|E\| \leq 5.72 \times 10^{-317}$ , and all 50 coefficients are sign-certified with radii at the  $10^{-282}$ – $10^{-316}$  level. This provides independent confirmation of the  $K = 256$  results and extends certification to eigenvalues 36–50.

**Table S5: Certified eigenvalue enclosures** ( $K = 1024$ ,  $P = 2048$ ). Each center  $\hat{\lambda}_j$  is displayed to full certified precision; the true eigenvalue satisfies  $|\lambda_j - \hat{\lambda}_j| \leq \delta_\lambda$ .

$$\hat{\lambda}_1 = 0.\text{99999 99999 99999 99999 99999 99999 99999 99999 99999 99999}$$
$$\text{99999 99999 99999 99999 99999 99999 99999 99999 99999 99999}$$
$$\text{99999 99999 99999 99999 99999 99999 99999 99999 99999 99999}$$
$$\text{99999 99999 99999 99999 99999 9999}$$

$$|\lambda_1 - \hat{\lambda}_1| \leq 1.28 \times 10^{-176}.$$

$$\hat{\lambda}_2 = -0.30366\ 30028\ 98732\ 65859\ 74481\ 21901\ 55623\ 31108\ 77352\ 25365\ 78951\ 88245\ 48146\ 72269\ 95294\ 24691\ 09843\ 40811\ 93436\ 36368\ 11098\ 27226\ 37106\ 16938\ 47461\ 48597\ 45801\ 31606\ 52653\ 81818\ 23787\ 91324\ 46139\ 89647\ 64297\ 4095$$

$$|\lambda_2 - \hat{\lambda}_2| \leq 4.78 \times 10^{-176}.$$

$$\hat{\lambda}_3 = 0.10088\,45092\,93104\,07530\,56376\,42992\,48624\,74444\,81593\,43167\,53370\,03907\,25964\,27590\,07927\,81841\,67247\,32621\,01762\,28045\,39685\,23188\,01770\,94416\,58435\,54872\,60239\,64040\,11083\,38360\,85141\,12346\,48669\,39374\,35335\,477$$

$$|\lambda_3 - \hat{\lambda}_3| \leq 1.56 \times 10^{-175}.$$

$$\hat{\lambda}_4 = -0.03549\,61590\,21659\,84540\,88916\,81134\,69699\,95131\,87327\,16359\,08886\,06988\,41890\,25177\,24145\,40691\,08539\,26275\,13976\,08788\,91062\,18902\,64418\,30742\,58746\,18397\,21688\,88672\,39537\,20853\,61326\,10750\,30125\,79606\,10577\,499$$

$$|\lambda_4 - \hat{\lambda}_4| \leq 4.73 \times 10^{-175}.$$

$$\hat{\lambda}_5 = 0.01284\,37903\,62440\,26481\,51602\,95302\,06302\,17224\,89539\,01888\,22097\,91312\,74460\,79017\,50484\,65465\,21591\,30219\,18680\,50642\,84700\,73120\,44195\,91396\,38638\,86171\,77410\,53992\,08984\,25769\,86252\,80881\,21157\,88121\,85149\,76$$

$$|\lambda_5 - \hat{\lambda}_5| \leq 1.37 \times 10^{-174}.$$

$$\hat{\lambda}_6 = -0.00471\,77775\,11571\,03107\,38754\,74999\,04633\,33223\,23342\,08299\,96846\,62822\,16479\,72129\,39521\,02944\,89588\,85554\,34586\,13760\,69150\,91817\,22351\,54199\,33246\,96147\,94166\,91810\,49289\,61157\,88418\,21627\,38836\,89162\,06732\,45$$

$$|\lambda_6 - \hat{\lambda}_6| \leq 3.82 \times 10^{-174}.$$

$$\hat{\lambda}_7 = 0.00174\,86751\,24305\,51191\,33117\,09674\,65212\,02156\,14465\,28114\,53628\,73710\,81591\,47512\,40452\,43229\,45054\,03543\,11822\,72779\,29883\,63325\,93290\,11560\,74134\,66268\,40073\,37559\,07505\,11214\,68611\,74824\,98241\,62367\,23102\,3$$

$$|\lambda_7 - \hat{\lambda}_7| \leq 1.05 \times 10^{-173}.$$

$$\hat{\lambda}_8 = -0.00065\,20208\,58320\,50290\,03302\,67784\,80928\,43706\,09589\,22214\,49882\,79381\,53508\,39604\,11175\,97241\,55403\,57982\,37411\,84677\,50651\,40193\,96349\,17024\,74659\,13396\,52703\,74260\,36432\,80774\,51882\,50357\,32102\,42442\,02259\,5$$

$$|\lambda_8 - \hat{\lambda}_8| \leq 2.90 \times 10^{-173}.$$

$$\begin{aligned} \hat{\lambda}_9 = & 0.00024\,41314\,65524\,51581\,21368\,50477\,91634\,93183\,68626\,21732 \\ & 22584\,16048\,18382\,67046\,41834\,46770\,18409\,10474\,62614\,27634 \\ & 18677\,04610\,06777\,48402\,32041\,26399\,18677\,32541\,06686\,69665 \\ & 30203\,87583\,52810\,99623\,95991\,3 \end{aligned}$$

$$|\lambda_9 - \hat{\lambda}_9| \leq 8.24 \times 10^{-173}.$$

$$\begin{aligned} \hat{\lambda}_{10} = & -0.00009\,16890\,83768\,59330\,29776\,86737\,14391\,00329\,38646\,15324 \\ & 26983\,28589\,48927\,48213\,93718\,25777\,19803\,73573\,90445\,52766 \\ & 84347\,32865\,75174\,26397\,71857\,48706\,73283\,32698\,13522\,83744 \\ & 84885\,70238\,51271\,90504\,35350 \end{aligned}$$

$$|\lambda_{10} - \hat{\lambda}_{10}| \leq 2.60 \times 10^{-172}.$$

$$\begin{aligned} \hat{\lambda}_{11} = & 0.00003\,45165\,46163\,85425\,33132\,47959\,13947\,83868\,80526\,92159 \\ & 08520\,86311\,76301\,91043\,30995\,59212\,28709\,71491\,39101\,49360 \\ & 97968\,37778\,89352\,93770\,96912\,94486\,41637\,87554\,51372\,03438 \\ & 21785\,50359\,64134\,04711\,0949 \end{aligned}$$

$$|\lambda_{11} - \hat{\lambda}_{11}| \leq 1.20 \times 10^{-171}.$$

$$\begin{aligned} \hat{\lambda}_{12} = & -0.00001\,30176\,97877\,02303\,05864\,01940\,63537\,68610\,78338\,51279 \\ & 22317\,86217\,67275\,58675\,87453\,43056\,48732\,32228\,66392\,65239 \\ & 97329\,56426\,18311\,54385\,55614\,07758\,38239\,47857\,48588\,65607 \\ & 63472\,97410\,25658\,75511\,5006 \end{aligned}$$

$$|\lambda_{12} - \hat{\lambda}_{12}| \leq 2.97 \times 10^{-171}.$$

$$\begin{aligned} \hat{\lambda}_{13} = & 0.00000\,49167\,82302\,46449\,12554\,61063\,80230\,80809\,03066\,92239 \\ & 45719\,11531\,85557\,42416\,31470\,38792\,23762\,08226\,60516\,67618 \\ & 80464\,66240\,50732\,15525\,90048\,97155\,67504\,39431\,07464\,29948 \\ & 26635\,54349\,83740\,66883\,0155 \end{aligned}$$

$$|\lambda_{13} - \hat{\lambda}_{13}| \leq 2.93 \times 10^{-171}.$$

$$\begin{aligned} \hat{\lambda}_{14} = & -0.00000\,18593\,07351\,50904\,23819\,86067\,49148\,55766\,74726\,32299 \\ & 23573\,04859\,75619\,41607\,74225\,24636\,77197\,31432\,72049\,13180 \\ & 20364\,14045\,24405\,63905\,79946\,88029\,15700\,94061\,33344\,00639 \\ & 89255\,36292\,69256\,57124\,2156 \end{aligned}$$

$$|\lambda_{14} - \hat{\lambda}_{14}| \leq 3.02 \times 10^{-171}.$$

$$\begin{aligned} \hat{\lambda}_{15} = & 0.00000\,07038\,11343\,08703\,98092\,46451\,58747\,28234\,80368\,16121 \\ & 84275\,68175\,19514\,95462\,50300\,55597\,63427\,62342\,64364\,02981 \\ & 46228\,62749\,60361\,58718\,80714\,72532\,43337\,15791\,63968\,26782 \\ & 56331\,31320\,82398\,97508\,7184 \end{aligned}$$

$$|\lambda_{15} - \hat{\lambda}_{15}| \leq 6.80 \times 10^{-171}.$$

$$\begin{aligned} \hat{\lambda}_{16} = & -0.00000\,02666\,41343\,44795\,64061\,71434\,24399\,65020\,90069\,70965 \\ & 19903\,84435\,70539\,68758\,02753\,28302\,46806\,73498\,65693\,68229 \\ & 28809\,70018\,57410\,33673\,31334\,12695\,64810\,97231\,65725\,89518 \\ & 75524\,70557\,646 \end{aligned}$$

$$|\lambda_{16} - \hat{\lambda}_{16}| \leq 1.71 \times 10^{-160}.$$

$$\begin{aligned} \hat{\lambda}_{17} = & 0.00000\,01010\,90553\,22149\,92469\,44625\,16592\,96810\,12050\,45533 \\ & 20755\,92349\,42207\,70771\,37268\,90091\,47364\,21391\,19922\,10577 \\ & 82774\,72183\,19919\,82298\,65233\,97929\,71572\,42038\,99241\,77745 \\ & 70194\,08245\,26 \end{aligned}$$

$$|\lambda_{17} - \hat{\lambda}_{17}| \leq 2.95 \times 10^{-159}.$$

$$\begin{aligned} \hat{\lambda}_{18} = & -0.00000\,00383\,49697\,95026\,56472\,70625\,94985\,61024\,36350\,86939 \\ & 20422\,19086\,95372\,32747\,30491\,77844\,25754\,53306\,96344\,18466 \\ & 35870\,50656\,71769\,50818\,10423\,99924\,87396\,73940\,07353\,49949 \\ & 86645\,83828\,5 \end{aligned}$$

$$|\lambda_{18} - \hat{\lambda}_{18}| \leq 5.11 \times 10^{-158}.$$

$$\begin{aligned} \hat{\lambda}_{19} = & 0.00000\,00145\,56138\,38668\,02305\,37072\,83970\,61356\,81493\,97573 \\ & 06186\,13537\,17964\,19623\,88955\,07208\,69473\,91235\,93245\,11002 \\ & 92086\,54811\,13185\,96257\,58594\,24301\,47652\,18894\,34247\,43944 \\ & 32528\,56414 \end{aligned}$$

$$|\lambda_{19} - \hat{\lambda}_{19}| \leq 8.83 \times 10^{-157}.$$

$$\begin{aligned} \hat{\lambda}_{20} = & -0.00000\,00055\,27567\,93799\,76080\,60488\,60801\,76572\,73702\,77389 \\ & 46171\,98874\,93165\,20263\,29087\,65460\,71376\,94876\,64184\,42155 \\ & 40262\,47735\,21069\,83440\,43869\,18179\,85435\,00006\,99878\,12456 \\ & 19045\,061 \end{aligned}$$

$$|\lambda_{20} - \hat{\lambda}_{20}| \leq 1.53 \times 10^{-155}.$$

$$\begin{aligned} \hat{\lambda}_{21} = & 0.00000000209991358297268764248798945279937160320784 \\ & 20225629540939121100908653459122006462599886689142 \\ & 60971000993888552605020319277495239007705862273359 \\ & 5254926 \end{aligned}$$

$$|\lambda_{21} - \hat{\lambda}_{21}| \leq 2.64 \times 10^{-154}.$$

$$\begin{aligned} \hat{\lambda}_{22} = & -0.00000000079804576827201962353935357260087901825327 \\ & 01174046868602968291574801686988593515388259329023 \\ & 11628306314951337916420043417650622116569246570872 \\ & 456792 \end{aligned}$$

$$|\lambda_{22} - \hat{\lambda}_{22}| \leq 4.57 \times 10^{-153}.$$

$$\begin{aligned} \hat{\lambda}_{23} = & 0.00000000030338629490985754219354145420248773687047 \\ & 07656689250061624575203663314318748469196372661660 \\ & 67664105075022929986142946244987068365726313802166 \\ & 68104 \end{aligned}$$

$$|\lambda_{23} - \hat{\lambda}_{23}| \leq 7.91 \times 10^{-152}.$$

$$\begin{aligned} \hat{\lambda}_{24} = & -0.00000000011536954181446685954677519722146716586194 \\ & 83705400330068375505966636251564052021327492432066 \\ & 57396998608657219820179597366471334575859552050934 \\ & 660 \end{aligned}$$

$$|\lambda_{24} - \hat{\lambda}_{24}| \leq 1.37 \times 10^{-150}.$$

$$\begin{aligned} \hat{\lambda}_{25} = & 0.00000000004388345011398436085206042678666550397893 \\ & 99870102747706566941806170983515775079007497903581 \\ & 50217381642739640908847827539464007103280564578477 \\ & 85 \end{aligned}$$

$$|\lambda_{25} - \hat{\lambda}_{25}| \leq 2.37 \times 10^{-149}.$$

$$\begin{aligned} \hat{\lambda}_{26} = & -0.00000000001669605215117376755281952859014377863436 \\ & 72130522510803043702080325630760043197532688281989 \\ & 84288776241384474156025285946654363325575742438194 \\ & 8 \end{aligned}$$

$$|\lambda_{26} - \hat{\lambda}_{26}| \leq 4.12 \times 10^{-148}.$$

$$\begin{aligned} \hat{\lambda}_{27} = & 0.00000000000635361242098269496304808082653766007307 \\ & 82529616587630463400769419983726272437490149587772 \\ & 55490640100399222808881604633783038207989186456382 \end{aligned}$$

$$|\lambda_{27} - \hat{\lambda}_{27}| \leq 7.20 \times 10^{-147}.$$

$$\begin{aligned} \hat{\lambda}_{28} = & -0.00000000000241831684759530204590226838906611048727 \\ & 34988721055132219360452614129282693371196889494500 \\ & 245886204055332975841915276659919686037071400504 \end{aligned}$$

$$|\lambda_{28} - \hat{\lambda}_{28}| \leq 1.28 \times 10^{-145}.$$

$$\begin{aligned} \hat{\lambda}_{29} = & 0.00000000000092062742005763398561192714565017245413 \\ & 01779802384789591274336074553633517321470837900953 \\ & 06931616697113898954929226299918771879953100847 \end{aligned}$$

$$|\lambda_{29} - \hat{\lambda}_{29}| \leq 2.37 \times 10^{-144}.$$

$$\begin{aligned} \hat{\lambda}_{30} = & -0.00000000000035053093545936863635537578208028732214 \\ & 69072180174123724528609105430959911617037879325867 \\ & 1236869670234771849410874429315237722469412747 \end{aligned}$$

$$|\lambda_{30} - \hat{\lambda}_{30}| \leq 4.98 \times 10^{-143}.$$

$$\begin{aligned} \hat{\lambda}_{31} = & 0.00000000000013348571441435690634868386438118599376 \\ & 48168539004568493686683981792543363498506810311243 \\ & 25138950216672349447615603868156219518969069 \end{aligned}$$

$$|\lambda_{31} - \hat{\lambda}_{31}| \leq 1.60 \times 10^{-141}.$$

$$\begin{aligned} \hat{\lambda}_{32} = & -0.00000000000005083983109740637151214897848777107852 \\ & 14205896407068171576571754113655981912444302093175 \\ & 2656166696739324314096515452727221827665 \end{aligned}$$

$$|\lambda_{32} - \hat{\lambda}_{32}| \leq 1.27 \times 10^{-137}.$$

$$\begin{aligned} \hat{\lambda}_{33} = & 0.00000000000001936554388308526740140270412156379527 \\ & 21988660348119832943314252006071540339587718062298 \\ & 4346423115012521280958974573612319531152479 \end{aligned}$$

$$|\lambda_{33} - \hat{\lambda}_{33}| \leq 1.25 \times 10^{-140}.$$

$$\begin{aligned} \hat{\lambda}_{34} = & -0.00000\,00000\,00007\,37747\,04644\,06519\,57074\,55159\,43241\,68679 \\ & 54772\,46843\,91168\,28992\,33533\,83899\,06088\,90936\,99060\,16239 \\ & 99417\,30208\,39739\,35594\,90300\,55585\,23721\,68201\,27 \end{aligned}$$

$$|\lambda_{34} - \hat{\lambda}_{34}| \leq 2.17 \times 10^{-139}.$$

$$\begin{aligned} \hat{\lambda}_{35} = & 0.00000\,00000\,00002\,81082\,45723\,26074\,06706\,68300\,89865\,16287 \\ & 86870\,67180\,18837\,22643\,64343\,20324\,36354\,52768\,10927\,97650 \\ & 94551\,61908\,52978\,72902\,05303\,96219\,54900\,03588\,2 \end{aligned}$$

$$|\lambda_{35} - \hat{\lambda}_{35}| \leq 3.75 \times 10^{-138}.$$

$$\begin{aligned} \hat{\lambda}_{36} = & -0.00000\,00000\,00001\,07103\,86501\,16071\,00414\,97633\,61770\,78216 \\ & 12807\,94556\,55501\,51969\,87878\,21886\,01916\,96150\,37692\,20969 \\ & 58640\,92516\,44233\,59127\,38940\,27032\,45536\,27426 \end{aligned}$$

$$|\lambda_{36} - \hat{\lambda}_{36}| \leq 6.49 \times 10^{-137}.$$

$$\begin{aligned} \hat{\lambda}_{37} = & 0.00000\,00000\,00000\,40814\,89263\,63649\,02966\,61004\,22050\,55381 \\ & 96587\,92825\,65666\,22615\,09857\,39984\,91082\,65255\,64096\,37780 \\ & 95878\,87809\,29855\,73079\,72987\,10706\,02639\,560 \end{aligned}$$

$$|\lambda_{37} - \hat{\lambda}_{37}| \leq 1.12 \times 10^{-135}.$$

$$\begin{aligned} \hat{\lambda}_{38} = & -0.00000\,00000\,00000\,15555\,05453\,23793\,10411\,05518\,34494\,23442 \\ & 35093\,77533\,75406\,22068\,70711\,84169\,46359\,60929\,66611\,59794 \\ & 98895\,03358\,64509\,60314\,17753\,00684\,90619\,03 \end{aligned}$$

$$|\lambda_{38} - \hat{\lambda}_{38}| \leq 1.95 \times 10^{-134}.$$

$$\begin{aligned} \hat{\lambda}_{39} = & 0.00000\,00000\,00000\,05928\,72462\,39469\,52612\,41063\,06396\,07007 \\ & 38665\,47218\,25869\,03804\,89329\,88236\,46537\,48947\,10200\,57837 \\ & 51834\,06871\,94806\,52976\,64016\,29729\,06676\,3 \end{aligned}$$

$$|\lambda_{39} - \hat{\lambda}_{39}| \leq 3.37 \times 10^{-133}.$$

$$\begin{aligned} \hat{\lambda}_{40} = & -0.00000\,00000\,00000\,02259\,88112\,97716\,18853\,47921\,00280\,21014 \\ & 88821\,57249\,84177\,54838\,75447\,45195\,73764\,88005\,64101\,76103 \\ & 25417\,00098\,88408\,14709\,38429\,15773\,12462 \end{aligned}$$

$$|\lambda_{40} - \hat{\lambda}_{40}| \leq 5.83 \times 10^{-132}.$$

$$\begin{aligned} \hat{\lambda}_{41} = & 0.0000000000000000000000861474442975977795666028896113483 \\ & 77979395397457470939971712708112145077799103686819 \\ & 731535148612838380085365007955598 \end{aligned}$$

$$|\lambda_{41} - \hat{\lambda}_{41}| \leq 1.01 \times 10^{-130}.$$

$$\begin{aligned} \hat{\lambda}_{42} = & -0.0000000000000000000000328420129321585877897586107292468 \\ & 00971151641599707181013398832236827530233922309159 \\ & 03339545214969923167972152660835 \end{aligned}$$

$$|\lambda_{42} - \hat{\lambda}_{42}| \leq 1.75 \times 10^{-129}.$$

$$\begin{aligned} \hat{\lambda}_{43} = & 0.0000000000000000000000125211997264208427204826448100541 \\ & 29806415795780230785197186679320894686690490969876 \\ & 4809635903749958999025626597601 \end{aligned}$$

$$|\lambda_{43} - \hat{\lambda}_{43}| \leq 3.03 \times 10^{-128}.$$

$$\begin{aligned} \hat{\lambda}_{44} = & -0.0000000000000000000000047740756993579664210694755595638 \\ & 21756408888267146060373676800771308519252099358278 \\ & 089352380302855982018822731096 \end{aligned}$$

$$|\lambda_{44} - \hat{\lambda}_{44}| \leq 5.24 \times 10^{-127}.$$

$$\begin{aligned} \hat{\lambda}_{45} = & 0.0000000000000000000000018203644456768280253736482973060 \\ & 34559245928823712059662125718028850346608565596909 \\ & 94366677494422114197612471676 \end{aligned}$$

$$|\lambda_{45} - \hat{\lambda}_{45}| \leq 9.07 \times 10^{-126}.$$

$$\begin{aligned} \hat{\lambda}_{46} = & -0.0000000000000000000000006941473812971440469492527446017 \\ & 56059774841724610623320919389595626509922228323583 \\ & 973749762451485044897639451 \end{aligned}$$

$$|\lambda_{46} - \hat{\lambda}_{46}| \leq 1.57 \times 10^{-124}.$$

$$\begin{aligned} \hat{\lambda}_{47} = & 0.0000000000000000000000002647086022847492490257442247002 \\ & 89651853864717540854140248086197572844679693581519 \\ & 32117944722602852507422524 \end{aligned}$$

$$|\lambda_{47} - \hat{\lambda}_{47}| \leq 2.72 \times 10^{-123}.$$

$$\begin{aligned}\hat{\lambda}_{48} = & -0.00000\,00000\,00000\,00001\,00949\,98340\,05395\,90567\,51533\,99168 \\ & 52679\,55619\,65231\,35003\,78746\,68010\,47645\,68214\,78473\,43166 \\ & 14456\,89882\,41406\,69648\,47009\end{aligned}$$

$$|\lambda_{48} - \hat{\lambda}_{48}| \leq 4.70 \times 10^{-122}.$$

$$\begin{aligned}\hat{\lambda}_{49} = & 0.00000\,00000\,00000\,00000\,38500\,39422\,49205\,11977\,39843\,44615 \\ & 51943\,75460\,62519\,74192\,73908\,33764\,80421\,07973\,93318\,22817 \\ & 15282\,90520\,75470\,65279\,7194\end{aligned}$$

$$|\lambda_{49} - \hat{\lambda}_{49}| \leq 8.13 \times 10^{-121}.$$

$$\begin{aligned}\hat{\lambda}_{50} = & -0.00000\,00000\,00000\,00000\,14683\,98058\,16557\,55858\,24316\,53623 \\ & 54677\,37312\,12115\,18606\,50471\,13246\,32124\,69237\,70691\,36956 \\ & 91737\,67646\,29538\,68141\,90\end{aligned}$$

$$|\lambda_{50} - \hat{\lambda}_{50}| \leq 1.41 \times 10^{-119}.$$

**Table S6: Certified spectral coefficients** ( $K = 1024$ ,  $P = 2048$ ). Each center  $\hat{\ell}_j(\mathbf{1})$  is displayed to full certified precision; the true coefficient satisfies  $|\ell_j(\mathbf{1}) - \hat{\ell}_j(\mathbf{1})| \leq \delta_{\ell,j}$ .

$\hat{\ell}_1(\mathbf{1}) = 0.83294037021578117245253644038968792199168460820204$   
74541 93931 62562 61984 78513 37166 84349 70973 22595 80071  
61918 72007 97131 31303 65391 83084 20150 89348 81061 30234  
64784 81541 05273 70875 43095 94816 06582 83234 84192 80548  
87181 74355 67519 83421 38580 24236 55153 38752 07332 37890  
84617 27195 91944 70727 88927 53818 18431 15174 99858 68254  
55515 87555 01531 2475

$$|\ell_1(\mathbf{1}) - \hat{\ell}_1(\mathbf{1})| \leq 4.52 \times 10^{-316}.$$

$\hat{\ell}_2(\mathbf{1}) = 0.45120576837332503477832474729206957160007477982538$   
78350 35516 19351 99477 99471 96868 59676 03798 34282 07351  
56774 24809 56406 69904 16290 68908 46780 64515 14968 82598  
84084 57869 58941 43115 26937 25112 32009 77529 23629 03468  
16205 02460 63979 69471 90978 66982 59267 55465 27779 39743  
56090 11484 49803 36268 04081 31047 84642 47308 28083 75713  
71998 42317 13823 580

$$|\ell_2(\mathbf{1}) - \hat{\ell}_2(\mathbf{1})| \leq 4.13 \times 10^{-315}.$$

$\hat{\ell}_3(\mathbf{1}) = -0.20193987421291717050277392531196327489140794213779$   
11057 75329 35266 07379 29708 17604 03987 30047 91797 93405  
92874 08737 77205 84080 78212 75458 02895 01194 06492 86684  
83616 06290 68971 77639 93175 61680 52114 14197 07945 15507  
61092 05065 84230 89376 12890 91658 81824 44860 42650 33985  
28206 48413 61638 78649 53447 15196 08623 07128 14007 14703  
22396 85621 48717 99

$$|\ell_3(\mathbf{1}) - \hat{\ell}_3(\mathbf{1})| \leq 2.96 \times 10^{-314}.$$

$\hat{\ell}_4(\mathbf{1}) = 0.08740239297620928797827366502808883409663074863687$   
99598 73640 34659 61891 06221 84673 29058 35503 84649 70471  
39309 91420 90722 76494 95880 50178 95722 86838 21977 96365  
55570 53491 76663 33941 20702 75480 75425 13419 05099 51844  
78360 38503 53317 10594 91655 04896 89769 41874 98225 98263  
72111 22028 20706 63333 52855 64327 49667 99619 75197 30143  
82708 93119 49341 2

$$|\ell_4(\mathbf{1}) - \hat{\ell}_4(\mathbf{1})| \leq 1.73 \times 10^{-313}.$$

$$\begin{aligned} \hat{\ell}_5(\mathbf{1}) = & -0.03694\,61611\,13582\,88926\,98152\,60092\,58180\,67466\,59884\,11878 \\ & 69597\,36290\,90224\,34070\,57210\,59890\,84868\,43641\,58374\,73410 \\ & 29261\,95699\,17557\,12296\,63259\,38179\,64004\,85030\,37397\,82506 \\ & 94570\,14372\,40665\,37439\,20833\,71370\,28291\,10180\,82462\,63266 \\ & 13307\,02898\,48369\,91783\,28530\,51764\,23344\,32767\,22416\,83256 \\ & 89724\,83469\,26331\,78781\,28063\,54620\,97860\,75745\,21932\,35917 \\ & 87334\,90183\,45996\,4 \end{aligned}$$

$$|\ell_5(\mathbf{1}) - \hat{\ell}_5(\mathbf{1})| \leq 8.94 \times 10^{-313}.$$

$$\begin{aligned} \hat{\ell}_6(\mathbf{1}) = & 0.01534\,79541\,61442\,57494\,96909\,43147\,07109\,14752\,59344\,45074 \\ & 33454\,22732\,89763\,74327\,95013\,20533\,16167\,79079\,40914\,90042 \\ & 37563\,40344\,58025\,57384\,24160\,99106\,11085\,04811\,29614\,27291 \\ & 28377\,14042\,17980\,22539\,06595\,23000\,88792\,55709\,46527\,29885 \\ & 22797\,87954\,90632\,13146\,19232\,52859\,13548\,43911\,50483\,29381 \\ & 34974\,72283\,85292\,66808\,87543\,79078\,05327\,71978\,89593\,49860 \\ & 04423\,74962\,33587 \end{aligned}$$

$$|\ell_6(\mathbf{1}) - \hat{\ell}_6(\mathbf{1})| \leq 4.31 \times 10^{-312}.$$

$$\begin{aligned} \hat{\ell}_7(\mathbf{1}) = & -0.00629\,49804\,19957\,31671\,82960\,99980\,08909\,06108\,36683\,41115 \\ & 55617\,41362\,75469\,42895\,05413\,82309\,40929\,16919\,25288\,43260 \\ & 80183\,89588\,97567\,09039\,84562\,31907\,51698\,46665\,54971\,76793 \\ & 43654\,08426\,15628\,14890\,50389\,66141\,34900\,92973\,37738\,70449 \\ & 15070\,05568\,30464\,61605\,36500\,68656\,94841\,46002\,26869\,61077 \\ & 47995\,87996\,23769\,38855\,99209\,53236\,45964\,34237\,09588\,94754 \\ & 63668\,97159\,3451 \end{aligned}$$

$$|\ell_7(\mathbf{1}) - \hat{\ell}_7(\mathbf{1})| \leq 2.01 \times 10^{-311}.$$

$$\begin{aligned} \hat{\ell}_8(\mathbf{1}) = & 0.00255\,74209\,14786\,48398\,64670\,44264\,86309\,04172\,52649\,20017 \\ & 08977\,08127\,87164\,04727\,81772\,18238\,95146\,89301\,26690\,94987 \\ & 84097\,48059\,30601\,57126\,09848\,11118\,64282\,14395\,36621\,80817 \\ & 06410\,53269\,59303\,01641\,02765\,05894\,20759\,30648\,29036\,33671 \\ & 80140\,38752\,92654\,73403\,88395\,77527\,50883\,16349\,27832\,87448 \\ & 58386\,78565\,39951\,05220\,86646\,93428\,61262\,66208\,49040\,60506 \\ & 64343\,10350\,4177 \end{aligned}$$

$$|\ell_8(\mathbf{1}) - \hat{\ell}_8(\mathbf{1})| \leq 9.18 \times 10^{-311}.$$

$$\begin{aligned} \hat{\ell}_9(\mathbf{1}) = & -0.00103\,14151\,91716\,37114\,14075\,91726\,11619\,67246\,00875\,57210 \\ & 36342\,92699\,05974\,34669\,05705\,66891\,36884\,21552\,29007\,20546 \\ & 19519\,26239\,47871\,44470\,71624\,26970\,12390\,37159\,98556\,85977 \\ & 18802\,38262\,13389\,60113\,46195\,20555\,51865\,11804\,59430\,36093 \\ & 49412\,20763\,16476\,89584\,77418\,33983\,04049\,31586\,15204\,73540 \\ & 44759\,21452\,68135\,15803\,95435\,36023\,00531\,45673\,13368\,70426 \\ & 94054\,72477\,871 \end{aligned}$$

$$|\ell_9(\mathbf{1}) - \hat{\ell}_9(\mathbf{1})| \leq 4.17 \times 10^{-310}.$$

$$\begin{aligned} \hat{\ell}_{10}(\mathbf{1}) = & 0.00041\,35795\,74474\,74152\,63779\,55854\,92949\,25024\,78480\,25928 \\ & 00126\,09564\,36756\,54902\,61983\,31121\,37756\,60779\,81488\,56700 \\ & 02432\,04759\,00483\,72463\,27639\,76300\,72178\,01885\,39817\,01385 \\ & 60354\,35640\,59017\,63754\,80014\,45781\,53546\,80332\,53028\,06241 \\ & 84619\,95629\,27999\,04777\,10226\,17647\,35560\,40242\,34282\,36980 \\ & 00013\,56001\,09557\,96476\,29092\,80823\,69941\,31401\,42781\,14159 \\ & 77070\,30315\,83 \end{aligned}$$

$$|\ell_{10}(\mathbf{1}) - \hat{\ell}_{10}(\mathbf{1})| \leq 1.89 \times 10^{-309}.$$

$$\begin{aligned} \hat{\ell}_{11}(\mathbf{1}) = & -0.00016\,50673\,61989\,44019\,51968\,26101\,84039\,62040\,39282\,04133 \\ & 83544\,90088\,18782\,69472\,78809\,92899\,26468\,84875\,54962\,87022 \\ & 98643\,75702\,33757\,69898\,92712\,57715\,68891\,69506\,04916\,84421 \\ & 78460\,08219\,79864\,28109\,40010\,43881\,21517\,51069\,19771\,25176 \\ & 63112\,55403\,36647\,42853\,71342\,16760\,41693\,65927\,47938\,05279 \\ & 95546\,14155\,76694\,32321\,95158\,69072\,19890\,91664\,35361\,88080 \\ & 57022\,20681\,79 \end{aligned}$$

$$|\ell_{11}(\mathbf{1}) - \hat{\ell}_{11}(\mathbf{1})| \leq 8.57 \times 10^{-309}.$$

$$\begin{aligned} \hat{\ell}_{12}(\mathbf{1}) = & 0.00006\,56291\,17563\,91487\,10872\,66400\,80300\,47617\,36245\,62781 \\ & 67575\,09425\,41998\,93610\,25642\,66108\,87464\,02904\,95402\,78877 \\ & 05153\,13696\,44079\,97309\,45155\,22530\,08717\,18847\,55020\,59196 \\ & 66158\,34431\,17687\,93355\,29523\,50637\,55276\,80866\,32286\,60372 \\ & 47423\,12404\,03839\,65564\,91610\,46446\,21218\,55580\,27985\,01328 \\ & 56116\,75605\,87351\,54820\,16063\,01136\,09686\,91913\,01656\,99204 \\ & 06716\,45675\,1 \end{aligned}$$

$$|\ell_{12}(\mathbf{1}) - \hat{\ell}_{12}(\mathbf{1})| \leq 3.90 \times 10^{-308}.$$

$$\begin{aligned} \hat{\ell}_{13}(\mathbf{1}) = & -0.00002\,60097\,16743\,28916\,78271\,24486\,10361\,54235\,21866\,99000 \\ & 70242\,50432\,41055\,67905\,13561\,49777\,59204\,79802\,27434\,49512 \\ & 19283\,12534\,78740\,04506\,51277\,98136\,97883\,64777\,33877\,76784 \\ & 54756\,40631\,17641\,27994\,39356\,00369\,39299\,63597\,16096\,00508 \\ & 83859\,59706\,65144\,85272\,29971\,80057\,17773\,44872\,84923\,29229 \\ & 65278\,53252\,05566\,52113\,66958\,87515\,63260\,74200\,30320\,01286 \\ & 45803\,76902 \end{aligned}$$

$$|\ell_{13}(\mathbf{1}) - \hat{\ell}_{13}(\mathbf{1})| \leq 1.78 \times 10^{-307}.$$

$$\begin{aligned} \hat{\ell}_{14}(\mathbf{1}) = & 0.00001\,02798\,81380\,84834\,56276\,88157\,45542\,43642\,43642\,16457 \\ & 69536\,01350\,07102\,24886\,17063\,90096\,01096\,41940\,19287\,38537 \\ & 20551\,72917\,80040\,90688\,35920\,47086\,86678\,79057\,92883\,71962 \\ & 19244\,04069\,30506\,61033\,22259\,57050\,69915\,32132\,02292\,48694 \\ & 55397\,01768\,56960\,54834\,18361\,87155\,87931\,07158\,29541\,57682 \\ & 33104\,05673\,31443\,47469\,54544\,83722\,15451\,39904\,55441\,10094 \\ & 35405\,59869 \end{aligned}$$

$$|\ell_{14}(\mathbf{1}) - \hat{\ell}_{14}(\mathbf{1})| \leq 8.16 \times 10^{-307}.$$

$$\begin{aligned} \hat{\ell}_{15}(\mathbf{1}) = & -0.00000\,40534\,02970\,27246\,15707\,46878\,86695\,82816\,59390\,60425 \\ & 55602\,95235\,10281\,29619\,82446\,85702\,36110\,43665\,89944\,20338 \\ & 20424\,15977\,78358\,86772\,96396\,69912\,26478\,27385\,63207\,89511 \\ & 36548\,14731\,43403\,19127\,08985\,85365\,73014\,39760\,97847\,33632 \\ & 35164\,48576\,90102\,51450\,22785\,88999\,83472\,68871\,80855\,51758 \\ & 78729\,81469\,79990\,78815\,05710\,86916\,08181\,20887\,77640\,80419 \\ & 58760\,1175 \end{aligned}$$

$$|\ell_{15}(\mathbf{1}) - \hat{\ell}_{15}(\mathbf{1})| \leq 3.75 \times 10^{-306}.$$

$$\begin{aligned} \hat{\ell}_{16}(\mathbf{1}) = & 0.00000\,15950\,11839\,90722\,49316\,92042\,21259\,13862\,20640\,27661 \\ & 62763\,23754\,31523\,00783\,30474\,94423\,72082\,86004\,08999\,98546 \\ & 62019\,23233\,96505\,70682\,14932\,01566\,69950\,41223\,78997\,95014 \\ & 18247\,64918\,26567\,33438\,77463\,67311\,56325\,79243\,97654\,15112 \\ & 75071\,91041\,43712\,11844\,93852\,99445\,76170\,26498\,10110\,91090 \\ & 11559\,31998\,44212\,03423\,76350\,68363\,49097\,15702\,25900\,36584 \\ & 68373\,106 \end{aligned}$$

$$|\ell_{16}(\mathbf{1}) - \hat{\ell}_{16}(\mathbf{1})| \leq 1.73 \times 10^{-305}.$$

$$\begin{aligned} \hat{\ell}_{17}(\mathbf{1}) = & -0.0000006265\ 11706\ 51509\ 46989\ 98059\ 35783\ 02802\ 86726\ 32041 \\ & 08945\ 87834\ 63161\ 03741\ 46023\ 91639\ 27379\ 27212\ 28264\ 37679 \\ & 87900\ 08058\ 26963\ 42407\ 53638\ 58173\ 25934\ 04021\ 10056\ 19635 \\ & 43916\ 11413\ 00763\ 76002\ 08428\ 19772\ 27569\ 86703\ 15729\ 15071 \\ & 08956\ 30702\ 44773\ 52630\ 41879\ 46981\ 01889\ 52845\ 19568\ 11269 \\ & 90364\ 73014\ 00075\ 33021\ 94447\ 01314\ 89657\ 92785\ 33422\ 00058 \\ & 36586\ 364 \end{aligned}$$

$$|\ell_{17}(\mathbf{1}) - \hat{\ell}_{17}(\mathbf{1})| \leq 7.98 \times 10^{-305}.$$

$$\begin{aligned} \hat{\ell}_{18}(\mathbf{1}) = & 0.0000002457\ 00158\ 16934\ 65096\ 92170\ 11693\ 21324\ 34089\ 02206 \\ & 96257\ 71210\ 36839\ 82660\ 36690\ 03835\ 99504\ 73456\ 57346\ 76275 \\ & 41758\ 29422\ 99112\ 78186\ 80763\ 28918\ 53617\ 14130\ 74627\ 33355 \\ & 55597\ 96792\ 68120\ 65057\ 81048\ 10531\ 78555\ 88079\ 81913\ 95841 \\ & 54423\ 47796\ 63234\ 76319\ 15942\ 55742\ 96207\ 33668\ 49611\ 53695 \\ & 21683\ 25416\ 53781\ 10895\ 46440\ 32743\ 13861\ 07477\ 82373\ 83601 \\ & 72512\ 82 \end{aligned}$$

$$|\ell_{18}(\mathbf{1}) - \hat{\ell}_{18}(\mathbf{1})| \leq 3.69 \times 10^{-304}.$$

$$\begin{aligned} \hat{\ell}_{19}(\mathbf{1}) = & -0.0000000962\ 20523\ 87808\ 12125\ 95527\ 00093\ 49043\ 53169\ 57818 \\ & 31496\ 78786\ 96957\ 58115\ 52913\ 09784\ 72500\ 90742\ 59081\ 47954 \\ & 46455\ 35617\ 27086\ 88164\ 74444\ 77948\ 55686\ 50802\ 74165\ 09046 \\ & 41760\ 74836\ 49340\ 91909\ 58127\ 57614\ 17739\ 41427\ 13910\ 37221 \\ & 76327\ 63617\ 91280\ 01317\ 15475\ 17820\ 74113\ 23506\ 59174\ 29018 \\ & 32146\ 42532\ 78097\ 66546\ 32918\ 42700\ 88331\ 81293\ 78542\ 41687 \\ & 40653\ 4 \end{aligned}$$

$$|\ell_{19}(\mathbf{1}) - \hat{\ell}_{19}(\mathbf{1})| \leq 1.71 \times 10^{-303}.$$

$$\begin{aligned} \hat{\ell}_{20}(\mathbf{1}) = & 0.0000000376\ 33916\ 39516\ 77577\ 80963\ 57080\ 51115\ 43030\ 33910 \\ & 78228\ 27230\ 22230\ 63956\ 67012\ 07737\ 45152\ 50225\ 38170\ 71439 \\ & 35526\ 76149\ 65562\ 28439\ 01374\ 98502\ 94132\ 97833\ 83286\ 34057 \\ & 49207\ 94205\ 97487\ 67167\ 78108\ 12003\ 94775\ 13696\ 56830\ 30508 \\ & 51473\ 54230\ 82586\ 19946\ 26705\ 66260\ 89627\ 98010\ 84739\ 82153 \\ & 02503\ 28748\ 32348\ 03058\ 38112\ 27275\ 74025\ 44054\ 05920\ 36489 \\ & 31402\ 4 \end{aligned}$$

$$|\ell_{20}(\mathbf{1}) - \hat{\ell}_{20}(\mathbf{1})| \leq 7.96 \times 10^{-303}.$$

$$\begin{aligned} \hat{\ell}_{21}(\mathbf{1}) = & -0.00000001470261334082057591634867943344852616297093 \\ & 38714909021866105146107021864974703248955346500419 \\ & 04740391876982326308893752590300457011493066968132 \\ & 39461640052112827061342135469077920096524871980677 \\ & 50201777257973234520018296015423920413984651738788 \\ & 91817131515121767070768344858098567798076338265443 \\ & 98672 \end{aligned}$$

$$|\ell_{21}(\mathbf{1}) - \hat{\ell}_{21}(\mathbf{1})| \leq 3.70 \times 10^{-302}.$$

$$\begin{aligned} \hat{\ell}_{22}(\mathbf{1}) = & 0.00000000573798579791060191841412698666384592903091 \\ & 07815521190662314336669052726713543104105945683097 \\ & 35254828935358597855683528203927713432638515155163 \\ & 09684467983680564023059184949047880306466158946264 \\ & 49216212878024597841635543387882575839898221259355 \\ & 33541339520953993093258511410211980441273009118146 \\ & 4949 \end{aligned}$$

$$|\ell_{22}(\mathbf{1}) - \hat{\ell}_{22}(\mathbf{1})| \leq 1.72 \times 10^{-301}.$$

$$\begin{aligned} \hat{\ell}_{23}(\mathbf{1}) = & -0.00000000223724920262289175521208518308520381057879 \\ & 34229622785990481523873276477079489505145224209777 \\ & 08880327872672840043995224569014679106384576967190 \\ & 86256637228283775847369761456845364146059462937233 \\ & 53914582031521585550057350156255057991628829444169 \\ & 67389280415010161701158726043623620955004688291992 \\ & 6745 \end{aligned}$$

$$|\ell_{23}(\mathbf{1}) - \hat{\ell}_{23}(\mathbf{1})| \leq 8.04 \times 10^{-301}.$$

$$\begin{aligned} \hat{\ell}_{24}(\mathbf{1}) = & 0.00000000087155378401660754502612188881341366842522 \\ & 29526655487100090794271995308317250847795072587972 \\ & 59470595126224795011469441827747253553790192032826 \\ & 60292152005917904524076601593165141029987018781674 \\ & 22024928250464518646275823285074173921593947703149 \\ & 06770403828526153668388549148391434965311006558254 \\ & 106 \end{aligned}$$

$$|\ell_{24}(\mathbf{1}) - \hat{\ell}_{24}(\mathbf{1})| \leq 3.75 \times 10^{-300}.$$

$$\begin{aligned} \hat{\ell}_{25}(\mathbf{1}) = & -0.00000000033925762914088370581811290854174761204253 \\ & 83699731959477880465019676477423794816538691298289 \\ & 04056837008166346078772920461458925586183054093591 \\ & 85183076564148552842882684675413150830223596382542 \\ & 45706068899172717882659456879278114312503414173113 \\ & 72665958525446347834739295517304078797540481631881 \\ & 10 \end{aligned}$$

$$|\ell_{25}(\mathbf{1}) - \hat{\ell}_{25}(\mathbf{1})| \leq 1.75 \times 10^{-299}.$$

$$\begin{aligned} \hat{\ell}_{26}(\mathbf{1}) = & 0.00000000013196163272027403585508760459090333353026 \\ & 22462262641538693186720571925023917216076342110537 \\ & 62203762752731710241721451192758335877495061986408 \\ & 81827380554155895860666353713345215185296963538275 \\ & 47819725217768976004269054260176857127441380827063 \\ & 05250348006946525509460785145480821721809696911626 \\ & 50 \end{aligned}$$

$$|\ell_{26}(\mathbf{1}) - \hat{\ell}_{26}(\mathbf{1})| \leq 8.21 \times 10^{-299}.$$

$$\begin{aligned} \hat{\ell}_{27}(\mathbf{1}) = & -0.00000000005129467879750722501701897535701730560240 \\ & 41379727916754137679790571440748887610199350483207 \\ & 21492793069092967738016947738211055465786076208921 \\ & 80905416189045540348081380022532692984361800049183 \\ & 28005819037473420181629377713952892815450491949571 \\ & 57571254517990312666444050800710344094610913576191 \\ & 0 \end{aligned}$$

$$|\ell_{27}(\mathbf{1}) - \hat{\ell}_{27}(\mathbf{1})| \leq 3.84 \times 10^{-298}.$$

$$\begin{aligned} \hat{\ell}_{28}(\mathbf{1}) = & 0.00000000001992621663281064431258836560396083525289 \\ & 30364721209460017685969333720963854814593274974157 \\ & 29017172858294595270547956431515815430094919043257 \\ & 63281224385769145198248534983054083918138563912166 \\ & 47445505846589148917531582030136841662551104828416 \\ & 78508943252789575957735230296761645507160530070606 \end{aligned}$$

$$|\ell_{28}(\mathbf{1}) - \hat{\ell}_{28}(\mathbf{1})| \leq 1.80 \times 10^{-297}.$$

$$\begin{aligned}\hat{\ell}_{29}(\mathbf{1}) = & -0.00000\,00000\,07736\,14043\,76857\,30102\,32114\,02696\,27414\,94474 \\ & 55355\,85935\,16285\,11674\,37634\,78492\,92381\,29112\,79332\,46258 \\ & 58548\,43733\,87391\,21489\,26052\,42186\,03883\,68103\,73101\,17716 \\ & 70541\,87590\,62072\,52043\,79612\,44846\,46336\,32404\,47662\,47813 \\ & 30285\,95480\,46893\,42363\,74282\,27692\,16087\,97298\,02142\,41055 \\ & 97355\,78429\,28061\,80967\,86161\,80145\,85711\,25901\,26447\,70310\end{aligned}$$

$$|\ell_{29}(\mathbf{1}) - \hat{\ell}_{29}(\mathbf{1})| \leq 8.43 \times 10^{-297}.$$

$$\begin{aligned}\hat{\ell}_{30}(\mathbf{1}) = & 0.00000\,00000\,03001\,84266\,52059\,16623\,25572\,51521\,10866\,48401 \\ & 59741\,75836\,54666\,54359\,75767\,84108\,10130\,86886\,13299\,17118 \\ & 01558\,20970\,58775\,96266\,79981\,42659\,43476\,10875\,91964\,31049 \\ & 37260\,74823\,74454\,96109\,75915\,46884\,66253\,16361\,38177\,91014 \\ & 54070\,43100\,60210\,35782\,98381\,50027\,49753\,48852\,92831\,59356 \\ & 63767\,96311\,12389\,56563\,12766\,71791\,02554\,46968\,11447\,9070\end{aligned}$$

$$|\ell_{30}(\mathbf{1}) - \hat{\ell}_{30}(\mathbf{1})| \leq 3.96 \times 10^{-296}.$$

$$\begin{aligned}\hat{\ell}_{31}(\mathbf{1}) = & -0.00000\,00000\,01164\,20917\,75750\,74682\,88056\,16638\,11475\,19435 \\ & 99612\,53689\,36247\,99422\,06546\,57671\,48553\,60451\,14701\,47910 \\ & 88320\,97254\,39455\,94413\,12450\,84566\,33523\,17971\,94513\,64842 \\ & 52813\,02090\,01195\,79521\,46722\,18059\,85759\,21091\,91948\,52290 \\ & 98792\,45737\,87234\,74415\,04256\,61646\,12249\,61045\,77664\,89163 \\ & 61781\,40843\,88435\,79349\,29740\,52766\,35273\,74558\,41238\,107\end{aligned}$$

$$|\ell_{31}(\mathbf{1}) - \hat{\ell}_{31}(\mathbf{1})| \leq 1.86 \times 10^{-295}.$$

$$\begin{aligned}\hat{\ell}_{32}(\mathbf{1}) = & 0.00000\,00000\,00451\,30233\,15697\,64116\,52945\,00735\,95807\,79794 \\ & 07569\,65545\,19098\,53197\,76485\,52221\,19408\,56610\,05898\,06370 \\ & 45237\,81925\,10071\,35198\,03780\,65740\,95023\,72598\,98657\,11950 \\ & 33509\,74764\,25514\,29213\,64175\,36412\,65720\,56345\,87858\,38339 \\ & 71678\,22976\,86936\,40505\,27380\,02762\,12266\,22026\,68171\,76996 \\ & 60942\,16412\,68312\,15506\,71160\,89711\,72493\,72577\,07870\,905\end{aligned}$$

$$|\ell_{32}(\mathbf{1}) - \hat{\ell}_{32}(\mathbf{1})| \leq 8.72 \times 10^{-295}.$$

$$\begin{aligned}\hat{\ell}_{33}(\mathbf{1}) = & -0.00000\,00000\,00174\,86796\,84921\,16744\,62212\,22651\,49431\,63725 \\ & 19126\,61850\,91192\,67448\,76079\,82135\,61220\,46441\,37137\,01484 \\ & 46103\,18894\,51272\,82759\,53936\,66076\,82563\,20710\,00124\,63852 \\ & 06481\,50327\,55507\,21056\,36213\,66978\,06951\,48040\,29575\,04861 \\ & 99653\,34333\,56020\,61627\,47373\,41742\,39521\,73767\,59306\,56910 \\ & 25141\,70628\,14925\,06899\,35905\,46064\,26031\,29235\,15937\,44\end{aligned}$$

$$|\ell_{33}(\mathbf{1}) - \hat{\ell}_{33}(\mathbf{1})| \leq 4.10 \times 10^{-294}.$$

$$\begin{aligned}\hat{\ell}_{34}(\mathbf{1}) = & 0.00000\,00000\,00067\,72836\,74309\,03661\,87786\,94167\,25441\,83325 \\ & 81297\,55485\,61666\,16972\,27965\,75105\,31293\,17606\,15730\,48660 \\ & 65859\,61956\,58019\,54574\,94180\,73105\,27312\,07460\,50337\,05024 \\ & 41644\,20854\,17164\,62398\,52008\,96038\,26452\,86070\,94675\,07901 \\ & 73882\,26074\,55842\,35632\,97958\,68283\,34565\,61068\,18329\,19223 \\ & 70000\,94189\,31098\,09818\,47313\,72650\,15347\,59939\,68161\,5\end{aligned}$$

$$|\ell_{34}(\mathbf{1}) - \hat{\ell}_{34}(\mathbf{1})| \leq 1.92 \times 10^{-293}.$$

$$\begin{aligned}\hat{\ell}_{35}(\mathbf{1}) = & -0.00000\,00000\,00026\,22159\,63077\,33029\,60968\,91584\,37676\,84519 \\ & 78240\,29160\,86764\,91438\,12132\,41186\,61351\,33059\,74146\,65208 \\ & 11266\,70026\,08717\,05315\,01361\,05161\,51832\,88164\,94938\,92948 \\ & 87565\,66369\,66983\,64219\,51379\,24496\,69786\,57815\,81999\,10478 \\ & 90234\,03764\,07337\,80642\,40131\,73177\,82104\,54333\,84099\,61011 \\ & 76809\,64128\,73933\,80883\,93217\,77189\,89621\,82220\,36980\,5\end{aligned}$$

$$|\ell_{35}(\mathbf{1}) - \hat{\ell}_{35}(\mathbf{1})| \leq 9.05 \times 10^{-293}.$$

$$\begin{aligned}\hat{\ell}_{36}(\mathbf{1}) = & 0.00000\,00000\,00010\,14811\,67697\,67601\,96665\,02498\,51231\,44686 \\ & 37686\,03045\,43721\,74227\,71703\,85117\,81952\,73323\,49170\,01217 \\ & 00843\,28658\,81118\,08680\,68844\,06406\,83895\,97161\,62184\,06696 \\ & 93600\,03712\,38819\,37483\,38559\,61616\,08555\,04941\,93477\,24767 \\ & 96869\,70162\,14106\,13150\,47743\,20297\,54405\,01033\,69847\,55491 \\ & 31579\,94450\,84373\,10266\,13306\,18789\,87771\,61594\,35945\end{aligned}$$

$$|\ell_{36}(\mathbf{1}) - \hat{\ell}_{36}(\mathbf{1})| \leq 4.26 \times 10^{-292}.$$

$$\begin{aligned}\hat{\ell}_{37}(\mathbf{1}) = & -0.0000000000000003\,92607\,35676\,82377\,04191\,19107\,08409\,25260 \\ & 85733\,00155\,88730\,68344\,87181\,08480\,99070\,43606\,42315\,81631 \\ & 12317\,22514\,13591\,57530\,89024\,06997\,03701\,22546\,04697\,85751 \\ & 85621\,90596\,71766\,90480\,46930\,14837\,86932\,15781\,34126\,45650 \\ & 59315\,02798\,88558\,92193\,22903\,15678\,12965\,85719\,55031\,05841 \\ & 79025\,93973\,25198\,19880\,59380\,37150\,07244\,76465\,3502\end{aligned}$$

$$|\ell_{37}(\mathbf{1}) - \hat{\ell}_{37}(\mathbf{1})| \leq 2.00 \times 10^{-291}.$$

$$\begin{aligned}\hat{\ell}_{38}(\mathbf{1}) = & 0.0000000000000001\,51839\,99867\,84238\,08691\,06819\,71457\,36392 \\ & 05888\,10708\,84009\,39310\,75056\,29225\,05785\,06946\,93421\,29135 \\ & 20815\,80228\,94951\,99221\,30813\,97203\,21494\,98416\,50590\,19808 \\ & 32384\,98422\,10403\,50127\,67771\,66841\,81921\,06218\,05000\,33122 \\ & 50575\,53845\,55861\,60347\,11617\,11479\,34804\,35704\,11130\,87741 \\ & 53218\,99340\,03103\,98131\,04033\,03643\,20861\,96639\,1524\end{aligned}$$

$$|\ell_{38}(\mathbf{1}) - \hat{\ell}_{38}(\mathbf{1})| \leq 9.43 \times 10^{-291}.$$

$$\begin{aligned}\hat{\ell}_{39}(\mathbf{1}) = & -0.0000000000000000\,58705\,15353\,82839\,51692\,86220\,59817\,93075 \\ & 37006\,42460\,82956\,65334\,84519\,20957\,10347\,13486\,87092\,59380 \\ & 53502\,47756\,83886\,62483\,33545\,10546\,31893\,89555\,22964\,70247 \\ & 98320\,23018\,27368\,84899\,57310\,30076\,31527\,31398\,28846\,87554 \\ & 44468\,06702\,25973\,10668\,13164\,59343\,24423\,03640\,44446\,84401 \\ & 01170\,34979\,23069\,03626\,50608\,29338\,89775\,27368\,628\end{aligned}$$

$$|\ell_{39}(\mathbf{1}) - \hat{\ell}_{39}(\mathbf{1})| \leq 4.44 \times 10^{-290}.$$

$$\begin{aligned}\hat{\ell}_{40}(\mathbf{1}) = & 0.0000000000000000\,22690\,05105\,20209\,61706\,24303\,00987\,26909 \\ & 78474\,66307\,97029\,90566\,26758\,57594\,64723\,26657\,61628\,04607 \\ & 36028\,93224\,65294\,99373\,52059\,78694\,61860\,30485\,34504\,34103 \\ & 45858\,17222\,15311\,13169\,54710\,84710\,62013\,48851\,34064\,40370 \\ & 20259\,62442\,20699\,46412\,83288\,28407\,33339\,63907\,64558\,01760 \\ & 06443\,32557\,41689\,92315\,86642\,70984\,15015\,69200\,36\end{aligned}$$

$$|\ell_{40}(\mathbf{1}) - \hat{\ell}_{40}(\mathbf{1})| \leq 2.09 \times 10^{-289}.$$

$$\begin{aligned}\hat{\ell}_{41}(\mathbf{1}) = & -0.00000\,00000\,00000\,08767\,39032\,21082\,48894\,38664\,45857\,63246 \\ & 01193\,85553\,27143\,45861\,58827\,16015\,30255\,17068\,46881\,61074 \\ & 06151\,57097\,71761\,49417\,36614\,37003\,65265\,37560\,30608\,04435 \\ & 82515\,19860\,90280\,13783\,34572\,31511\,05266\,16843\,99524\,20869 \\ & 26190\,37925\,46729\,29547\,51871\,73123\,48919\,59511\,83738\,44133 \\ & 83195\,11207\,83878\,73064\,45966\,04879\,87399\,54566\,20\end{aligned}$$

$$|\ell_{41}(\mathbf{1}) - \hat{\ell}_{41}(\mathbf{1})| \leq 9.86 \times 10^{-289}.$$

$$\begin{aligned}\hat{\ell}_{42}(\mathbf{1}) = & 0.00000\,00000\,00000\,03386\,77844\,27817\,27577\,38966\,53650\,25569 \\ & 02370\,12834\,24159\,74015\,31087\,02827\,71707\,10703\,07606\,54027 \\ & 00827\,97129\,98924\,02588\,55347\,93369\,20971\,35935\,50433\,00060 \\ & 69819\,12213\,89714\,73264\,14095\,06585\,72555\,20139\,05359\,79588 \\ & 54691\,02030\,16865\,33309\,59158\,18326\,97937\,69688\,40756\,63978 \\ & 56447\,40083\,80163\,97014\,47868\,50131\,23049\,48592\,1\end{aligned}$$

$$|\ell_{42}(\mathbf{1}) - \hat{\ell}_{42}(\mathbf{1})| \leq 4.65 \times 10^{-288}.$$

$$\begin{aligned}\hat{\ell}_{43}(\mathbf{1}) = & -0.00000\,00000\,00000\,01307\,94758\,80025\,34886\,18765\,86978\,04696 \\ & 90870\,49657\,12296\,23704\,48498\,90195\,70426\,78586\,56741\,93654 \\ & 60440\,75318\,52520\,14528\,44872\,04096\,13649\,39465\,14003\,88861 \\ & 53675\,22832\,73697\,62602\,19578\,32966\,85911\,55088\,19861\,10148 \\ & 31387\,28666\,69766\,12176\,17741\,84513\,52985\,43523\,04643\,43448 \\ & 43040\,88132\,67497\,18187\,32948\,54861\,70818\,61261\end{aligned}$$

$$|\ell_{43}(\mathbf{1}) - \hat{\ell}_{43}(\mathbf{1})| \leq 2.19 \times 10^{-287}.$$

$$\begin{aligned}\hat{\ell}_{44}(\mathbf{1}) = & 0.00000\,00000\,00000\,00504\,99392\,91761\,21294\,03581\,84025\,98543 \\ & 94966\,16367\,25017\,79877\,75642\,65859\,12371\,89383\,96314\,60353 \\ & 15760\,51097\,99780\,51542\,46766\,65744\,92076\,61363\,24330\,31598 \\ & 39543\,64510\,44880\,46224\,23660\,62748\,03347\,86691\,35039\,15994 \\ & 28534\,87464\,45230\,69731\,58447\,87747\,08957\,21877\,23331\,87230 \\ & 21010\,17702\,98073\,40981\,43058\,78846\,98419\,6642\end{aligned}$$

$$|\ell_{44}(\mathbf{1}) - \hat{\ell}_{44}(\mathbf{1})| \leq 1.03 \times 10^{-286}.$$

$$\begin{aligned}\hat{\ell}_{45}(\mathbf{1}) = & -0.000000000000000000194930160255073897467808982635176 \\ & 05154518135213910622404081620718059869392494426984 \\ & 99675793244281537550578993859580841567461466803136 \\ & 52769485314577821752792798034172077756215520974517 \\ & 19090143645125313877304390508769633657827686317867 \\ & 998858361497716537389022867541446358695\end{aligned}$$

$$|\ell_{45}(\mathbf{1}) - \hat{\ell}_{45}(\mathbf{1})| \leq 4.88 \times 10^{-286}.$$

$$\begin{aligned}\hat{\ell}_{46}(\mathbf{1}) = & 0.000000000000000000075226954158724014965860796142862 \\ & 60971424353818771769508401236055873045362805764663 \\ & 06657330962887528293304608679942957256300367548972 \\ & 67237991962809377416631128832570064003678448850057 \\ & 22935620379598689065054250307185946466864388966452 \\ & 33827842082691178450506171331910005971\end{aligned}$$

$$|\ell_{46}(\mathbf{1}) - \hat{\ell}_{46}(\mathbf{1})| \leq 2.30 \times 10^{-285}.$$

$$\begin{aligned}\hat{\ell}_{47}(\mathbf{1}) = & -0.000000000000000000029025096503307981266287301536231 \\ & 72287003016347809686189409604284931244483866033430 \\ & 86746682698083993227599071139750418446078150331651 \\ & 08644661301300901610685621447165373058129560089176 \\ & 91094723670352232854030274558027246164117118148429 \\ & 0955799585201291654524997206700642380\end{aligned}$$

$$|\ell_{47}(\mathbf{1}) - \hat{\ell}_{47}(\mathbf{1})| \leq 1.09 \times 10^{-284}.$$

$$\begin{aligned}\hat{\ell}_{48}(\mathbf{1}) = & 0.000000000000000000011196532833624031361439907970968 \\ & 57041231922302091704040350286510747319879927494037 \\ & 07737803403628729538427443781947085987764400170700 \\ & 90684013482171414869739013427715503367404289457551 \\ & 23977558281065003429476416712057857604733932794576 \\ & 8699354459866876146314522561921873373\end{aligned}$$

$$|\ell_{48}(\mathbf{1}) - \hat{\ell}_{48}(\mathbf{1})| \leq 5.13 \times 10^{-284}.$$

$$\begin{aligned}\hat{\ell}_{49}(\mathbf{1}) = & -0.00000\,00000\,00000\,00004\,31824\,05156\,79868\,02922\,39393\,05944 \\ & 71740\,47160\,87386\,26963\,34529\,92429\,84721\,10897\,75020\,82016 \\ & 91903\,84710\,14276\,41527\,67812\,23744\,79550\,80887\,58317\,18142 \\ & 73531\,58072\,50026\,52267\,60062\,18716\,98785\,14989\,61733\,51077 \\ & 77306\,89085\,53409\,69217\,42086\,97780\,15827\,13166\,02175\,16831 \\ & 27509\,21297\,53255\,23332\,56306\,61851\,46106\,7\end{aligned}$$

$$|\ell_{49}(\mathbf{1}) - \hat{\ell}_{49}(\mathbf{1})| \leq 2.42 \times 10^{-283}.$$

$$\begin{aligned}\hat{\ell}_{50}(\mathbf{1}) = & 0.00000\,00000\,00000\,00001\,66512\,54226\,17630\,81195\,26544\,35618 \\ & 62659\,29217\,54463\,40836\,49242\,00435\,75189\,65337\,10785\,36216 \\ & 73364\,47127\,53808\,53677\,94103\,97121\,38763\,53859\,36035\,55020 \\ & 40514\,22043\,53929\,63648\,86567\,75096\,33902\,80075\,54221\,26732 \\ & 74767\,41029\,15922\,88703\,64209\,18189\,61521\,81575\,53581\,07264 \\ & 28317\,81803\,72680\,63902\,33022\,33022\,96907\end{aligned}$$

$$|\ell_{50}(\mathbf{1}) - \hat{\ell}_{50}(\mathbf{1})| \leq 1.14 \times 10^{-282}.$$

## Eigenfunctions

The following figures show the eigenfunctions  $v_j(x)$  evaluated on  $[0.01, 0.99]$  in the shifted monomial basis  $\{(x-1)^k\}_{k=0}^K$ , with  $K = 1024$  (2048-bit precision). Each batch of 10 eigenfunctions is plotted in a  $2 \times 5$  grid.

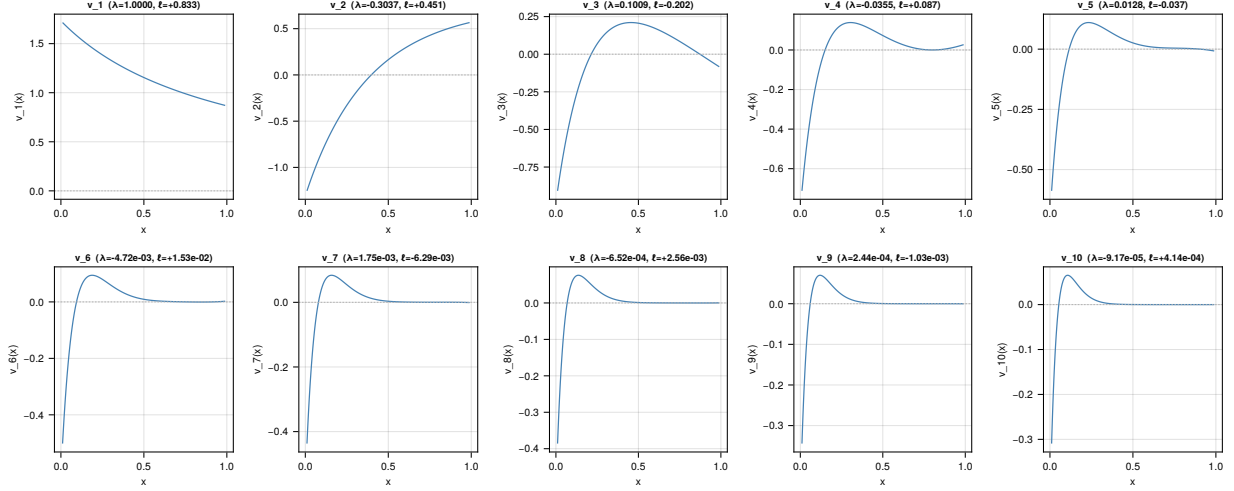

Figure S1: Eigenfunctions  $v_1, \dots, v_{10}$ . The invariant density  $v_1$  (top left) is positive; higher eigenfunctions oscillate with increasing frequency. Each panel shows  $\lambda_j$  and  $\ell_j(1)$ .

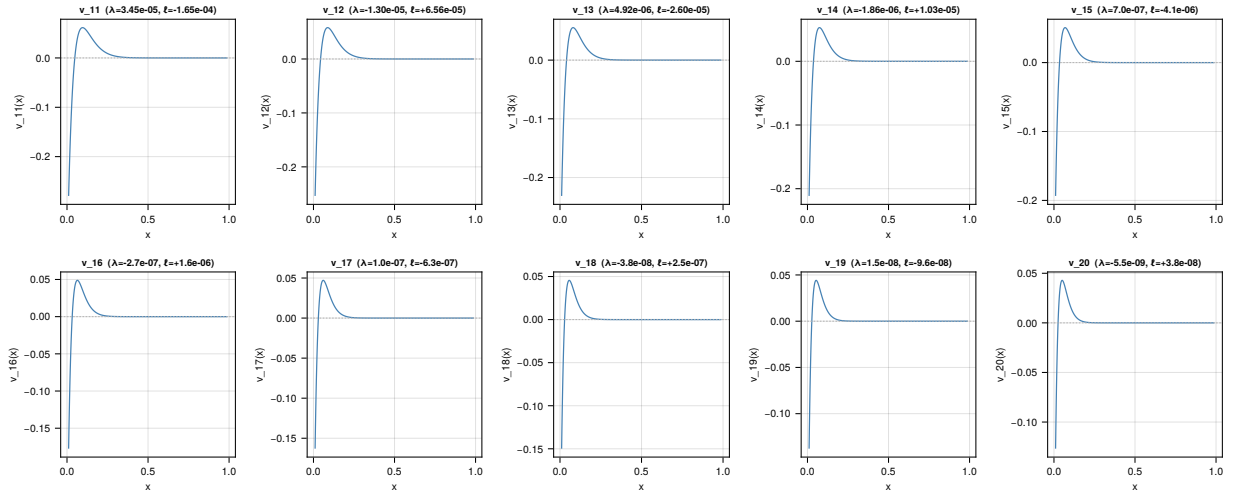

Figure S2: Eigenfunctions  $v_{11}, \dots, v_{20}$ . Eigenvalues  $|\lambda_j| \sim 10^{-5}$ – $10^{-9}$ ; these modes decay rapidly under iteration.

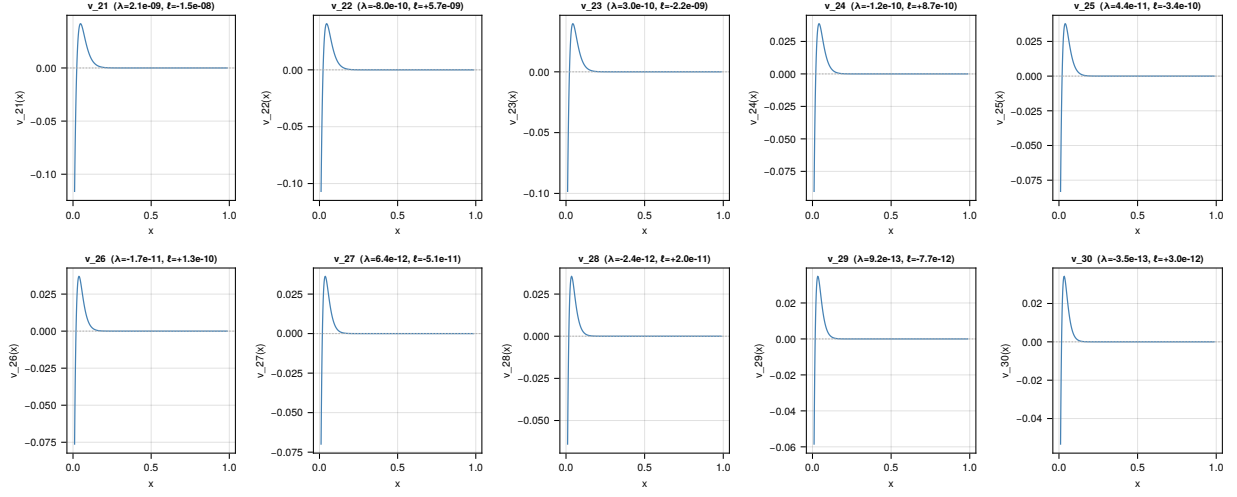

Figure S3: Eigenfunctions  $v_{21}, \dots, v_{30}$ . Eigenvalues  $|\lambda_j| \sim 10^{-9}$ – $10^{-13}$ .

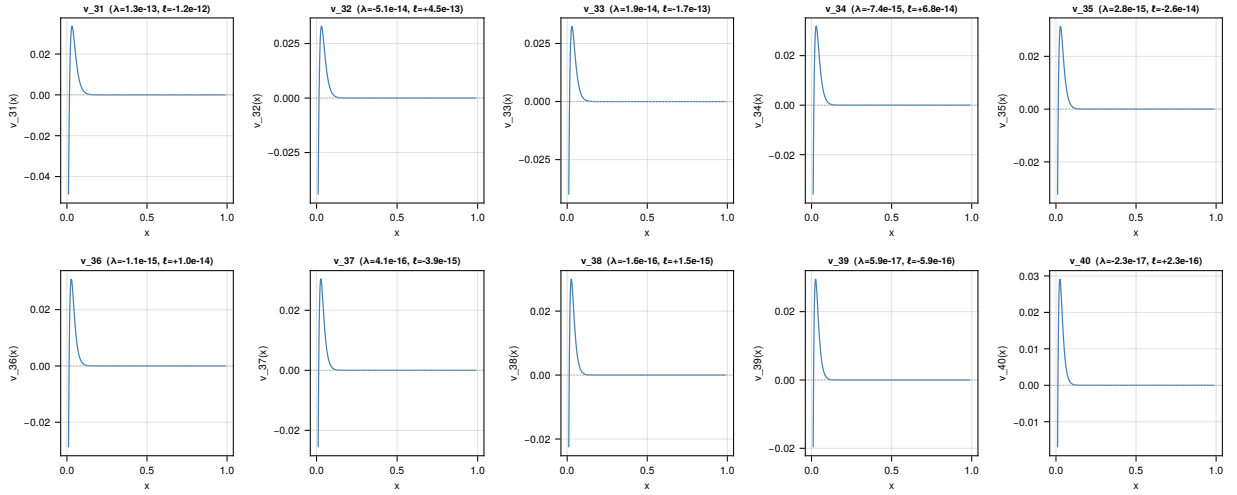

Figure S4: Eigenfunctions  $v_{31}, \dots, v_{40}$ . Eigenvalues  $|\lambda_j| \sim 10^{-13}$ – $10^{-17}$ .

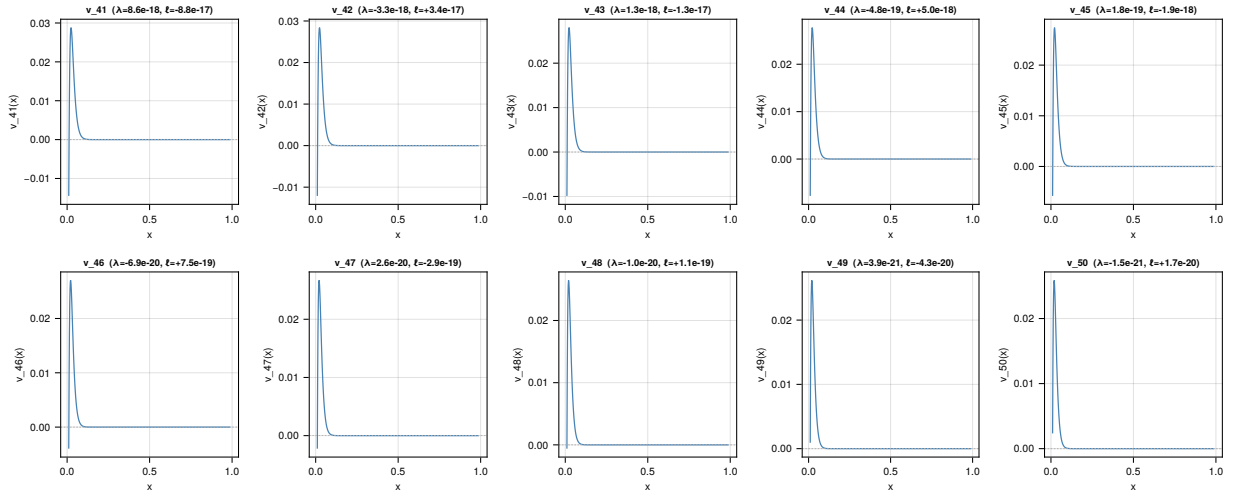

Figure S5: Eigenfunctions  $v_{41}, \dots, v_{50}$ . Eigenvalues  $|\lambda_j| \sim 10^{-17} - 10^{-21}$ .

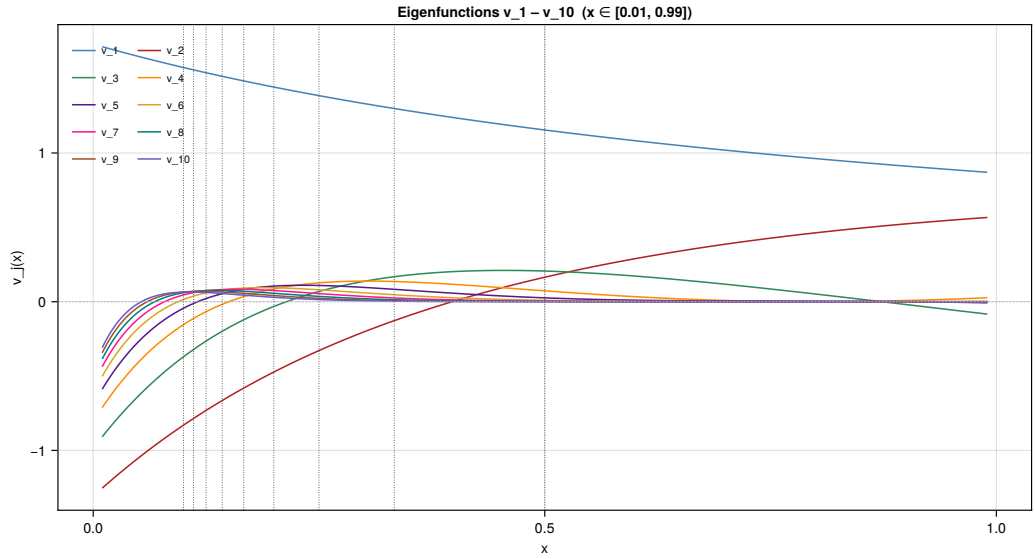

Figure S6: Eigenfunctions  $v_1, \dots, v_{10}$  overlaid with Markov partition (vertical lines at  $x = 1/n$ ,  $n = 2, \dots, 10$ ).

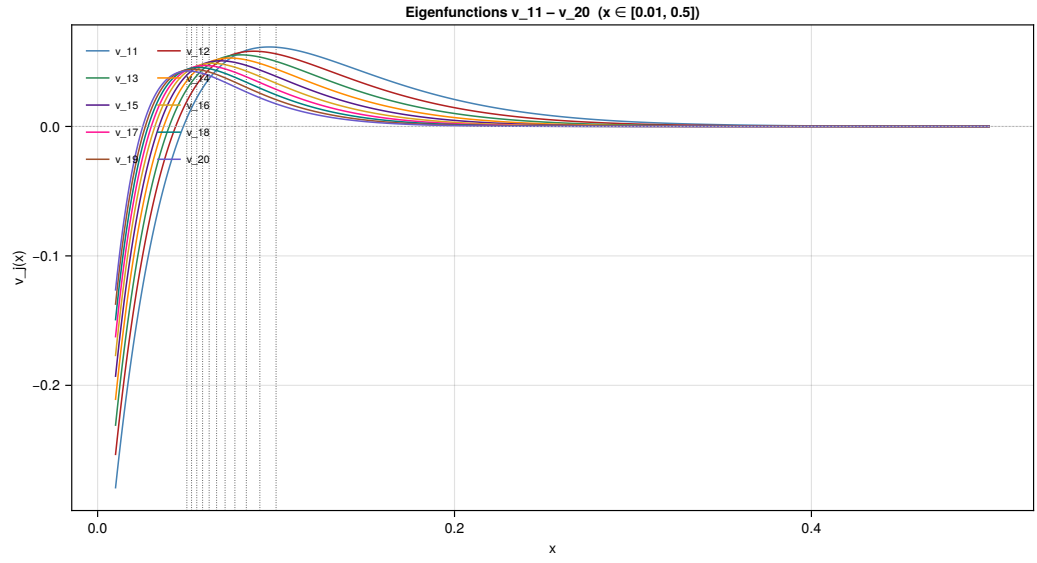

Figure S7: Eigenfunctions  $v_{11}, \dots, v_{20}$  overlaid with Markov partition.

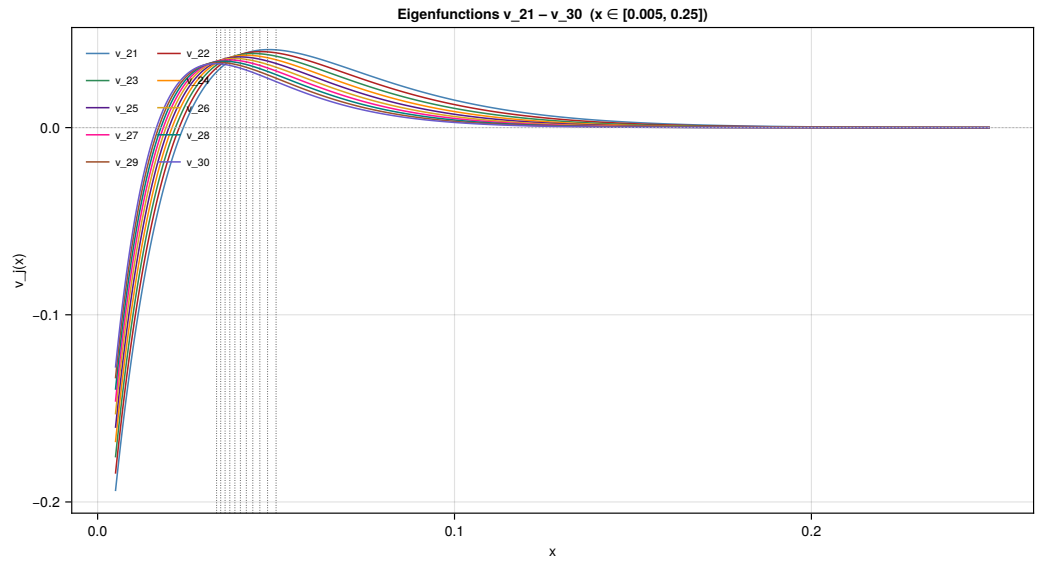

Figure S8: Eigenfunctions  $v_{21}, \dots, v_{30}$  overlaid with Markov partition.

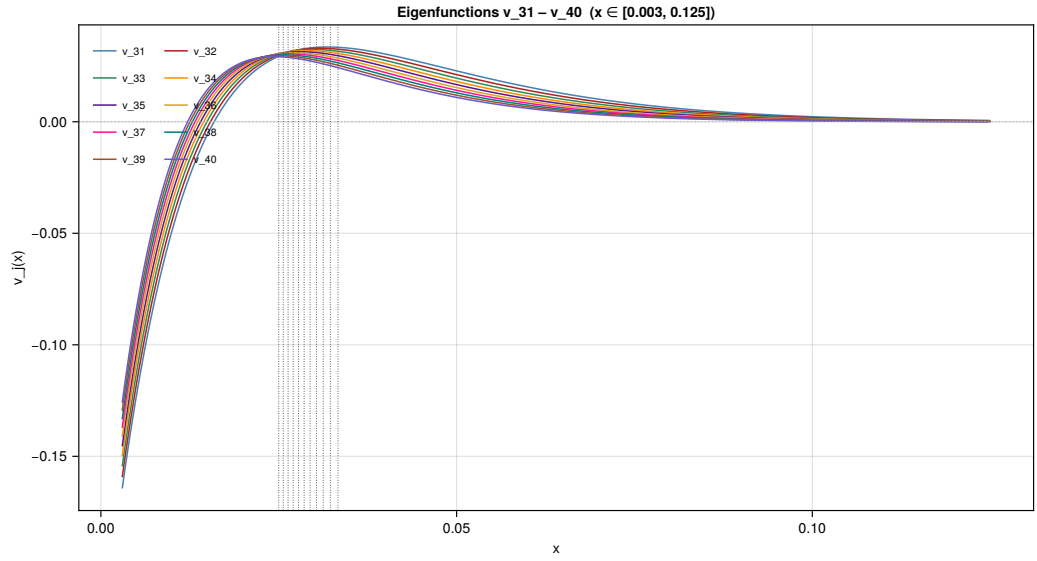

Figure S9: Eigenfunctions  $v_{31}, \dots, v_{40}$  overlaid with Markov partition.

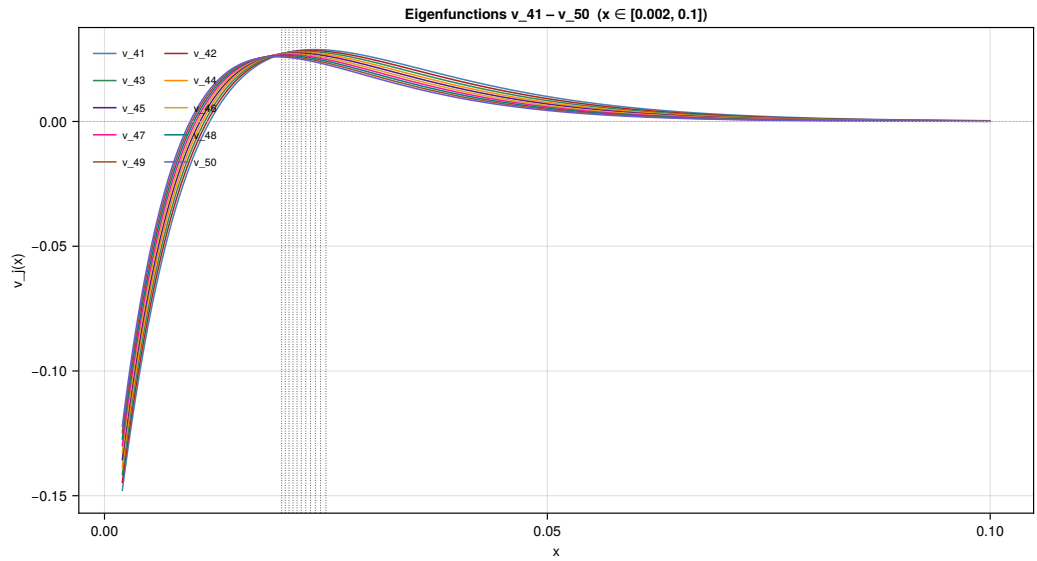

Figure S10: Eigenfunctions  $v_{41}, \dots, v_{50}$  overlaid with Markov partition.

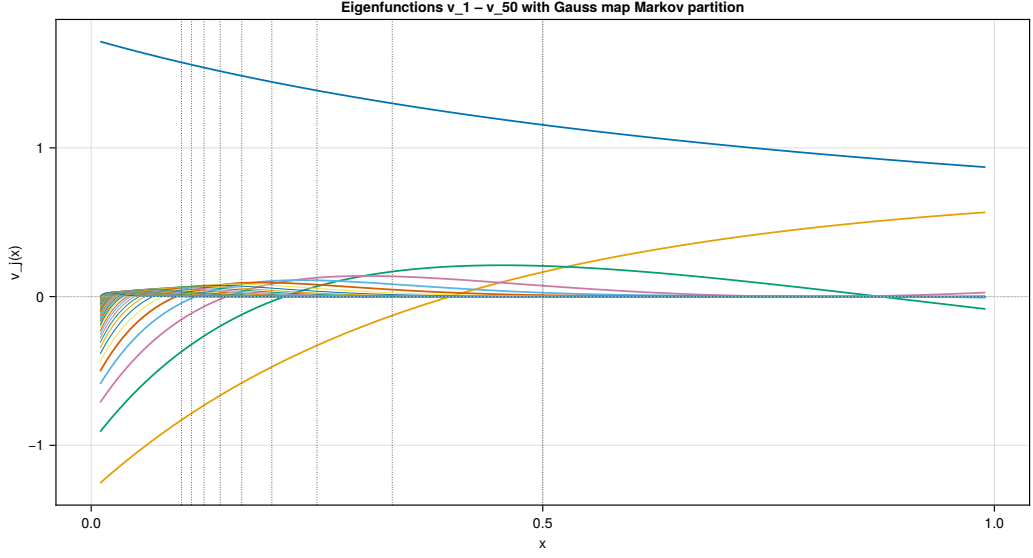

Figure S11: All 50 eigenfunctions overlaid, with Gauss map Markov partition (vertical dotted lines at  $x = 1/n$ ,  $n = 2, \dots, 10$ ).

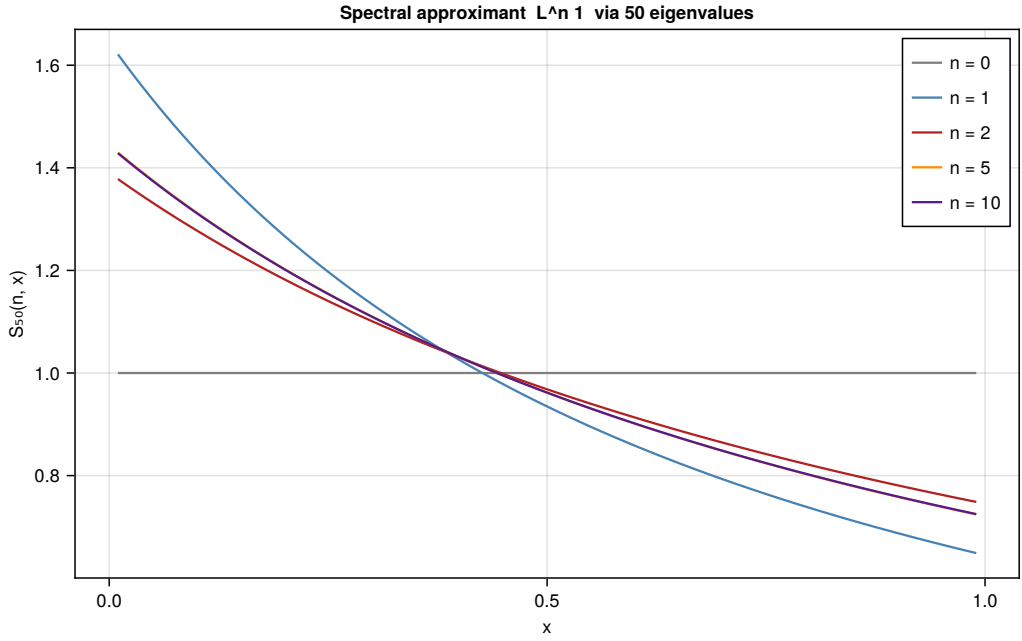

Figure S12: Spectral approximant  $S_{50}(n, x) = \sum_{j=1}^{50} \lambda_j^n \ell_j(\mathbf{1}) v_j(x)$  for  $n = 0, 1, 2, 5, 10$ . At  $n = 0$  the sum reconstructs the constant function  $\mathbf{1}$ ; at  $n = 1$  it approximates the transfer operator applied to  $\mathbf{1}$ ; for large  $n$  it converges to  $\lambda_1^n \ell_1(\mathbf{1}) v_1(x)$ .

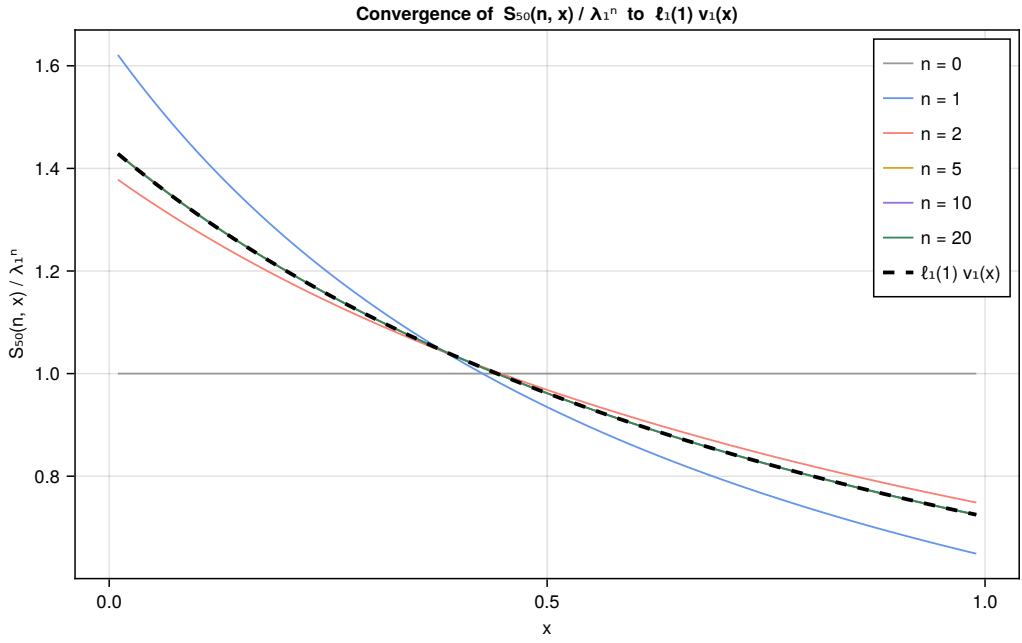

Figure S13: Convergence of  $S_{50}(n, x)/\lambda_1^n$  to the invariant density  $\ell_1(\mathbf{1}) v_1(x)$  (dashed black). The spectral gap  $|\lambda_2/\lambda_1| \approx 0.304$  governs the rate of convergence.

## Eigenvector Coefficients $[v_j]_k$

The following tables list the first 50 coefficients of each unit-norm eigenvector  $v_j$  in the shifted monomial basis  $\{(w-1)^k\}_{k=0}^K$ . The  $\ell^2$  error  $\|\hat{v}_j - v_j\| \leq \delta_j$  shown for each eigenvector is controlled by the Schur orthogonality defect and the reconstruction error from the ordschur + Sylvester pipeline (see Table S6). Eigenvectors at  $K = 1024$  (2048-bit precision) achieve radii  $\sim 10^{-316} - 10^{-282}$ .

$$j = 1: \lambda_1 = 1.000000e + 00, \quad \ell_1(\mathbf{1}) = +8.329404e - 01, \quad \|\hat{v}_1 - v_1\| \leq 3.62e - 162$$

| $k$ | $[v_1]_k$           | $k$ | $[v_1]_k$           |
|-----|---------------------|-----|---------------------|
| 0   | +8.6602540378e - 01 | 25  | -2.5809568280e - 08 |
| 1   | -4.3301270189e - 01 | 26  | +1.2904784140e - 08 |
| 2   | +2.1650635095e - 01 | 27  | -6.4523920699e - 09 |
| 3   | -1.0825317547e - 01 | 28  | +3.2261960349e - 09 |
| 4   | +5.4126587737e - 02 | 29  | -1.6130980175e - 09 |
| 5   | -2.7063293868e - 02 | 30  | +8.0654900873e - 10 |
| 6   | +1.3531646934e - 02 | 31  | -4.0327450437e - 10 |
| 7   | -6.7658234671e - 03 | 32  | +2.0163725218e - 10 |
| 8   | +3.3829117335e - 03 | 33  | -1.0081862609e - 10 |
| 9   | -1.6914558668e - 03 | 34  | +5.0409313046e - 11 |
| 10  | +8.4572793338e - 04 | 35  | -2.5204656523e - 11 |
| 11  | -4.2286396669e - 04 | 36  | +1.2602328261e - 11 |
| 12  | +2.1143198335e - 04 | 37  | -6.3011641307e - 12 |
| 13  | -1.0571599167e - 04 | 38  | +3.1505820654e - 12 |
| 14  | +5.2857995836e - 05 | 39  | -1.5752910327e - 12 |
| 15  | -2.6428997918e - 05 | 40  | +7.8764551634e - 13 |
| 16  | +1.3214498959e - 05 | 41  | -3.9382275817e - 13 |
| 17  | -6.6072494796e - 06 | 42  | +1.9691137909e - 13 |
| 18  | +3.3036247398e - 06 | 43  | -9.8455689543e - 14 |
| 19  | -1.6518123699e - 06 | 44  | +4.9227844771e - 14 |
| 20  | +8.2590618494e - 07 | 45  | -2.4613922386e - 14 |
| 21  | -4.1295309247e - 07 | 46  | +1.2306961193e - 14 |
| 22  | +2.0647654624e - 07 | 47  | -6.1534805964e - 15 |
| 23  | -1.0323827312e - 07 | 48  | +3.0767402982e - 15 |
| 24  | +5.1619136559e - 08 | 49  | -1.5383701491e - 15 |

$$j = 2: \lambda_2 = -3.036630e - 01, \quad \ell_2(\mathbf{1}) = +4.512058e - 01, \quad \|\hat{v}_2 - v_2\| \leq 2.00e - 161$$

| $k$ $[v_2]_k$          | $k$ $[v_2]_k$          |
|------------------------|------------------------|
| 0 $+5.7050920659e-01$  | 25 $+2.1137822436e-07$ |
| 1 $+4.1624549960e-01$  | 26 $-1.0569761625e-07$ |
| 2 $-5.1196167436e-01$  | 27 $+5.2851197768e-08$ |
| 3 $+3.8491986254e-01$  | 28 $-2.6426213142e-08$ |
| 4 $-2.4616997141e-01$  | 29 $+1.3213239926e-08$ |
| 5 $+1.4508248976e-01$  | 30 $-6.6066375954e-09$ |
| 6 $-8.1412161204e-02$  | 31 $+3.3033150334e-09$ |
| 7 $+4.4232939695e-02$  | 32 $-1.6516529702e-09$ |
| 8 $-2.3500357920e-02$  | 33 $+8.2582392107e-10$ |
| 9 $+1.2286594354e-02$  | 34 $-4.1291080660e-10$ |
| 10 $-6.3488447731e-03$ | 35 $+2.0645495059e-10$ |
| 11 $+3.2523318873e-03$ | 36 $-1.0322731864e-10$ |
| 12 $-1.6553890182e-03$ | 37 $+5.1613613481e-11$ |
| 13 $+8.3854489512e-04$ | 38 $-2.5806797425e-11$ |
| 14 $-4.2326095063e-04$ | 39 $+1.2903399301e-11$ |
| 15 $+2.1308196815e-04$ | 40 $-6.4517018099e-12$ |
| 16 $-1.0706384161e-04$ | 41 $+3.2258525849e-12$ |
| 17 $+5.3718283692e-05$ | 42 $-1.6129272967e-12$ |
| 18 $-2.6924831316e-05$ | 43 $+8.0646418026e-13$ |
| 19 $+1.3485294563e-05$ | 44 $-4.0323235203e-13$ |
| 20 $-6.7505119961e-06$ | 45 $+2.0161629853e-13$ |
| 21 $+3.3779201786e-06$ | 46 $-1.0080820435e-13$ |
| 22 $-1.6898475614e-06$ | 47 $+5.0404126138e-14$ |
| 23 $+8.4521363390e-07$ | 48 $-2.5202073187e-14$ |
| 24 $-4.2269924754e-07$ | 49 $+1.2601040747e-14$ |

$$j = 3: \lambda_3 = 1.008845e - 01, \quad \ell_3(\mathbf{1}) = -2.019399e - 01, \quad \|\hat{v}_3 - v_3\| \leq 9.37e - 161$$

| $k$ $[v_3]_k$          | $k$ $[v_3]_k$          |
|------------------------|------------------------|
| 0 $-9.0447344941e-02$  | 25 $+1.4405034690e-06$ |
| 1 $-7.0686601071e-01$  | 26 $-7.2111182399e-07$ |
| 2 $+9.4489856788e-02$  | 27 $+3.6084832338e-07$ |
| 3 $+3.0867750376e-01$  | 28 $-1.8052087863e-07$ |
| 4 $-4.0512541768e-01$  | 29 $+9.0291304149e-08$ |
| 5 $+3.4761664596e-01$  | 30 $-4.5155022432e-08$ |
| 6 $-2.4964571405e-01$  | 31 $+2.2580145600e-08$ |
| 7 $+1.6202173376e-01$  | 32 $-1.1290716982e-08$ |
| 8 $-9.8450913170e-02$  | 33 $+5.6454685428e-09$ |
| 9 $+5.7125257848e-02$  | 34 $-2.8227263359e-09$ |
| 10 $-3.2043727636e-02$ | 35 $+1.4113422414e-09$ |
| 11 $+1.7521112776e-02$ | 36 $-7.0565691808e-10$ |
| 12 $-9.3937359563e-03$ | 37 $+3.5282096728e-10$ |
| 13 $+4.9597294662e-03$ | 38 $-1.7640697401e-10$ |
| 14 $-2.5873265244e-03$ | 39 $+8.8201962240e-11$ |
| 15 $+1.3369832382e-03$ | 40 $-4.4100355916e-11$ |
| 16 $-6.8572831237e-04$ | 41 $+2.2049934531e-11$ |
| 17 $+3.4963821569e-04$ | 42 $-1.1024877405e-11$ |
| 18 $-1.7744974958e-04$ | 43 $+5.5124075668e-12$ |
| 19 $+8.9734547254e-05$ | 44 $-2.7561939091e-12$ |
| 20 $-4.5250271856e-05$ | 45 $+1.3780942688e-12$ |
| 21 $+2.2768685168e-05$ | 46 $-6.8904664447e-13$ |
| 22 $-1.1437476432e-05$ | 47 $+3.4452338541e-13$ |
| 23 $+5.7381449931e-06$ | 48 $-1.7226182909e-13$ |
| 24 $-2.8760584487e-06$ | 49 $+8.6131015376e-14$ |

$$j = 4: \lambda_4 = -3.549616e - 02, \quad \ell_4(\mathbf{1}) = +8.740239e - 02, \quad \|\hat{v}_4 - v_4\| \leq 3.83e - 160$$

| $k$ $[v_4]_k$            | $k$ $[v_4]_k$            |
|--------------------------|--------------------------|
| 0 $+2.9668451307e - 02$  | 25 $+9.3012438559e - 06$ |
| 1 $+2.7924054265e - 01$  | 26 $-4.6825960255e - 06$ |
| 2 $+5.6853860189e - 01$  | 27 $+2.3534773267e - 06$ |
| 3 $-4.4824188327e - 01$  | 28 $-1.1813144791e - 06$ |
| 4 $+3.3409474574e - 02$  | 29 $+5.9235060337e - 07$ |
| 5 $+2.5167800897e - 01$  | 30 $-2.9679138185e - 07$ |
| 6 $-3.4618786849e - 01$  | 31 $+1.4861544706e - 07$ |
| 7 $+3.2023977666e - 01$  | 32 $-7.4384269422e - 08$ |
| 8 $-2.4757279345e - 01$  | 33 $+3.7218012651e - 08$ |
| 9 $+1.7190363582e - 01$  | 34 $-1.8617414047e - 08$ |
| 10 $-1.1098770133e - 01$ | 35 $+9.3112868289e - 09$ |
| 11 $+6.7973144203e - 02$ | 36 $-4.6563649096e - 09$ |
| 12 $-3.9996876950e - 02$ | 37 $+2.3283501234e - 09$ |
| 13 $+2.2812107298e - 02$ | 38 $-1.1641958726e - 09$ |
| 14 $-1.2691930309e - 02$ | 39 $+5.8208892068e - 10$ |
| 15 $+6.9215101502e - 03$ | 40 $-2.9103450369e - 10$ |
| 16 $-3.7136745268e - 03$ | 41 $+1.4551100833e - 10$ |
| 17 $+1.9661656212e - 03$ | 42 $-7.2752230647e - 11$ |
| 18 $-1.0296382006e - 03$ | 43 $+3.6374552655e - 11$ |
| 19 $+5.3437088712e - 04$ | 44 $-1.8186574860e - 11$ |
| 20 $-2.7529049710e - 04$ | 45 $+9.0929869112e - 12$ |
| 21 $+1.4096381725e - 04$ | 46 $-4.5463697302e - 12$ |
| 22 $-7.1824532168e - 05$ | 47 $+2.2731358030e - 12$ |
| 23 $+3.6449132229e - 05$ | 48 $-1.1365491915e - 12$ |
| 24 $-1.8436745987e - 05$ | 49 $+5.6826777399e - 13$ |

$$j = 5: \lambda_5 = 1.284379e - 02, \quad \ell_5(\mathbf{1}) = -3.694616e - 02, \quad \|\hat{v}_5 - v_5\| \leq 1.45e - 159$$

| $k$ $[v_5]_k$            | $k$ $[v_5]_k$            |
|--------------------------|--------------------------|
| 0 $-8.8043043986e - 03$  | 25 $+5.6712684176e - 05$ |
| 1 $-1.2821141655e - 01$  | 26 $-2.8984255395e - 05$ |
| 2 $-4.0620172038e - 01$  | 27 $+1.4751250734e - 05$ |
| 3 $-2.5046189333e - 01$  | 28 $-7.4813774835e - 06$ |
| 4 $+5.3864569107e - 01$  | 29 $+3.7833678490e - 06$ |
| 5 $-3.4385788333e - 01$  | 30 $-1.9087125191e - 06$ |
| 6 $+1.7687881189e - 02$  | 31 $+9.6107039237e - 07$ |
| 7 $+2.1476374450e - 01$  | 32 $-4.8314951109e - 07$ |
| 8 $-3.0753683353e - 01$  | 33 $+2.4257905525e - 07$ |
| 9 $+3.0005617346e - 01$  | 34 $-1.2166964329e - 07$ |
| 10 $-2.4487939302e - 01$ | 35 $+6.0976298735e - 08$ |
| 11 $+1.7911864358e - 01$ | 36 $-3.0539790507e - 08$ |
| 12 $-1.2144537659e - 01$ | 37 $+1.5288308267e - 08$ |
| 13 $+7.7837988391e - 02$ | 38 $-7.6505288082e - 09$ |
| 14 $-4.7763889976e - 02$ | 39 $+3.8273865267e - 09$ |
| 15 $+2.8311025326e - 02$ | 40 $-1.9143609935e - 09$ |
| 16 $-1.6314781544e - 02$ | 41 $+9.5737228056e - 10$ |
| 17 $+9.1859688538e - 03$ | 42 $-4.7873208370e - 10$ |
| 18 $-5.0730711145e - 03$ | 43 $+2.3937206451e - 10$ |
| 19 $+2.7565802706e - 03$ | 44 $-1.1968356974e - 10$ |
| 20 $-1.4775041526e - 03$ | 45 $+5.9838916142e - 11$ |
| 21 $+7.8281931439e - 04$ | 46 $-2.9917598054e - 11$ |
| 22 $-4.1071277215e - 04$ | 47 $+1.4957792419e - 11$ |
| 23 $+2.1370271470e - 04$ | 48 $-7.4783998741e - 12$ |
| 24 $-1.1041605544e - 04$ | 49 $+3.7389693930e - 12$ |

$$j = 6: \lambda_6 = -4.717778e - 03, \quad \ell_6(\mathbf{1}) = +1.534795e - 02, \quad \|\hat{v}_6 - v_6\| \leq 5.27e - 159$$

| $k$ | $[v_6]_k$           | $k$ | $[v_6]_k$           |
|-----|---------------------|-----|---------------------|
| 0   | +2.9288005304e - 03 | 25  | +3.1381308619e - 04 |
| 1   | +5.2713511483e - 02 | 26  | -1.6480576749e - 04 |
| 2   | +2.5758421280e - 01 | 27  | +8.5893432199e - 05 |
| 3   | +3.7733209909e - 01 | 28  | -4.4471579252e - 05 |
| 4   | -8.7332643623e - 02 | 29  | +2.2894637725e - 05 |
| 5   | -3.7954659177e - 01 | 30  | -1.1728959324e - 05 |
| 6   | +4.8680576276e - 01 | 31  | +5.9836173338e - 06 |
| 7   | -2.8921038250e - 01 | 32  | -3.0416841901e - 06 |
| 8   | +1.4754988883e - 02 | 33  | +1.5415053684e - 06 |
| 9   | +1.8736691367e - 01 | 34  | -7.7922335306e - 07 |
| 10  | -2.7901534902e - 01 | 35  | +3.9304657578e - 07 |
| 11  | +2.8413322669e - 01 | 36  | -1.9790044778e - 07 |
| 12  | -2.4217035435e - 01 | 37  | +9.9495772191e - 08 |
| 13  | +1.8484043104e - 01 | 38  | -4.9961213509e - 08 |
| 14  | -1.3057138188e - 01 | 39  | +2.5062840942e - 08 |
| 15  | +8.7022433528e - 02 | 40  | -1.2562613434e - 08 |
| 16  | -5.5410631501e - 02 | 41  | +6.2929196399e - 09 |
| 17  | +3.4005412572e - 02 | 42  | -3.1506873855e - 09 |
| 18  | -2.0244519606e - 02 | 43  | +1.5768401622e - 09 |
| 19  | +1.1749626794e - 02 | 44  | -7.8893057108e - 10 |
| 20  | -6.6741449169e - 03 | 45  | +3.9463051949e - 10 |
| 21  | +3.7221436445e - 03 | 46  | -1.9736447204e - 10 |
| 22  | -2.0433607145e - 03 | 47  | +9.8694741849e - 11 |
| 23  | +1.1066109468e - 03 | 48  | -4.9349373601e - 11 |
| 24  | -5.9230063610e - 04 | 49  | +2.4674256052e - 11 |

$$j = 7: \lambda_7 = 1.748675e - 03, \quad \ell_7(\mathbf{1}) = -6.294980e - 03, \quad \|\hat{v}_7 - v_7\| \leq 1.87e - 158$$

| $k$ | $[v_7]_k$           | $k$ | $[v_7]_k$           |
|-----|---------------------|-----|---------------------|
| 0   | -9.8055287385e - 04 | 25  | +1.5153807365e - 03 |
| 1   | -2.1860588173e - 02 | 26  | -8.2791609363e - 04 |
| 2   | -1.3820176619e - 01 | 27  | +4.4707439112e - 04 |
| 3   | -3.4256938976e - 01 | 28  | -2.3895005724e - 04 |
| 4   | -1.9744018209e - 01 | 29  | +1.2656057412e - 04 |
| 5   | +2.9440585261e - 01 | 30  | -6.6499936385e - 05 |
| 6   | +8.8207678372e - 02 | 31  | +3.4696854350e - 05 |
| 7   | -4.1415744698e - 01 | 32  | -1.7991781746e - 05 |
| 8   | +4.4439275024e - 01 | 33  | +9.2790396749e - 06 |
| 9   | -2.5719478485e - 01 | 34  | -4.7629002568e - 06 |
| 10  | +1.7193970567e - 02 | 35  | +2.4346886257e - 06 |
| 11  | +1.6505458952e - 01 | 36  | -1.2400950839e - 06 |
| 12  | -2.5611455673e - 01 | 37  | +6.2967608130e - 07 |
| 13  | +2.7071961776e - 01 | 38  | -3.1887337166e - 07 |
| 14  | -2.3939660325e - 01 | 39  | +1.6111110867e - 07 |
| 15  | +1.8947230843e - 01 | 40  | -8.1243217250e - 08 |
| 16  | -1.3866088775e - 01 | 41  | +4.0900992244e - 08 |
| 17  | +9.5628348606e - 02 | 42  | -2.0562710360e - 08 |
| 18  | -6.2923782054e - 02 | 43  | +1.0325871095e - 08 |
| 19  | +3.9847890015e - 02 | 44  | -5.1803558743e - 09 |
| 20  | -2.4442242880e - 02 | 45  | +2.5968910133e - 09 |
| 21  | +1.4593481152e - 02 | 46  | -1.3009868701e - 09 |
| 22  | -8.5143110135e - 03 | 47  | +6.5143531766e - 10 |
| 23  | +4.8694811257e - 03 | 48  | -3.2605766464e - 10 |
| 24  | -2.7370962618e - 03 | 49  | +1.6314741925e - 10 |

$$j = 8: \lambda_8 = -6.520209e - 04, \quad \ell_8(\mathbf{1}) = +2.557421e - 03, \quad \|\hat{v}_8 - v_8\| \leq 6.54e - 158$$

| $k$ $[v_8]_k$            | $k$ $[v_8]_k$            |
|--------------------------|--------------------------|
| 0 $+3.3816038721e - 04$  | 25 $+6.2014947319e - 03$ |
| 1 $+8.8712621469e - 03$  | 26 $-3.5661271091e - 03$ |
| 2 $+7.0040265312e - 02$  | 27 $+2.0174580968e - 03$ |
| 3 $+2.3725221109e - 01$  | 28 $-1.1249354472e - 03$ |
| 4 $+3.2135236940e - 01$  | 29 $+6.1924650269e - 04$ |
| 5 $-4.5408229903e - 02$  | 30 $-3.3699277531e - 04$ |
| 6 $-2.9898964426e - 01$  | 31 $+1.8152382819e - 04$ |
| 7 $+1.7562043210e - 01$  | 32 $-9.6889519810e - 05$ |
| 8 $+1.8249405818e - 01$  | 33 $+5.1294747872e - 05$ |
| 9 $-4.1882715750e - 01$  | 34 $-2.6958830190e - 05$ |
| 10 $+4.1193080144e - 01$ | 35 $+1.4076757346e - 05$ |
| 11 $-2.3751440328e - 01$ | 36 $-7.3077905994e - 06$ |
| 12 $+2.2412015993e - 02$ | 37 $+3.7742513570e - 06$ |
| 13 $+1.4574225898e - 01$ | 38 $-1.9403952820e - 06$ |
| 14 $-2.3660112868e - 01$ | 39 $+9.9356040970e - 07$ |
| 15 $+2.5882669856e - 01$ | 40 $-5.0693439770e - 07$ |
| 16 $-2.3645950137e - 01$ | 41 $+2.5784095463e - 07$ |
| 17 $+1.9320544604e - 01$ | 42 $-1.3078741619e - 07$ |
| 18 $-1.4587027901e - 01$ | 43 $+6.6183319911e - 08$ |
| 19 $+1.0370377154e - 01$ | 44 $-3.3422489643e - 08$ |
| 20 $-7.0278596440e - 02$ | 45 $+1.6848507392e - 08$ |
| 21 $+4.5790881619e - 02$ | 46 $-8.4806233509e - 09$ |
| 22 $-2.8867930402e - 02$ | 47 $+4.2632096248e - 09$ |
| 23 $+1.7694940545e - 02$ | 48 $-2.1407970004e - 09$ |
| 24 $-1.0586583669e - 02$ | 49 $+1.0740409385e - 09$ |

$$j = 9: \lambda_9 = 2.441315e - 04, \quad \ell_9(\mathbf{1}) = -1.031415e - 03, \quad \|\hat{v}_9 - v_9\| \leq 2.28e - 157$$

| $k$ $[v_9]_k$            | $k$ $[v_9]_k$            |
|--------------------------|--------------------------|
| 0 $-1.1799547910e - 04$  | 25 $+2.1031142393e - 02$ |
| 1 $-3.5825018552e - 03$  | 26 $-1.2881889170e - 02$ |
| 2 $-3.3725281451e - 02$  | 27 $+7.7187224649e - 03$ |
| 3 $-1.4603058030e - 01$  | 28 $-4.5360503861e - 03$ |
| 4 $-2.9886824515e - 01$  | 29 $+2.6200998185e - 03$ |
| 5 $-1.8545475471e - 01$  | 30 $-1.4902832301e - 03$ |
| 6 $+2.3247141884e - 01$  | 31 $+8.3603637339e - 04$ |
| 7 $+1.3477449923e - 01$  | 32 $-4.6322633391e - 04$ |
| 8 $-2.8813177543e - 01$  | 33 $+2.5380915511e - 04$ |
| 9 $+8.1173431804e - 02$  | 34 $-1.3767079278e - 04$ |
| 10 $+2.3449479102e - 01$ | 35 $+7.3998208039e - 05$ |
| 11 $-4.1289479127e - 01$ | 36 $-3.9448207702e - 05$ |
| 12 $+3.8721655110e - 01$ | 37 $+2.0873984602e - 05$ |
| 13 $-2.2531195759e - 01$ | 38 $-1.0971579021e - 05$ |
| 14 $+2.9238457729e - 02$ | 39 $+5.7319787919e - 06$ |
| 15 $+1.2834557148e - 01$ | 40 $-2.9783320709e - 06$ |
| 16 $-2.1925984696e - 01$ | 41 $+1.5399771601e - 06$ |
| 17 $+2.4787497215e - 01$ | 42 $-7.9277105056e - 07$ |
| 18 $-2.3328565645e - 01$ | 43 $+4.0651382364e - 07$ |
| 19 $+1.9615236620e - 01$ | 44 $-2.0772176822e - 07$ |
| 20 $-1.5229855765e - 01$ | 45 $+1.0581266317e - 07$ |
| 21 $+1.1127777959e - 01$ | 46 $-5.3752382090e - 08$ |
| 22 $-7.7451963565e - 02$ | 47 $+2.7239826076e - 08$ |
| 23 $+5.1792687547e - 02$ | 48 $-1.3774854450e - 08$ |
| 24 $-3.3484691285e - 02$ | 49 $+6.9528595371e - 09$ |

$$j = 10: \lambda_{10} = -9.168908e - 05, \quad \ell_{10}(\mathbf{1}) = +4.135796e - 04, \quad \|\hat{v}_{10} - v_{10}\| \leq 7.92e - 157$$

| $k$ | $[v_{10}]_k$        | $k$ | $[v_{10}]_k$        |
|-----|---------------------|-----|---------------------|
| 0   | +4.1693739426e - 05 | 25  | +5.7817303214e - 02 |
| 1   | +1.4356803898e - 03 | 26  | -3.8259119809e - 02 |
| 2   | +1.5740329954e - 02 | 27  | +2.4579824204e - 02 |
| 3   | +8.2688195017e - 02 | 28  | -1.5389964310e - 02 |
| 4   | +2.2620743416e - 01 | 29  | +9.4199704682e - 03 |
| 5   | +2.7822067868e - 01 | 30  | -5.6509683529e - 03 |
| 6   | -1.1595749712e - 02 | 31  | +3.3295927307e - 03 |
| 7   | -2.7851814217e - 01 | 32  | -1.9304193851e - 03 |
| 8   | +8.6091010633e - 02 | 33  | +1.1030468741e - 03 |
| 9   | +2.1705213403e - 01 | 34  | -6.2204291906e - 04 |
| 10  | -2.4686942041e - 01 | 35  | +3.4662663351e - 04 |
| 11  | +1.2443907115e - 02 | 36  | -1.9106926089e - 04 |
| 12  | +2.6344547145e - 01 | 37  | +1.0428689691e - 04 |
| 13  | -4.0329954443e - 01 | 38  | -5.6410453631e - 05 |
| 14  | +3.6828131879e - 01 | 39  | +3.0263944566e - 05 |
| 15  | -2.1796047790e - 01 | 40  | -1.6115430604e - 05 |
| 16  | +3.7053787775e - 02 | 41  | +8.5230739066e - 06 |
| 17  | +1.1225066617e - 01 | 42  | -4.4797368267e - 06 |
| 18  | -2.0337663545e - 01 | 43  | +2.3412819003e - 06 |
| 19  | +2.3750705199e - 01 | 44  | -1.2173745951e - 06 |
| 20  | -2.2982635410e - 01 | 45  | +6.3004499121e - 07 |
| 21  | +1.9838764906e - 01 | 46  | -3.2470412192e - 07 |
| 22  | -1.5801420611e - 01 | 47  | +1.6670588380e - 07 |
| 23  | +1.1837004459e - 01 | 48  | -8.5295443546e - 08 |
| 24  | -8.4423852514e - 02 | 49  | +4.3507605710e - 08 |

$$j = 11: \lambda_{11} = 3.451655e - 05, \quad \ell_{11}(\mathbf{1}) = -1.650674e - 04, \quad \|\hat{v}_{11} - v_{11}\| \leq 2.75e - 156$$

| $k$ | $[v_{11}]_k$        | $k$ | $[v_{11}]_k$        |
|-----|---------------------|-----|---------------------|
| 0   | -1.4856799781e - 05 | 25  | +1.2499432422e - 01 |
| 1   | -5.7278068075e - 04 | 26  | -9.1176725084e - 02 |
| 2   | -7.1637694239e - 03 | 27  | +6.3833249597e - 02 |
| 3   | -4.4295545512e - 02 | 28  | -4.3160820203e - 02 |
| 4   | -1.5096183323e - 01 | 29  | +2.8319491938e - 02 |
| 5   | -2.7188625823e - 01 | 30  | -1.8099765605e - 02 |
| 6   | -1.6590624973e - 01 | 31  | +1.1302670227e - 02 |
| 7   | +1.8096331602e - 01 | 32  | -6.9136900348e - 03 |
| 8   | +1.7480530397e - 01 | 33  | +4.1513164595e - 03 |
| 9   | -2.3703415193e - 01 | 34  | -2.4513203810e - 03 |
| 10  | -2.7476522023e - 02 | 35  | +1.4257279586e - 03 |
| 11  | +2.4654543560e - 01 | 36  | -8.1788697947e - 04 |
| 12  | -2.0169921280e - 01 | 37  | +4.6333704418e - 04 |
| 13  | -3.6539556280e - 02 | 38  | -2.5948751235e - 04 |
| 14  | +2.7919354800e - 01 | 39  | +1.4380411081e - 04 |
| 15  | -3.9276889886e - 01 | 40  | -7.8929597375e - 05 |
| 16  | +3.5365056420e - 01 | 41  | +4.2940323581e - 05 |
| 17  | -2.1390123647e - 01 | 42  | -2.3171830528e - 05 |
| 18  | +4.5494057165e - 02 | 43  | +1.2411133618e - 05 |
| 19  | +9.7086078846e - 02 | 44  | -6.6021004011e - 06 |
| 20  | -1.8850600773e - 01 | 45  | +3.4899210672e - 06 |
| 21  | +2.2749255813e - 01 | 46  | -1.8341597179e - 06 |
| 22  | -2.2605014548e - 01 | 47  | +9.5886160127e - 07 |
| 23  | +1.9996431926e - 01 | 48  | -4.9884607996e - 07 |
| 24  | -1.6306691331e - 01 | 49  | +2.5837498578e - 07 |

$$j = 12: \lambda_{12} = -1.301770e - 05, \quad \ell_{12}(\mathbf{1}) = +6.562912e - 05, \quad \|\hat{v}_{12} - v_{12}\| \leq 9.56e - 156$$

| $k$ | $[v_{12}]_k$          | $k$ | $[v_{12}]_k$          |
|-----|-----------------------|-----|-----------------------|
| 0   | $+5.3326453385e - 06$ | 25  | $+2.0092202477e - 01$ |
| 1   | $+2.2756510459e - 04$ | 26  | $-1.6749389819e - 01$ |
| 2   | $+3.1994533880e - 03$ | 27  | $+1.3116023367e - 01$ |
| 3   | $+2.2749944884e - 02$ | 28  | $-9.7694842398e - 02$ |
| 4   | $+9.2766484638e - 02$ | 29  | $+6.9812509799e - 02$ |
| 5   | $+2.1767285817e - 01$ | 30  | $-4.8161849885e - 02$ |
| 6   | $+2.4906057084e - 01$ | 31  | $+3.2229384441e - 02$ |
| 7   | $-7.2880184724e - 04$ | 32  | $-2.0999682746e - 02$ |
| 8   | $-2.4549995292e - 01$ | 33  | $+1.3363109696e - 02$ |
| 9   | $+1.0393677854e - 02$ | 34  | $-8.3258752603e - 03$ |
| 10  | $+2.4310591520e - 01$ | 35  | $+5.0897912214e - 03$ |
| 11  | $-1.6179713004e - 01$ | 36  | $-3.0584633835e - 03$ |
| 12  | $-1.0323446777e - 01$ | 37  | $+1.8093342105e - 03$ |
| 13  | $+2.4991258343e - 01$ | 38  | $-1.0552116256e - 03$ |
| 14  | $-1.6088907999e - 01$ | 39  | $+6.0741917329e - 04$ |
| 15  | $-7.1245282290e - 02$ | 40  | $-3.4548596264e - 04$ |
| 16  | $+2.8705639065e - 01$ | 41  | $+1.9434865776e - 04$ |
| 17  | $-3.8240024962e - 01$ | 42  | $-1.0822239296e - 04$ |
| 18  | $+3.4224992398e - 01$ | 43  | $+5.9700425540e - 05$ |
| 19  | $-2.1214532203e - 01$ | 44  | $-3.2649208842e - 05$ |
| 20  | $+5.4328744753e - 02$ | 45  | $+1.7712794772e - 05$ |
| 21  | $+8.2615459497e - 02$ | 46  | $-9.5385491956e - 06$ |
| 22  | $-1.7435718831e - 01$ | 47  | $+5.1015259849e - 06$ |
| 23  | $+2.1767791278e - 01$ | 48  | $-2.7112190900e - 06$ |
| 24  | $-2.2193728096e - 01$ | 49  | $+1.4324663259e - 06$ |

$$j = 13: \lambda_{13} = 4.916782e - 06, \quad \ell_{13}(\mathbf{1}) = -2.600972e - 05, \quad \|\hat{v}_{13} - v_{13}\| \leq 3.33e - 155$$

| $k$ | $[v_{13}]_k$          | $k$ | $[v_{13}]_k$          |
|-----|-----------------------|-----|-----------------------|
| 0   | $-1.9251350393e - 06$ | 25  | $+2.0795837756e - 01$ |
| 1   | $-9.0120688193e - 05$ | 26  | $-2.1747612414e - 01$ |
| 2   | $-1.4071545989e - 03$ | 27  | $+2.0129170113e - 01$ |
| 3   | $-1.1313434202e - 02$ | 28  | $-1.7132377568e - 01$ |
| 4   | $-5.3659908959e - 02$ | 29  | $+1.3687437652e - 01$ |
| 5   | $-1.5458581942e - 01$ | 30  | $-1.0396376707e - 01$ |
| 6   | $-2.5163194528e - 01$ | 31  | $+7.5729727003e - 02$ |
| 7   | $-1.5007440271e - 01$ | 32  | $-5.3236245942e - 02$ |
| 8   | $+1.5241951743e - 01$ | 33  | $+3.6289385302e - 02$ |
| 9   | $+1.8094865039e - 01$ | 34  | $-2.4077661904e - 02$ |
| 10  | $-1.7192716230e - 01$ | 35  | $+1.5596595759e - 02$ |
| 11  | $-1.1489889704e - 01$ | 36  | $-9.8881452546e - 03$ |
| 12  | $+2.4557237593e - 01$ | 37  | $+6.1487178908e - 03$ |
| 13  | $-8.8591648220e - 02$ | 38  | $-3.7568145553e - 03$ |
| 14  | $-1.5055178898e - 01$ | 39  | $+2.2588886915e - 03$ |
| 15  | $+2.4112491343e - 01$ | 40  | $-1.3384391950e - 03$ |
| 16  | $-1.2648307898e - 01$ | 41  | $+7.8243844468e - 04$ |
| 17  | $-9.5709446764e - 02$ | 42  | $-4.5176295674e - 04$ |
| 18  | $+2.9004328791e - 01$ | 43  | $+2.5786523736e - 04$ |
| 19  | $-3.7260755967e - 01$ | 44  | $-1.4563600466e - 04$ |
| 20  | $+3.3329298229e - 01$ | 45  | $+8.1447123843e - 05$ |
| 21  | $-2.1203246136e - 01$ | 46  | $-4.5135807056e - 05$ |
| 22  | $+6.3402917487e - 02$ | 47  | $+2.4802003361e - 05$ |
| 23  | $+6.8682907158e - 02$ | 48  | $-1.3521708824e - 05$ |
| 24  | $-1.6073398510e - 01$ | 49  | $+7.3180468444e - 06$ |

$$j = 14: \lambda_{14} = -1.859307e - 06, \quad \ell_{14}(\mathbf{1}) = +1.027988e - 05, \quad \|\hat{v}_{14} - v_{14}\| \leq 1.16e - 154$$

| $k$ $[v_{14}]_k$       | $k$ $[v_{14}]_k$       |
|------------------------|------------------------|
| 0 +6.9839204447e - 07  | 25 +5.5183102296e - 02 |
| 1 +3.5590437909e - 05  | 26 -1.4750093339e - 01 |
| 2 +6.1120610499e - 04  | 27 +1.9826164119e - 01 |
| 3 +5.4824014243e - 03  | 28 -2.1266086666e - 01 |
| 4 +2.9643512430e - 02  | 29 +2.0109845198e - 01 |
| 5 +1.0100817539e - 01  | 30 -1.7457909549e - 01 |
| 6 +2.1089546142e - 01  | 31 +1.4214115435e - 01 |
| 7 +2.2613606565e - 01  | 32 -1.0997004731e - 01 |
| 8 +3.8586220423e - 03  | 33 +8.1561628605e - 02 |
| 9 -2.2222524508e - 01  | 34 -5.8359654245e - 02 |
| 10 -2.8641204973e - 02 | 35 +4.0479930522e - 02 |
| 11 +2.2532854208e - 01 | 36 -2.7321283018e - 02 |
| 12 -6.5066300773e - 02 | 37 +1.7997574694e - 02 |
| 13 -1.8658213373e - 01 | 38 -1.1600170958e - 02 |
| 14 +2.1834492290e - 01 | 39 +7.3310127987e - 03 |
| 15 -2.7552311101e - 02 | 40 -4.5508207970e - 03 |
| 16 -1.7861462258e - 01 | 41 +2.7791521272e - 03 |
| 17 +2.2733026157e - 01 | 42 -1.6719256136e - 03 |
| 18 -9.8399813265e - 02 | 43 +9.9201702611e - 04 |
| 19 -1.1276964385e - 01 | 44 -5.8113457693e - 04 |
| 20 +2.8992422252e - 01 | 45 +3.3643364330e - 04 |
| 21 -3.6350594136e - 01 | 46 -1.9264434256e - 04 |
| 22 +3.2619624408e - 01 | 47 +1.0918968937e - 04 |
| 23 -2.1310346976e - 01 | 48 -6.1302784273e - 05 |
| 24 +7.2607085163e - 02 | 49 +3.4113866789e - 05 |

$$j = 15: \lambda_{15} = 7.038113e - 07, \quad \ell_{15}(\mathbf{1}) = -4.053403e - 06, \quad \|\hat{v}_{15} - v_{15}\| \leq 4.03e - 154$$

| $k$ $[v_{15}]_k$       | $k$ $[v_{15}]_k$       |
|------------------------|------------------------|
| 0 -2.5440017920e - 07  | 25 -2.1502807213e - 01 |
| 1 -1.4022477968e - 05  | 26 +8.1860360750e - 02 |
| 2 -2.6272062088e - 04  | 27 +4.2043984978e - 02 |
| 3 -2.6012069807e - 03  | 28 -1.3456317163e - 01 |
| 4 -1.5788943361e - 02  | 29 +1.8853772795e - 01 |
| 5 -6.2043814076e - 02  | 30 -2.0749004043e - 01 |
| 6 -1.5722370765e - 01  | 31 +2.0036342236e - 01 |
| 7 -2.3565390879e - 01  | 32 -1.7727808525e - 01 |
| 8 -1.3561427070e - 01  | 33 +1.4696337733e - 01 |
| 9 +1.3325448741e - 01  | 34 -1.1570102844e - 01 |
| 10 +1.8086453250e - 01 | 35 +8.7286618375e - 02 |
| 11 -1.2714887956e - 01 | 36 -6.3509047340e - 02 |
| 12 -1.5026485342e - 01 | 37 +4.4781927369e - 02 |
| 13 +1.9297368195e - 01 | 38 -3.0717812120e - 02 |
| 14 +2.9309212784e - 02 | 39 +2.0559725140e - 02 |
| 15 -2.1910446217e - 01 | 40 -1.3460745442e - 02 |
| 16 +1.8071658077e - 01 | 41 +8.6388384265e - 03 |
| 17 +2.0239796958e - 02 | 42 -5.4444040770e - 03 |
| 18 -1.9415530102e - 01 | 43 +3.3745964472e - 03 |
| 19 +2.1214228010e - 01 | 44 -2.0599280735e - 03 |
| 20 -7.5900765837e - 02 | 45 +1.2398053912e - 03 |
| 21 -1.2440590241e - 01 | 46 -7.3651436339e - 04 |
| 22 +2.8777318166e - 01 | 47 +4.3225702156e - 04 |
| 23 -3.5507923797e - 01 | 48 -2.5084320874e - 04 |
| 24 +3.2051989679e - 01 | 49 +1.4404356517e - 04 |

$$j = 16: \lambda_{16} = -2.666413e - 07, \quad \ell_{16}(\mathbf{1}) = +1.595012e - 06, \quad \|\hat{v}_{16} - v_{16}\| \leq 1.41e - 153$$

| $k$ $[v_{16}]_k$         | $k$ $[v_{16}]_k$         |
|--------------------------|--------------------------|
| 0 $+9.2996230395e - 08$  | 25 $-3.4725646475e - 01$ |
| 1 $+5.5135688933e - 06$  | 26 $+3.1592718589e - 01$ |
| 2 $+1.1193313080e - 04$  | 27 $-2.1756182882e - 01$ |
| 3 $+1.2126129608e - 03$  | 28 $+9.1100549291e - 02$ |
| 4 $+8.1636033175e - 03$  | 29 $+2.9216186478e - 02$ |
| 5 $+3.6316728617e - 02$  | 30 $-1.2185392133e - 01$ |
| 6 $+1.0792745979e - 01$  | 31 $+1.7875253842e - 01$ |
| 7 $+2.0505505174e - 01$  | 32 $-2.0196552123e - 01$ |
| 8 $+2.0743349642e - 01$  | 33 $+1.9910506297e - 01$ |
| 9 $+4.1733275532e - 03$  | 34 $-1.7943588558e - 01$ |
| 10 $-2.0334560247e - 01$ | 35 $+1.5134273703e - 01$ |
| 11 $-5.3398498140e - 02$ | 36 $-1.2114474722e - 01$ |
| 12 $+2.0454995644e - 01$ | 37 $+9.2884488580e - 02$ |
| 13 $-2.7238319182e - 03$ | 38 $-6.8662512632e - 02$ |
| 14 $-2.0186731146e - 01$ | 39 $+4.9176688427e - 02$ |
| 15 $+1.3107653491e - 01$ | 40 $-3.4254239815e - 02$ |
| 16 $+9.9945226519e - 02$ | 41 $+2.3276032422e - 02$ |
| 17 $-2.2698787815e - 01$ | 42 $-1.5467844597e - 02$ |
| 18 $+1.4199152968e - 01$ | 43 $+1.0073630785e - 02$ |
| 19 $+5.6508088239e - 02$ | 44 $-6.4409576907e - 03$ |
| 20 $-2.0172377992e - 01$ | 45 $+4.0493818697e - 03$ |
| 21 $+1.9734367649e - 01$ | 46 $-2.5065755768e - 03$ |
| 22 $-5.8123606009e - 02$ | 47 $+1.5294552637e - 03$ |
| 23 $-1.3200862239e - 01$ | 48 $-9.2089308034e - 04$ |
| 24 $+2.8425834978e - 01$ | 49 $+5.4764936320e - 04$ |

$$j = 17: \lambda_{17} = 1.010906e - 07, \quad \ell_{17}(\mathbf{1}) = -6.265117e - 07, \quad \|\hat{v}_{17} - v_{17}\| \leq 4.91e - 153$$

| $k$ $[v_{17}]_k$         | $k$ $[v_{17}]_k$         |
|--------------------------|--------------------------|
| 0 $-3.4098551032e - 08$  | 25 $-1.3656541888e - 01$ |
| 1 $-2.1640736846e - 06$  | 26 $+2.7980383065e - 01$ |
| 2 $-4.7328370576e - 05$  | 27 $-3.3994753162e - 01$ |
| 3 $-5.5690960434e - 04$  | 28 $+3.1215642565e - 01$ |
| 4 $-4.1180222676e - 03$  | 29 $-2.2051930465e - 01$ |
| 5 $-2.0448659427e - 02$  | 30 $+1.0027807240e - 01$ |
| 6 $-6.9606992142e - 02$  | 31 $+1.6666296356e - 02$ |
| 7 $-1.5914504313e - 01$  | 32 $-1.0932638994e - 01$ |
| 8 $-2.2227375851e - 01$  | 33 $+1.6888356888e - 01$ |
| 9 $-1.2260963819e - 01$  | 34 $-1.9609184136e - 01$ |
| 10 $+1.2076214445e - 01$ | 35 $+1.9734000776e - 01$ |
| 11 $+1.7649142663e - 01$ | 36 $-1.8106544613e - 01$ |
| 12 $-9.2684322852e - 02$ | 37 $+1.5528017812e - 01$ |
| 13 $-1.6719411743e - 01$ | 38 $-1.2628987850e - 01$ |
| 14 $+1.4401093290e - 01$ | 39 $+9.8336217071e - 02$ |
| 15 $+9.5602693572e - 02$ | 40 $-7.3799094751e - 02$ |
| 16 $-2.0484006442e - 01$ | 41 $+5.3645880739e - 02$ |
| 17 $+6.4731864945e - 02$ | 42 $-3.7917312144e - 02$ |
| 18 $+1.4809281929e - 01$ | 43 $+2.6138849977e - 02$ |
| 19 $-2.2068691126e - 01$ | 44 $-1.7618679083e - 02$ |
| 20 $+1.0624231190e - 01$ | 45 $+1.1636124136e - 02$ |
| 21 $+8.3532790173e - 02$ | 46 $-7.5433439992e - 03$ |
| 22 $-2.0430717426e - 01$ | 47 $+4.8073369108e - 03$ |
| 23 $+1.8376263311e - 01$ | 48 $-3.0158419719e - 03$ |
| 24 $-4.4267212927e - 02$ | 49 $+1.8645938566e - 03$ |

$$j = 18: \lambda_{18} = -3.834970e - 08, \quad \ell_{18}(\mathbf{1}) = +2.457002e - 07, \quad \|\hat{v}_{18} - v_{18}\| \leq 1.72e - 152$$

| $k$ | $[v_{18}]_k$        | $k$ | $[v_{18}]_k$        |
|-----|---------------------|-----|---------------------|
| 0   | +1.2536120551e - 08 | 25  | +1.7172887351e - 01 |
| 1   | +8.4807341810e - 07 | 26  | -3.3644388194e - 02 |
| 2   | +1.9880091518e - 05 | 27  | -1.3878722065e - 01 |
| 3   | +2.5250997382e - 04 | 28  | +2.7468309857e - 01 |
| 4   | +2.0343801499e - 03 | 29  | -3.3305994586e - 01 |
| 5   | +1.1151032091e - 02 | 30  | +3.0900148747e - 01 |
| 6   | +4.2734393241e - 02 | 31  | -2.2375675350e - 01 |
| 7   | +1.1381885071e - 01 | 32  | +1.0935212066e - 01 |
| 8   | +1.9979660368e - 01 | 33  | +4.3724105691e - 03 |
| 9   | +1.9145447805e - 01 | 34  | -9.6948356775e - 02 |
| 10  | +2.3229228209e - 03 | 35  | +1.5891698730e - 01 |
| 11  | -1.8869298308e - 01 | 36  | -1.8987570196e - 01 |
| 12  | -6.7934583203e - 02 | 37  | +1.9508369697e - 01 |
| 13  | +1.8225094020e - 01 | 38  | -1.8217818845e - 01 |
| 14  | +4.1748510917e - 02 | 39  | +1.5877619403e - 01 |
| 15  | -1.9608195552e - 01 | 40  | -1.3112571452e - 01 |
| 16  | +5.8204060839e - 02 | 41  | +1.0362382477e - 01 |
| 17  | +1.5681113453e - 01 | 42  | -7.8898679318e - 02 |
| 18  | -1.8049254621e - 01 | 43  | +5.8171488577e - 02 |
| 19  | +4.9198206331e - 03 | 44  | -4.1693557471e - 02 |
| 20  | +1.7841017445e - 01 | 45  | +2.9139951766e - 02 |
| 21  | -2.0695023006e - 01 | 46  | -1.9909739735e - 02 |
| 22  | +7.4944967825e - 02 | 47  | +1.3326373626e - 02 |
| 23  | +1.0340618680e - 01 | 48  | -8.7538933653e - 03 |
| 24  | -2.0384448613e - 01 | 49  | +5.6519408554e - 03 |

$$j = 19: \lambda_{19} = 1.455614e - 08, \quad \ell_{19}(\mathbf{1}) = -9.622052e - 08, \quad \|\hat{v}_{19} - v_{19}\| \leq 6.00e - 152$$

| $k$ | $[v_{19}]_k$        | $k$ | $[v_{19}]_k$        |
|-----|---------------------|-----|---------------------|
| 0   | -4.6196522899e - 09 | 25  | +1.1784115736e - 01 |
| 1   | -3.3188936729e - 07 | 26  | -2.0158750590e - 01 |
| 2   | -8.3023730111e - 06 | 27  | +1.6131431421e - 01 |
| 3   | -1.1322378885e - 04 | 28  | -2.5685267346e - 02 |
| 4   | -9.8719943622e - 04 | 29  | -1.3919293855e - 01 |
| 5   | -5.9192441604e - 03 | 30  | +2.6907469761e - 01 |
| 6   | -2.5203893273e - 02 | 31  | -3.2650636071e - 01 |
| 7   | -7.6474071929e - 02 | 32  | +3.0629800540e - 01 |
| 8   | -1.6048505755e - 01 | 33  | -2.2716060579e - 01 |
| 9   | -2.1063495521e - 01 | 34  | +1.1828815140e - 01 |
| 10  | -1.1067969063e - 01 | 35  | -7.6789087845e - 03 |
| 11  | +1.1239356380e - 01 | 36  | -8.4698446206e - 02 |
| 12  | +1.7086512800e - 01 | 37  | +1.4884558178e - 01 |
| 13  | -6.7538992861e - 02 | 38  | -1.8332561717e - 01 |
| 14  | -1.7165461730e - 01 | 39  | +1.9235082731e - 01 |
| 15  | +9.9035014500e - 02 | 40  | -1.8278450402e - 01 |
| 16  | +1.3533774098e - 01 | 41  | +1.6183106417e - 01 |
| 17  | -1.6981569664e - 01 | 42  | -1.3564216425e - 01 |
| 18  | -2.2210476777e - 02 | 43  | +1.0873027636e - 01 |
| 19  | +1.8617134569e - 01 | 44  | -8.3941908372e - 02 |
| 20  | -1.4361631722e - 01 | 45  | +6.2735787968e - 02 |
| 21  | -4.4733303701e - 02 | 46  | -4.5569311557e - 02 |
| 22  | +1.9568504377e - 01 | 47  | +3.2270578369e - 02 |
| 23  | -1.8990383793e - 01 | 48  | -2.2336838078e - 02 |
| 24  | +4.8345292430e - 02 | 49  | +1.5143776347e - 02 |

$$j = 20: \lambda_{20} = -5.527568e - 09, \quad \ell_{20}(\mathbf{1}) = +3.763392e - 08, \quad \|\hat{v}_{20} - v_{20}\| \leq 2.10e - 151$$

| $k$ | $[v_{20}]_k$        | $k$ | $[v_{20}]_k$        |
|-----|---------------------|-----|---------------------|
| 0   | +1.7059246344e - 09 | 25  | -1.7197266599e - 01 |
| 1   | +1.2972248512e - 07 | 26  | +2.6147097823e - 02 |
| 2   | +3.4495679690e - 06 | 27  | +1.2817274074e - 01 |
| 3   | +5.0275713287e - 05 | 28  | -1.9834031291e - 01 |
| 4   | +4.7166922523e - 04 | 29  | +1.5246147155e - 01 |
| 5   | +3.0705964380e - 03 | 30  | -1.9924058437e - 02 |
| 6   | +1.4375423448e - 02 | 31  | -1.3816663689e - 01 |
| 7   | +4.8885722595e - 02 | 32  | +2.6309633388e - 01 |
| 8   | +1.1887846966e - 01 | 33  | -3.2020764939e - 01 |
| 9   | +1.9488399384e - 01 | 34  | +3.0391348094e - 01 |
| 10  | +1.7739173543e - 01 | 35  | -2.3063961639e - 01 |
| 11  | -8.4328050351e - 04 | 36  | +1.2705622557e - 01 |
| 12  | -1.7706713617e - 01 | 37  | -1.9494769483e - 02 |
| 13  | -7.6550582688e - 02 | 38  | -7.2563495516e - 02 |
| 14  | +1.6230633866e - 01 | 39  | +1.3866728575e - 01 |
| 15  | +7.1039066088e - 02 | 40  | -1.7645164731e - 01 |
| 16  | -1.7760845889e - 01 | 41  | +1.8915568161e - 01 |
| 17  | -2.1134169777e - 03 | 42  | -1.8289413340e - 01 |
| 18  | +1.7868088205e - 01 | 43  | +1.6444504563e - 01 |
| 19  | -1.1743579090e - 01 | 44  | -1.3982976486e - 01 |
| 20  | -8.5648360077e - 02 | 45  | +1.1363941219e - 01 |
| 21  | +1.9261939711e - 01 | 46  | -8.8910120073e - 02 |
| 22  | -1.0310831877e - 01 | 47  | +6.7321331191e - 02 |
| 23  | -8.4011964101e - 02 | 48  | -4.9530742098e - 02 |
| 24  | +2.0386780236e - 01 | 49  | +3.5521478683e - 02 |

$$j = 21: \lambda_{21} = 2.099914e - 09, \quad \ell_{21}(\mathbf{1}) = -1.470261e - 08, \quad \|\hat{v}_{21} - v_{21}\| \leq 7.34e - 151$$

| $k$ | $[v_{21}]_k$        | $k$ | $[v_{21}]_k$        |
|-----|---------------------|-----|---------------------|
| 0   | -6.3112920693e - 10 | 25  | -1.1407814914e - 01 |
| 1   | -5.0646933860e - 08 | 26  | +2.0594464494e - 01 |
| 2   | -1.4267534045e - 06 | 27  | -1.5452204276e - 01 |
| 3   | -2.2132562200e - 05 | 28  | +7.8511071689e - 03 |
| 4   | -2.2231306122e - 04 | 29  | +1.3541707196e - 01 |
| 5   | -1.5614631328e - 03 | 30  | -1.9461525185e - 01 |
| 6   | -7.9695262978e - 03 | 31  | +1.4505234478e - 01 |
| 7   | -2.9996517155e - 02 | 32  | -1.5981870119e - 02 |
| 8   | -8.2736317963e - 02 | 33  | -1.3599652870e - 01 |
| 9   | -1.6133355966e - 01 | 34  | +2.5682622485e - 01 |
| 10  | -2.0019411599e - 01 | 35  | -3.1409379431e - 01 |
| 11  | -9.9623682490e - 02 | 36  | +3.0174008355e - 01 |
| 12  | +1.0684287787e - 01 | 37  | -2.3411938955e - 01 |
| 13  | +1.6482106769e - 01 | 38  | +1.3562988243e - 01 |
| 14  | -4.8949229275e - 02 | 39  | -3.1077488275e - 02 |
| 15  | -1.7022749919e - 01 | 40  | -6.0536652640e - 02 |
| 16  | +6.2276720019e - 02 | 41  | +1.2838409429e - 01 |
| 17  | +1.5402826841e - 01 | 42  | -1.6926519333e - 01 |
| 18  | -1.2505999281e - 01 | 43  | +1.8551237253e - 01 |
| 19  | -8.5550117104e - 02 | 44  | -1.8251645775e - 01 |
| 20  | +1.8264489364e - 01 | 45  | +1.6661852901e - 01 |
| 21  | -5.8125032449e - 02 | 46  | -1.4367970005e - 01 |
| 22  | -1.3025578142e - 01 | 47  | +1.1833590273e - 01 |
| 23  | +1.8425252641e - 01 | 48  | -9.3785307087e - 02 |
| 24  | -6.3808192716e - 02 | 49  | +7.1910939578e - 02 |

$$j = 22: \lambda_{22} = -7.980458e - 10, \quad \ell_{22}(\mathbf{1}) = +5.737986e - 09, \quad \|\hat{v}_{22} - v_{22}\| \leq 2.57e - 150$$

| $k$ $[v_{22}]_k$       | $k$ $[v_{22}]_k$       |
|------------------------|------------------------|
| 0 +2.3388513408e - 10  | 25 +1.6720760999e - 01 |
| 1 +1.9753910029e - 08  | 26 -2.8053360802e - 02 |
| 2 +5.8770580534e - 07  | 27 -1.3649800760e - 01 |
| 3 +9.6686981119e - 06  | 28 +2.0407453226e - 01 |
| 4 +1.0353185802e - 04  | 29 -1.3827283917e - 01 |
| 5 +7.8033021831e - 04  | 30 -7.0836196281e - 03 |
| 6 +4.3113729372e - 03  | 31 +1.4033841488e - 01 |
| 7 +1.7783559924e - 02  | 32 -1.9073408544e - 01 |
| 8 +5.4770239462e - 02  | 33 +1.3894524396e - 01 |
| 9 +1.2323822761e - 01  | 34 -1.3550371867e - 02 |
| 10 +1.9017167299e - 01 | 35 -1.3290188898e - 01 |
| 11 +1.6471447265e - 01 | 36 +2.5031673431e - 01 |
| 12 -4.7850796728e - 03 | 37 -3.0810373645e - 01 |
| 13 -1.6776969302e - 01 | 38 +2.9968934129e - 01 |
| 14 -8.1296996863e - 02 | 39 -2.3753848648e - 01 |
| 15 +1.4506886517e - 01 | 40 +1.4398536699e - 01 |
| 16 +9.0374064261e - 02 | 41 -4.2425725335e - 02 |
| 17 -1.5559774285e - 01 | 42 -4.8615972325e - 02 |
| 18 -4.6243310937e - 02 | 43 +1.1800125112e - 01 |
| 19 +1.7507430693e - 01 | 44 -1.6177883397e - 01 |
| 20 -5.1351426055e - 02 | 45 +1.8143502367e - 01 |
| 21 -1.4042756998e - 01 | 46 -1.8166072495e - 01 |
| 22 +1.6152275788e - 01 | 47 +1.6835216575e - 01 |
| 23 -2.3301810388e - 03 | 48 -1.4718382205e - 01 |
| 24 -1.5825917493e - 01 | 49 +1.2280521956e - 01 |

$$j = 23: \lambda_{23} = 3.033863e - 10, \quad \ell_{23}(\mathbf{1}) = -2.237249e - 09, \quad \|\hat{v}_{23} - v_{23}\| \leq 9.00e - 150$$

| $k$ $[v_{23}]_k$       | $k$ $[v_{23}]_k$       |
|------------------------|------------------------|
| 0 -8.6804571889e - 11  | 25 +4.5285570024e - 02 |
| 1 -7.6975883194e - 09  | 26 -1.7310729218e - 01 |
| 2 -2.4119731656e - 07  | 27 +1.4574336073e - 01 |
| 3 -4.1948155614e - 06  | 28 +3.2620016822e - 03 |
| 4 -4.7702008988e - 05  | 29 -1.5281166826e - 01 |
| 5 -3.8401774639e - 04  | 30 +1.9977731335e - 01 |
| 6 -2.2831551706e - 03  | 31 -1.2356150571e - 01 |
| 7 -1.0237480310e - 02  | 32 -1.9167514366e - 02 |
| 8 -3.4786144530e - 02  | 33 +1.4350821274e - 01 |
| 9 -8.8461997270e - 02  | 34 -1.8689373833e - 01 |
| 10 -1.6174907672e - 01 | 35 +1.3399415336e - 01 |
| 11 -1.9060592490e - 01 | 36 -1.2377780355e - 02 |
| 12 -8.9273138066e - 02 | 37 -1.2905185766e - 01 |
| 13 +1.0322918430e - 01 | 38 +2.4360322791e - 01 |
| 14 +1.5884384712e - 01 | 39 -3.0218476337e - 01 |
| 15 -3.5291651870e - 02 | 40 +2.9768817511e - 01 |
| 16 -1.6572870469e - 01 | 41 -2.4084561045e - 01 |
| 17 +3.2815011623e - 02 | 42 +1.5210109376e - 01 |
| 18 +1.6032218229e - 01 | 43 -5.3535337935e - 02 |
| 19 -8.2146566674e - 02 | 44 -3.6803359985e - 02 |
| 20 -1.2357119205e - 01 | 45 +1.0752662689e - 01 |
| 21 +1.5208919982e - 01 | 46 -1.5400619319e - 01 |
| 22 +2.0318168609e - 02 | 47 +1.7693790421e - 01 |
| 23 -1.6811880553e - 01 | 48 -1.8033622563e - 01 |
| 24 +1.2713595975e - 01 | 49 +1.6964697237e - 01 |

$$j = 24: \lambda_{24} = -1.153695e - 10, \quad \ell_{24}(\mathbf{1}) = +8.715538e - 10, \quad \|\hat{v}_{24} - v_{24}\| \leq 3.15e - 149$$

| $k$ | $[v_{24}]_k$        | $k$ | $[v_{24}]_k$        |
|-----|---------------------|-----|---------------------|
| 0   | +3.2260982235e - 11 | 25  | -1.7443291719e - 01 |
| 1   | +2.9970391679e - 09 | 26  | +8.7694907819e - 02 |
| 2   | +9.8658898015e - 08 | 27  | +8.3388961894e - 02 |
| 3   | +1.8086751407e - 06 | 28  | -1.7820267686e - 01 |
| 4   | +2.1768814091e - 05 | 29  | +1.2264724459e - 01 |
| 5   | +1.8641797134e - 04 | 30  | +3.0027512598e - 02 |
| 6   | +1.1865918093e - 03 | 31  | -1.6436808299e - 01 |
| 7   | +5.7450758300e - 03 | 32  | +1.9410290130e - 01 |
| 8   | +2.1333514019e - 02 | 33  | -1.1050022868e - 01 |
| 9   | +6.0390944436e - 02 | 34  | -2.8852558302e - 02 |
| 10  | +1.2699126303e - 01 | 35  | +1.4535253454e - 01 |
| 11  | +1.8556184101e - 01 | 36  | -1.8320924090e - 01 |
| 12  | +1.5307489812e - 01 | 37  | +1.3005851741e - 01 |
| 13  | -9.1921527600e - 03 | 38  | -1.2257384996e - 02 |
| 14  | -1.6023014082e - 01 | 39  | -1.2457873557e - 01 |
| 15  | -8.3530590452e - 02 | 40  | +2.3670990710e - 01 |
| 16  | +1.3059964651e - 01 | 41  | -2.9629172774e - 01 |
| 17  | +1.0275567550e - 01 | 42  | +2.9567590109e - 01 |
| 18  | -1.3337106208e - 01 | 43  | -2.4399753960e - 01 |
| 19  | -7.7500253821e - 02 | 44  | +1.5995727127e - 01 |
| 20  | +1.5884275331e - 01 | 45  | -6.4400035097e - 02 |
| 21  | +4.3982794937e - 03 | 46  | -2.5103762820e - 02 |
| 22  | -1.6115909395e - 01 | 47  | +9.6970234771e - 02 |
| 23  | +1.0550307284e - 01 | 48  | -1.4596182935e - 01 |
| 24  | +7.8951045167e - 02 | 49  | +1.7203552842e - 01 |

$$j = 25: \lambda_{25} = 4.388345e - 11, \quad \ell_{25}(\mathbf{1}) = -3.392576e - 10, \quad \|\hat{v}_{25} - v_{25}\| \leq 1.11e - 148$$

| $k$ | $[v_{25}]_k$        | $k$ | $[v_{25}]_k$        |
|-----|---------------------|-----|---------------------|
| 0   | -1.2004798857e - 11 | 25  | +5.0868194365e - 02 |
| 1   | -1.1659941593e - 09 | 26  | +1.2124394340e - 01 |
| 2   | -4.0232865913e - 08 | 27  | -1.6579902758e - 01 |
| 3   | -7.7546769681e - 07 | 28  | +4.8300081486e - 02 |
| 4   | -9.8486812230e - 06 | 29  | +1.1235821092e - 01 |
| 5   | -8.9393771905e - 05 | 30  | -1.7643370655e - 01 |
| 6   | -6.0649683811e - 04 | 31  | +9.9652310905e - 02 |
| 7   | -3.1527747726e - 03 | 32  | +5.2526145634e - 02 |
| 8   | -1.2695420231e - 02 | 33  | -1.7228288246e - 01 |
| 9   | -3.9543231573e - 02 | 34  | +1.8776473276e - 01 |
| 10  | -9.3702479929e - 02 | 35  | -9.9074515311e - 02 |
| 11  | -1.6177283367e - 01 | 36  | -3.6525641803e - 02 |
| 12  | -1.8163749309e - 01 | 37  | +1.4618863292e - 01 |
| 13  | -7.9506782170e - 02 | 38  | -1.7974194723e - 01 |
| 14  | +1.0098240660e - 01 | 39  | +1.2700777520e - 01 |
| 15  | +1.5310714279e - 01 | 40  | -1.3018363122e - 02 |
| 16  | -2.5289911146e - 02 | 41  | -1.1958749498e - 01 |
| 17  | -1.5991364349e - 01 | 42  | +2.2965369797e - 01 |
| 18  | +9.7098207038e - 03 | 43  | -2.9038624057e - 01 |
| 19  | +1.5898323358e - 01 | 44  | +2.9360193875e - 01 |
| 20  | -4.4222390707e - 02 | 45  | -2.4695758792e - 01 |
| 21  | -1.4326661134e - 01 | 46  | +1.6753563800e - 01 |
| 22  | +1.1199762852e - 01 | 47  | -7.5011888517e - 02 |
| 23  | +7.7666370784e - 02 | 48  | -1.3524539790e - 02 |
| 24  | -1.6509458703e - 01 | 49  | +8.6343846240e - 02 |

$$j = 26: \lambda_{26} = -1.669605e - 11, \quad \ell_{26}(\mathbf{1}) = +1.319616e - 10, \quad \|\hat{v}_{26} - v_{26}\| \leq 3.88e - 148$$

| $k$ $[v_{26}]_k$         | $k$ $[v_{26}]_k$         |
|--------------------------|--------------------------|
| 0 $+4.4722743877e - 12$  | 25 $+1.2747585372e - 01$ |
| 1 $+4.5330759883e - 10$  | 26 $-1.4575267712e - 01$ |
| 2 $+1.6361363208e - 08$  | 27 $-2.0742960210e - 03$ |
| 3 $+3.3078118645e - 07$  | 28 $+1.4793597636e - 01$ |
| 4 $+4.4209759051e - 06$  | 29 $-1.4774328350e - 01$ |
| 5 $+4.2397026300e - 05$  | 30 $+1.1796927025e - 02$ |
| 6 $+3.0540915187e - 04$  | 31 $+1.3332640115e - 01$ |
| 7 $+1.6962950487e - 03$  | 32 $-1.7007454931e - 01$ |
| 8 $+7.3594297334e - 03$  | 33 $+7.7773350829e - 02$ |
| 9 $+2.4991321128e - 02$  | 34 $+7.1211774770e - 02$ |
| 10 $+6.5751653162e - 02$ | 35 $-1.7744911280e - 01$ |
| 11 $+1.3020522049e - 01$ | 36 $+1.8123906368e - 01$ |
| 12 $+1.8098791979e - 01$ | 37 $-8.9202083580e - 02$ |
| 13 $+1.4223300434e - 01$ | 38 $-4.2511608235e - 02$ |
| 14 $-1.3866208559e - 02$ | 39 $+1.4625253937e - 01$ |
| 15 $-1.5403304773e - 01$ | 40 $-1.7651818615e - 01$ |
| 16 $-8.4071197871e - 02$ | 41 $+1.2472304338e - 01$ |
| 17 $+1.1860830536e - 01$ | 42 $-1.4518508832e - 02$ |
| 18 $+1.1043738934e - 01$ | 43 $-1.1416265678e - 01$ |
| 19 $-1.1275818123e - 01$ | 44 $+2.2244686771e - 01$ |
| 20 $-9.8588406146e - 02$ | 45 $-2.8443590727e - 01$ |
| 21 $+1.3661131209e - 01$ | 46 $+2.9142404039e - 01$ |
| 22 $+4.7921352957e - 02$ | 47 $-2.4969444505e - 01$ |
| 23 $-1.5978542906e - 01$ | 48 $+1.7481927615e - 01$ |
| 24 $+4.6669315777e - 02$ | 49 $-8.5361737846e - 02$ |

$$j = 27: \lambda_{27} = 6.353612e - 12, \quad \ell_{27}(\mathbf{1}) = -5.129468e - 11, \quad \|\hat{v}_{27} - v_{27}\| \leq 1.36e - 147$$

| $k$ $[v_{27}]_k$          | $k$ $[v_{27}]_k$         |
|---------------------------|--------------------------|
| 0 $-1.6678529109e - 12$   | 25 $-1.3914086561e - 01$ |
| 1 $-1.7611878204e - 10$   | 26 $-1.8360931012e - 02$ |
| 2 $-6.6366776908e - 09$   | 27 $+1.5326777694e - 01$ |
| 3 $-1.4043719272e - 07$   | 28 $-1.1293858917e - 01$ |
| 4 $-1.9704205009e - 06$   | 29 $-4.8190248616e - 02$ |
| 5 $-1.9907758705e - 05$   | 30 $+1.6149437371e - 01$ |
| 6 $-1.5174299525e - 04$   | 31 $-1.2448872146e - 01$ |
| 7 $-8.9670145640e - 04$   | 32 $-2.0458946920e - 02$ |
| 8 $-4.1688071647e - 03$   | 33 $+1.4765874501e - 01$ |
| 9 $-1.5318812094e - 02$   | 34 $-1.6083560105e - 01$ |
| 10 $-4.4245056897e - 02$  | 35 $+5.7552969245e - 02$ |
| 11 $-9.8496969381e - 02$  | 36 $+8.6587421919e - 02$ |
| 12 $-1.6143502938e - 01$  | 37 $-1.8056731831e - 01$ |
| 13 $-1.7312769050e - 01$  | 38 $+1.7483665549e - 01$ |
| 14 $-7.0233012670e - 02$  | 39 $-8.0767975887e - 02$ |
| 15 $+9.9709589379e - 02$  | 40 $-4.7080167374e - 02$ |
| 16 $+1.4767149466e - 01$  | 41 $+1.4571968937e - 01$ |
| 17 $-1.80461111286e - 02$ | 42 $-1.7354165307e - 01$ |
| 18 $-1.5369603823e - 01$  | 43 $+1.2309728750e - 01$ |
| 19 $-8.2515820559e - 03$  | 44 $-1.6638504288e - 02$ |
| 20 $+1.5338811466e - 01$  | 45 $-1.0837331381e - 01$ |
| 21 $-1.2525620684e - 02$  | 46 $+2.1509879697e - 01$ |
| 22 $-1.4986993665e - 01$  | 47 $-2.7841363423e - 01$ |
| 23 $+7.0553094429e - 02$  | 48 $+2.8910690930e - 01$ |
| 24 $+1.1467959219e - 01$  | 49 $-2.5218129152e - 01$ |

$$j = 28: \lambda_{28} = -2.418317e - 12, \quad \ell_{28}(\mathbf{1}) = +1.992622e - 11, \quad \|\hat{v}_{28} - v_{28}\| \leq 4.77e - 147$$

| $k$ $[v_{28}]_k$       | $k$ $[v_{28}]_k$       |
|------------------------|------------------------|
| 0 +6.2259699081e - 13  | 25 -6.0018035421e - 03 |
| 1 +6.8384105752e - 11  | 26 +1.4821629920e - 01 |
| 2 +2.6857270091e - 09  | 27 -9.6886382951e - 02 |
| 3 +5.9368284938e - 08  | 28 -7.2821118323e - 02 |
| 4 +8.7249916911e - 07  | 29 +1.5894187035e - 01 |
| 5 +9.2631112781e - 06  | 30 -7.4222462427e - 02 |
| 6 +7.4483590687e - 05  | 31 -8.5429757336e - 02 |
| 7 +4.6656415714e - 04  | 32 +1.6483633940e - 01 |
| 8 +2.3134779413e - 03  | 33 -9.9029974134e - 02 |
| 9 +9.1420496539e - 03  | 34 -4.8030767726e - 02 |
| 10 +2.8728725901e - 02 | 35 +1.5668966930e - 01 |
| 11 +7.0855855226e - 02 | 36 -1.4996216517e - 01 |
| 12 +1.3293070277e - 01 | 37 +3.9232777349e - 02 |
| 13 +1.7640354496e - 01 | 38 +9.9142229485e - 02 |
| 14 +1.3201943807e - 01 | 39 -1.8217965487e - 01 |
| 15 -1.8677965771e - 02 | 40 +1.6875367829e - 01 |
| 16 -1.4886307819e - 01 | 41 -7.3645122644e - 02 |
| 17 -8.3449668866e - 02 | 42 -5.0453843641e - 02 |
| 18 +1.0876293703e - 01 | 43 +1.4472027591e - 01 |
| 19 +1.1491455318e - 01 | 44 -1.7080167652e - 01 |
| 20 -9.4405488010e - 02 | 45 +1.2203473219e - 01 |
| 21 -1.1218513138e - 01 | 46 -1.9277411649e - 02 |
| 22 +1.1271701541e - 01 | 47 -1.0227683431e - 01 |
| 23 +7.9512833976e - 02 | 48 +2.0761718511e - 01 |
| 24 -1.4465920757e - 01 | 49 -2.7229701434e - 01 |

$$j = 29: \lambda_{29} = 9.206274e - 13, \quad \ell_{29}(\mathbf{1}) = -7.736140e - 12, \quad \|\hat{v}_{29} - v_{29}\| \leq 1.67e - 146$$

| $k$ $[v_{29}]_k$       | $k$ $[v_{29}]_k$       |
|------------------------|------------------------|
| 0 -2.3261861851e - 13  | 25 +1.3427571238e - 01 |
| 1 -2.6537502006e - 11  | 26 -1.0197852170e - 01 |
| 2 -1.0845014304e - 09  | 27 -7.1978755758e - 02 |
| 3 -2.4997977908e - 08  | 28 +1.5206988491e - 01 |
| 4 -3.8403281045e - 07  | 29 -4.6136747755e - 02 |
| 5 -4.2744181205e - 06  | 30 -1.1268847280e - 01 |
| 6 -3.6158761725e - 05  | 31 +1.4973968839e - 01 |
| 7 -2.3930616479e - 04  | 32 -3.4776951085e - 02 |
| 8 -1.2604759035e - 03  | 33 -1.1358212855e - 01 |
| 9 -5.3283302399e - 03  | 34 +1.6070737855e - 01 |
| 10 -1.8085705768e - 02 | 35 -7.3365326757e - 02 |
| 11 -4.8873347785e - 02 | 36 -7.1010771848e - 02 |
| 12 -1.0287576572e - 01 | 37 +1.6160646294e - 01 |
| 13 -1.6075886746e - 01 | 38 -1.3833695416e - 01 |
| 14 -1.6496213167e - 01 | 39 +2.2868808827e - 02 |
| 15 -6.1383129450e - 02 | 40 +1.0932184791e - 01 |
| 16 +9.9134249551e - 02 | 41 -1.8270160139e - 01 |
| 17 +1.4253640965e - 01 | 42 +1.6310751503e - 01 |
| 18 -1.2902955864e - 02 | 43 -6.7706038275e - 02 |
| 19 -1.4757770894e - 01 | 44 -5.2815649345e - 02 |
| 20 -2.2110477079e - 02 | 45 +1.4335067125e - 01 |
| 21 +1.4559570653e - 01 | 46 -1.6827874672e - 01 |
| 22 +1.3184876153e - 02 | 47 +1.2144992745e - 01 |
| 23 -1.4796068625e - 01 | 48 -2.2349122311e - 02 |
| 24 +3.2506603709e - 02 | 49 -9.5921615504e - 02 |

$$j = 30: \lambda_{30} = -3.505309e - 13, \quad \ell_{30}(\mathbf{1}) = +3.001843e - 12, \quad \|\hat{v}_{30} - v_{30}\| \leq 5.87e - 146$$

| $k$ $[v_{30}]_k$       | $k$ $[v_{30}]_k$       |
|------------------------|------------------------|
| 0 +8.6984479598e - 14  | 25 -1.2243155723e - 01 |
| 1 +1.0292879842e - 11  | 26 -4.8273218736e - 02 |
| 2 +4.3704308320e - 10  | 27 +1.4777487381e - 01 |
| 3 +1.0487295291e - 08  | 28 -4.2716704650e - 02 |
| 4 +1.6810211529e - 07  | 29 -1.1789356976e - 01 |
| 5 +1.9573959706e - 06  | 30 +1.3417651497e - 01 |
| 6 +1.7377221324e - 05  | 31 +4.0423095824e - 03 |
| 7 +1.2115557786e - 04  | 32 -1.3775157911e - 01 |
| 8 +6.7546704760e - 04  | 33 +1.3067010487e - 01 |
| 9 +3.0407254436e - 03  | 34 +2.2192866315e - 03 |
| 10 +1.1080686297e - 02 | 35 -1.3341034753e - 01 |
| 11 +3.2521637753e - 02 | 36 +1.5143223821e - 01 |
| 12 +7.5706318333e - 02 | 37 -4.8746625822e - 02 |
| 13 +1.3520655160e - 01 | 38 -8.9768754605e - 02 |
| 14 +1.7177623454e - 01 | 39 +1.6341122499e - 01 |
| 15 +1.2231192352e - 01 | 40 -1.2656961339e - 01 |
| 16 -2.3539333508e - 02 | 41 +8.4075902816e - 03 |
| 17 -1.4448074617e - 01 | 42 +1.1751730115e - 01 |
| 18 -8.2011766906e - 02 | 43 -1.8244904376e - 01 |
| 19 +1.0073524227e - 01 | 44 +1.5796180253e - 01 |
| 20 +1.1721629829e - 01 | 45 -6.2829145363e - 02 |
| 21 -7.8466998224e - 02 | 46 -5.4315944377e - 02 |
| 22 -1.2036615510e - 01 | 47 +1.4168193497e - 01 |
| 23 +8.9452369407e - 02 | 48 -1.6594821506e - 01 |
| 24 +1.0107656000e - 01 | 49 +1.2126670027e - 01 |

$$j = 31: \lambda_{31} = 1.334857e - 13, \quad \ell_{31}(\mathbf{1}) = -1.164209e - 12, \quad \|\hat{v}_{31} - v_{31}\| \leq 2.06e - 145$$

| $k$ $[v_{31}]_k$       | $k$ $[v_{31}]_k$       |
|------------------------|------------------------|
| 0 -3.2551689036e - 14  | 25 -2.6815405982e - 04 |
| 1 -3.9902556917e - 12  | 26 +1.4079745609e - 01 |
| 2 -1.7579466350e - 10  | 27 -6.2107340380e - 02 |
| 3 -4.3847645928e - 09  | 28 -1.0748721849e - 01 |
| 4 -7.3208344837e - 08  | 29 +1.2877969136e - 01 |
| 5 -8.9006676337e - 07  | 30 +1.7251798635e - 02 |
| 6 -8.2741193456e - 06  | 31 -1.4213086812e - 01 |
| 7 -6.0613784846e - 05  | 32 +1.0289821074e - 01 |
| 8 -3.5656926002e - 04  | 33 +4.8321844372e - 02 |
| 9 -1.7026668396e - 03  | 34 -1.4976116921e - 01 |
| 10 -6.6274090744e - 03 | 35 +1.0587247171e - 01 |
| 11 -2.0976241578e - 02 | 36 +3.5055294448e - 02 |
| 12 -5.3412826991e - 02 | 37 -1.4610449742e - 01 |
| 13 -1.0686260848e - 01 | 38 +1.3885910576e - 01 |
| 14 -1.5976294738e - 01 | 39 -2.5894840807e - 02 |
| 15 -1.5705825171e - 01 | 40 -1.0479712692e - 01 |
| 16 -5.2905162473e - 02 | 41 +1.6292191318e - 01 |
| 17 +9.9056155097e - 02 | 42 -1.1506894368e - 01 |
| 18 +1.3767568660e - 01 | 43 -4.2646883278e - 03 |
| 19 -9.3799628084e - 03 | 44 +1.2406365993e - 01 |
| 20 -1.4181232547e - 01 | 45 -1.8166040430e - 01 |
| 21 -3.2737367752e - 02 | 46 +1.5334387962e - 01 |
| 22 +1.3689481614e - 01 | 47 -5.8901876835e - 02 |
| 23 +3.3597207357e - 02 | 48 -5.5078324280e - 02 |
| 24 -1.4080436104e - 01 | 49 +1.3976616736e - 01 |

$$j = 32: \lambda_{32} = -5.083983e - 14, \quad \ell_{32}(\mathbf{1}) = +4.513023e - 13, \quad \|\hat{v}_{32} - v_{32}\| \leq 7.24e - 145$$

| $k$ | $[v_{32}]_k$        | $k$ | $[v_{32}]_k$        |
|-----|---------------------|-----|---------------------|
| 0   | +1.2190371234e - 14 | 25  | +1.1468767512e - 01 |
| 1   | +1.5461977209e - 12 | 26  | -9.7410119834e - 02 |
| 2   | +7.0587793293e - 11 | 27  | -7.9609475009e - 02 |
| 3   | +1.8274979338e - 09 | 28  | +1.3353238022e - 01 |
| 4   | +3.1731580711e - 08 | 29  | +7.0802258777e - 03 |
| 5   | +4.0210499281e - 07 | 30  | -1.3789546239e - 01 |
| 6   | +3.9062067681e - 06 | 31  | +8.9766205103e - 02 |
| 7   | +2.9996201518e - 05 | 32  | +6.8336657948e - 02 |
| 8   | +1.8566522560e - 04 | 33  | -1.4733874950e - 01 |
| 9   | +9.3720451230e - 04 | 34  | +6.5244870876e - 02 |
| 10  | +3.8794344098e - 03 | 35  | +8.4185461974e - 02 |
| 11  | +1.3163326358e - 02 | 36  | -1.5123737160e - 01 |
| 12  | +3.6349063897e - 02 | 37  | +7.8476664021e - 02 |
| 13  | +8.0305009901e - 02 | 38  | +6.3016087016e - 02 |
| 14  | +1.3706333176e - 01 | 39  | -1.5296265512e - 01 |
| 15  | +1.6708330197e - 01 | 40  | +1.2439363748e - 01 |
| 16  | +1.1302079563e - 01 | 41  | -5.1684763526e - 03 |
| 17  | -2.8388389819e - 02 | 42  | -1.1661980231e - 01 |
| 18  | -1.4070150506e - 01 | 43  | +1.6079085391e - 01 |
| 19  | -7.9988491598e - 02 | 44  | -1.0409865698e - 01 |
| 20  | +9.4233819814e - 02 | 45  | -1.5291027077e - 02 |
| 21  | +1.1804189565e - 01 | 46  | +1.2924357379e - 01 |
| 22  | -6.4837517636e - 02 | 47  | -1.8051426773e - 01 |
| 23  | -1.2472402947e - 01 | 48  | +1.4925690835e - 01 |
| 24  | +6.7999969452e - 02 | 49  | -5.5821877285e - 02 |

$$j = 33: \lambda_{33} = 1.936554e - 14, \quad \ell_{33}(\mathbf{1}) = -1.748680e - 13, \quad \|\hat{v}_{33} - v_{33}\| \leq 2.54e - 144$$

| $k$ | $[v_{33}]_k$        | $k$ | $[v_{33}]_k$        |
|-----|---------------------|-----|---------------------|
| 0   | -4.5682661250e - 15 | 25  | -1.3070298261e - 01 |
| 1   | -5.9888311557e - 13 | 26  | -2.7300842068e - 02 |
| 2   | -2.8297346895e - 11 | 27  | +1.3814284443e - 01 |
| 3   | -7.5943113848e - 10 | 28  | -2.4352943452e - 02 |
| 4   | -1.3693379068e - 08 | 29  | -1.2674730402e - 01 |
| 5   | -1.8056546581e - 07 | 30  | +9.4071284767e - 02 |
| 6   | -1.8296218539e - 06 | 31  | +6.7459170590e - 02 |
| 7   | -1.4696162335e - 05 | 32  | -1.4153333607e - 01 |
| 8   | -9.5469604442e - 05 | 33  | +4.2112309270e - 02 |
| 9   | -5.0788336260e - 04 | 34  | +1.0614830536e - 01 |
| 10  | -2.2272251606e - 03 | 35  | -1.3788147235e - 01 |
| 11  | -8.0613561217e - 03 | 36  | +2.6365860383e - 02 |
| 12  | -2.3972247354e - 02 | 37  | +1.1098472765e - 01 |
| 13  | -5.7850304490e - 02 | 38  | -1.4478723394e - 01 |
| 14  | -1.1047635963e - 01 | 39  | +5.0691297731e - 02 |
| 15  | -1.5846280255e - 01 | 40  | +8.6016655521e - 02 |
| 16  | -1.4935575953e - 01 | 41  | -1.5522026481e - 01 |
| 17  | -4.4759732186e - 02 | 42  | +1.0906716958e - 01 |
| 18  | +9.9327135207e - 02 | 43  | +1.3312093394e - 02 |
| 19  | +1.3305272324e - 01 | 44  | -1.2574175373e - 01 |
| 20  | -7.1205836530e - 03 | 45  | +1.5752926423e - 01 |
| 21  | -1.3651620782e - 01 | 46  | -9.3819263091e - 02 |
| 22  | -4.0824698690e - 02 | 47  | -2.4824369439e - 02 |
| 23  | +1.2805709556e - 01 | 48  | +1.3329289619e - 01 |
| 24  | +4.9552210686e - 02 | 49  | -1.7914320566e - 01 |

$$j = 34: \lambda_{34} = -7.377470e - 15, \quad \ell_{34}(\mathbf{1}) = +6.772837e - 14, \quad \|\hat{v}_{34} - v_{34}\| \leq 8.93e - 144$$

| $k$ | $[v_{34}]_k$        | $k$ | $[v_{34}]_k$        |
|-----|---------------------|-----|---------------------|
| 0   | +1.7130036569e - 15 | 25  | +4.8851903818e - 02 |
| 1   | +2.3186916316e - 13 | 26  | +1.2227745760e - 01 |
| 2   | +1.1326584919e - 11 | 27  | -7.2303365394e - 02 |
| 3   | +3.1472023984e - 10 | 28  | -1.0100464484e - 01 |
| 4   | +5.8850036774e - 09 | 29  | +1.1137789277e - 01 |
| 5   | +8.0629104028e - 08 | 30  | +4.8057756087e - 02 |
| 6   | +8.5072584600e - 07 | 31  | -1.3809850749e - 01 |
| 7   | +7.1337245744e - 06 | 32  | +3.9483896248e - 02 |
| 8   | +4.8527262213e - 05 | 33  | +1.1017765310e - 01 |
| 9   | +2.7133120989e - 04 | 34  | -1.2470640455e - 01 |
| 10  | +1.2563626401e - 03 | 35  | -5.7119457905e - 03 |
| 11  | +4.8300136633e - 03 | 36  | +1.2983834991e - 01 |
| 12  | +1.5378220895e - 02 | 37  | -1.1833357861e - 01 |
| 13  | +4.0192362429e - 02 | 38  | -1.0343368195e - 02 |
| 14  | +8.4653159777e - 02 | 39  | +1.2918197396e - 01 |
| 15  | +1.3852568068e - 01 | 40  | -1.3276285582e - 01 |
| 16  | +1.6230918987e - 01 | 41  | +2.3973551623e - 02 |
| 17  | +1.0407953796e - 01 | 42  | +1.0434016873e - 01 |
| 18  | -3.3180194072e - 02 | 43  | -1.5397051868e - 01 |
| 19  | -1.3738167204e - 01 | 44  | +9.3611274016e - 02 |
| 20  | -7.7536619090e - 02 | 45  | +2.9576246814e - 02 |
| 21  | +8.9008639878e - 02 | 46  | -1.3262367092e - 01 |
| 22  | +1.1786997565e - 01 | 47  | +1.5353207078e - 01 |
| 23  | -5.3307134444e - 02 | 48  | -8.4318966735e - 02 |
| 24  | -1.2643115352e - 01 | 49  | -3.3016114441e - 02 |

$$j = 35: \lambda_{35} = 2.810825e - 15, \quad \ell_{35}(\mathbf{1}) = -2.622160e - 14, \quad \|\hat{v}_{35} - v_{35}\| \leq 3.14e - 143$$

| $k$ | $[v_{35}]_k$        | $k$ | $[v_{35}]_k$        |
|-----|---------------------|-----|---------------------|
| 0   | -6.4271834664e - 16 | 25  | +6.1857866203e - 02 |
| 1   | -8.9738328287e - 14 | 26  | -1.1919671935e - 01 |
| 2   | -4.5272053656e - 12 | 27  | -4.8893203425e - 02 |
| 3   | -1.3008929878e - 10 | 28  | +1.2951584007e - 01 |
| 4   | -2.5195132248e - 09 | 29  | +8.7874110836e - 03 |
| 5   | -3.5815883731e - 08 | 30  | -1.3296492560e - 01 |
| 6   | -3.9288275021e - 07 | 31  | +5.5601484445e - 02 |
| 7   | -3.4331917842e - 06 | 32  | +1.0159238163e - 01 |
| 8   | -2.4404978823e - 05 | 33  | -1.2036066427e - 01 |
| 9   | -1.4306979482e - 04 | 34  | -1.6407079599e - 02 |
| 10  | -6.9741931217e - 04 | 35  | +1.3300897311e - 01 |
| 11  | -2.8372954761e - 03 | 36  | -9.4704442384e - 02 |
| 12  | -9.6249056762e - 03 | 37  | -4.8319773707e - 02 |
| 13  | -2.7056918783e - 02 | 38  | +1.4061994016e - 01 |
| 14  | -6.2174097931e - 02 | 39  | -9.2730031538e - 02 |
| 15  | -1.1373223329e - 01 | 40  | -4.2901999947e - 02 |
| 16  | -1.5687190403e - 01 | 41  | +1.3981347906e - 01 |
| 17  | -1.4181038059e - 01 | 42  | -1.1712549250e - 01 |
| 18  | -3.6916985701e - 02 | 43  | -7.9149923439e - 04 |
| 19  | +9.9835329097e - 02 | 44  | +1.1846115144e - 01 |
| 20  | +1.2862863051e - 01 | 45  | -1.5013740494e - 01 |
| 21  | -5.8572804820e - 03 | 46  | +7.8526126672e - 02 |
| 22  | -1.3172728187e - 01 | 47  | +4.3742103579e - 02 |
| 23  | -4.6916020212e - 02 | 48  | -1.3767160339e - 01 |
| 24  | +1.1953227248e - 01 | 49  | +1.4910044462e - 01 |

$$j = 36: \lambda_{36} = -1.071039e - 15, \quad \ell_{36}(\mathbf{1}) = +1.014812e - 14, \quad \|\hat{v}_{36} - v_{36}\| \leq 1.10e - 142$$

| $k$ $[v_{36}]_k$         | $k$ $[v_{36}]_k$         |
|--------------------------|--------------------------|
| 0 $+2.4128104872e - 16$  | 25 $-1.2634011528e - 01$ |
| 1 $+3.4718129081e - 14$  | 26 $+3.2119837843e - 02$ |
| 2 $+1.8070762352e - 12$  | 27 $+1.2545516926e - 01$ |
| 3 $+5.3642366992e - 11$  | 28 $-4.8652278268e - 02$ |
| 4 $+1.0747954517e - 09$  | 29 $-1.1411387124e - 01$ |
| 5 $+1.5831960577e - 08$  | 30 $+8.5671057785e - 02$ |
| 6 $+1.8029399942e - 07$  | 31 $+7.8807089214e - 02$ |
| 7 $+1.6391244535e - 06$  | 32 $-1.2448189618e - 01$ |
| 8 $+1.2153036565e - 05$  | 33 $-7.9067922250e - 03$ |
| 9 $+7.4533717198e - 05$  | 34 $+1.2951440797e - 01$ |
| 10 $+3.8149057123e - 04$ | 35 $-8.3920420310e - 02$ |
| 11 $+1.6370338395e - 03$ | 36 $-6.4613654270e - 02$ |
| 12 $+5.8920358818e - 03$ | 37 $+1.3774076823e - 01$ |
| 13 $+1.7713879526e - 02$ | 38 $-5.8059823587e - 02$ |
| 14 $+4.4034713263e - 02$ | 39 $-8.2881847408e - 02$ |
| 15 $+8.8751377256e - 02$ | 40 $+1.4068666768e - 01$ |
| 16 $+1.3961393726e - 01$ | 41 $-6.4286150400e - 02$ |
| 17 $+1.5744365866e - 01$ | 42 $-7.0366215039e - 02$ |
| 18 $+9.5438458637e - 02$ | 43 $+1.4414036016e - 01$ |
| 19 $-3.7881174041e - 02$ | 44 $-9.9423605015e - 02$ |
| 20 $-1.3440817913e - 01$ | 45 $-2.3132758737e - 02$ |
| 21 $-7.4764400376e - 02$ | 46 $+1.2893184312e - 01$ |
| 22 $+8.4849390899e - 02$ | 47 $-1.4447723807e - 01$ |
| 23 $+1.1702823465e - 01$ | 48 $+6.4138142792e - 02$ |
| 24 $-4.3632146860e - 02$ | 49 $+5.5975488227e - 02$ |

$$j = 37: \lambda_{37} = 4.081489e - 16, \quad \ell_{37}(\mathbf{1}) = -3.926074e - 15, \quad \|\hat{v}_{37} - v_{37}\| \leq 3.87e - 142$$

| $k$ $[v_{37}]_k$         | $k$ $[v_{37}]_k$         |
|--------------------------|--------------------------|
| 0 $-9.0625781893e - 17$  | 25 $+1.1156667145e - 01$ |
| 1 $-1.3427233587e - 14$  | 26 $+7.1227933709e - 02$ |
| 2 $-7.2039669012e - 13$  | 27 $-1.0728792952e - 01$ |
| 3 $-2.2069190830e - 11$  | 28 $-6.5676517275e - 02$ |
| 4 $-4.5695138276e - 10$  | 29 $+1.1732922822e - 01$ |
| 5 $-6.9663167620e - 09$  | 30 $+3.6375666470e - 02$ |
| 6 $-8.2247865564e - 08$  | 31 $-1.2959879342e - 01$ |
| 7 $-7.7677177242e - 07$  | 32 $+1.8395916106e - 02$ |
| 8 $-5.9966565317e - 06$  | 33 $+1.2033234206e - 01$ |
| 9 $-3.8397807889e - 05$  | 34 $-8.7580013585e - 02$ |
| 10 $-2.0587017355e - 04$ | 35 $-6.3839981814e - 02$ |
| 11 $-9.2913550260e - 04$ | 36 $+1.3291146099e - 01$ |
| 12 $-3.5352925458e - 03$ | 37 $-3.8861518942e - 02$ |
| 13 $-1.1312333160e - 02$ | 38 $-1.0056695600e - 01$ |
| 14 $-3.0214569309e - 02$ | 39 $+1.2807301715e - 01$ |
| 15 $-6.6373657346e - 02$ | 40 $-1.9854834349e - 02$ |
| 16 $-1.1664270574e - 01$ | 41 $-1.0841751495e - 01$ |
| 17 $-1.5500233648e - 01$ | 42 $+1.3251664643e - 01$ |
| 18 $-1.3438961590e - 01$ | 43 $-3.5375303043e - 02$ |
| 19 $-2.9354365982e - 02$ | 44 $-9.2496995799e - 02$ |
| 20 $+1.0049482557e - 01$ | 45 $+1.4343897622e - 01$ |
| 21 $+1.2436604033e - 01$ | 46 $-8.0827298570e - 02$ |
| 22 $-5.3867097930e - 03$ | 47 $-4.2865694693e - 02$ |
| 23 $-1.2744019296e - 01$ | 48 $+1.3631291547e - 01$ |
| 24 $-5.1433916338e - 02$ | 49 $-1.3759408215e - 01$ |

$$j = 38: \lambda_{38} = -1.555505e - 16, \quad \ell_{38}(\mathbf{1}) = +1.518400e - 15, \quad \|\hat{v}_{38} - v_{38}\| \leq 1.36e - 141$$

| $k$ $[v_{38}]_k$         | $k$ $[v_{38}]_k$         |
|--------------------------|--------------------------|
| 0 $+3.4055987834e - 17$  | 25 $-3.5571778740e - 02$ |
| 1 $+5.1913046270e - 15$  | 26 $-1.2506302220e - 01$ |
| 2 $+2.8684475539e - 13$  | 27 $+1.7710264901e - 02$ |
| 3 $+9.0601252115e - 12$  | 28 $+1.2549950206e - 01$ |
| 4 $+1.9365838794e - 10$  | 29 $-2.7241196846e - 02$ |
| 5 $+3.0521304903e - 09$  | 30 $-1.2068560435e - 01$ |
| 6 $+3.7312628357e - 08$  | 31 $+5.9339907804e - 02$ |
| 7 $+3.6555648781e - 07$  | 32 $+9.9741204210e - 02$ |
| 8 $+2.9337544704e - 06$  | 33 $-1.0248794550e - 01$ |
| 9 $+1.9577498203e - 05$  | 34 $-4.7563988730e - 02$ |
| 10 $+1.0971610118e - 04$ | 35 $+1.3005872357e - 01$ |
| 11 $+5.1945917052e - 04$ | 36 $-3.6710592099e - 02$ |
| 12 $+2.0828286551e - 03$ | 37 $-1.0390018225e - 01$ |
| 13 $+7.0643540577e - 03$ | 38 $+1.1694132567e - 01$ |
| 14 $+2.0159050116e - 02$ | 39 $+6.8612641965e - 03$ |
| 15 $+4.7860739203e - 02$ | 40 $-1.2297939347e - 01$ |
| 16 $+9.2599783044e - 02$ | 41 $+1.0821856135e - 01$ |
| 17 $+1.4034529520e - 01$ | 42 $+1.6371502818e - 02$ |
| 18 $+1.5248052519e - 01$ | 43 $-1.2514305622e - 01$ |
| 19 $+8.7060332743e - 02$ | 44 $+1.1847366201e - 01$ |
| 20 $-4.2465557250e - 02$ | 45 $-7.6282779317e - 03$ |
| 21 $-1.3169122088e - 01$ | 46 $-1.0949931610e - 01$ |
| 22 $-7.1747772458e - 02$ | 47 $+1.3888681839e - 01$ |
| 23 $+8.1580526799e - 02$ | 48 $-6.2185574266e - 02$ |
| 24 $+1.1574130539e - 01$ | 49 $-5.9995246138e - 02$ |

$$j = 39: \lambda_{39} = 5.928725e - 17, \quad \ell_{39}(\mathbf{1}) = -5.870515e - 16, \quad \|\hat{v}_{39} - v_{39}\| \leq 4.79e - 141$$

| $k$ $[v_{39}]_k$         | $k$ $[v_{39}]_k$         |
|--------------------------|--------------------------|
| 0 $-1.2803730896e - 17$  | 25 $-5.4705982137e - 02$ |
| 1 $-2.0064736299e - 15$  | 26 $+1.0428071693e - 01$ |
| 2 $-1.1408552621e - 13$  | 27 $+7.8263106326e - 02$ |
| 3 $-3.7119631555e - 12$  | 28 $-9.5603632037e - 02$ |
| 4 $-8.1828450951e - 11$  | 29 $-7.8386898078e - 02$ |
| 5 $-1.3318192165e - 09$  | 30 $+1.0331808153e - 01$ |
| 6 $-1.6839242970e - 08$  | 31 $+5.8371667849e - 02$ |
| 7 $-1.7091750112e - 07$  | 32 $-1.1971396409e - 01$ |
| 8 $-1.4238793287e - 06$  | 33 $-1.4705086670e - 02$ |
| 9 $-9.8858943099e - 06$  | 34 $+1.2617912603e - 01$ |
| 10 $-5.7797716042e - 05$ | 35 $-5.0409664003e - 02$ |
| 11 $-2.8640756212e - 04$ | 36 $-9.6634568453e - 02$ |
| 12 $-1.2067547524e - 03$ | 37 $+1.1329940199e - 01$ |
| 13 $-4.3229658195e - 03$ | 38 $+1.5827316135e - 02$ |
| 14 $-1.3117538591e - 02$ | 39 $-1.2549658592e - 01$ |
| 15 $-3.3430435912e - 02$ | 40 $+8.8072185884e - 02$ |
| 16 $-7.0439319487e - 02$ | 41 $+4.7876162550e - 02$ |
| 17 $-1.1921819808e - 01$ | 42 $-1.3265463010e - 01$ |
| 18 $-1.5286526226e - 01$ | 43 $+8.2105119932e - 02$ |
| 19 $-1.2706979463e - 01$ | 44 $+4.8429665570e - 02$ |
| 20 $-2.2054951850e - 02$ | 45 $-1.3396065920e - 01$ |
| 21 $+1.0123864035e - 01$ | 46 $+1.0061122118e - 01$ |
| 22 $+1.2023084367e - 01$ | 47 $+1.7924530721e - 02$ |
| 23 $-5.5523841307e - 03$ | 48 $-1.2183172515e - 01$ |
| 24 $-1.2362646341e - 01$ | 49 $+1.3150976816e - 01$ |

$$j = 40: \lambda_{40} = -2.259881e - 17, \quad \ell_{40}(\mathbf{1}) = +2.269005e - 16, \quad \|\hat{v}_{40} - v_{40}\| \leq 1.68e - 140$$

| $k$ $[v_{40}]_k$         | $k$ $[v_{40}]_k$         |
|--------------------------|--------------------------|
| 0 $+4.8158179342e - 18$  | 25 $+1.1416288121e - 01$ |
| 1 $+7.7528976862e - 16$  | 26 $-2.8904331793e - 02$ |
| 2 $+4.5326146309e - 14$  | 27 $-1.2303565459e - 01$ |
| 3 $+1.5178988339e - 12$  | 28 $+5.4309868025e - 03$ |
| 4 $+3.4478382631e - 11$  | 29 $+1.2339223578e - 01$ |
| 5 $+5.7893664767e - 10$  | 30 $-8.3756607715e - 03$ |
| 6 $+7.5623920114e - 09$  | 31 $-1.2232034702e - 01$ |
| 7 $+7.9426070713e - 08$  | 32 $+3.4211008406e - 02$ |
| 8 $+6.8592736401e - 07$  | 33 $+1.1213394301e - 01$ |
| 9 $+4.9472239700e - 06$  | 34 $-7.6395078570e - 02$ |
| 10 $+3.0120825200e - 05$ | 35 $-7.7590077310e - 02$ |
| 11 $+1.5589326944e - 04$ | 36 $+1.1694065737e - 01$ |
| 12 $+6.8849888492e - 04$ | 37 $+8.5588486092e - 03$ |
| 13 $+2.5968895700e - 03$ | 38 $-1.2250833981e - 01$ |
| 14 $+8.3451919930e - 03$ | 39 $+7.8944722462e - 02$ |
| 15 $+2.2702694086e - 02$ | 40 $+6.1570367948e - 02$ |
| 16 $+5.1656232029e - 02$ | 41 $-1.2980394545e - 01$ |
| 17 $+9.6198138048e - 02$ | 42 $+5.2430238553e - 02$ |
| 18 $+1.4073463568e - 01$ | 43 $+8.1142089296e - 02$ |
| 19 $+1.4741676145e - 01$ | 44 $-1.3151892658e - 01$ |
| 20 $+7.8917330186e - 02$ | 45 $+5.3002895281e - 02$ |
| 21 $-4.6913057891e - 02$ | 46 $+7.5186059860e - 02$ |
| 22 $-1.2915888361e - 01$ | 47 $-1.3609575367e - 01$ |
| 23 $-6.8540887732e - 02$ | 48 $+8.0603144415e - 02$ |
| 24 $+7.9055876811e - 02$ | 49 $+4.0709434272e - 02$ |

$$j = 41: \lambda_{41} = 8.614744e - 18, \quad \ell_{41}(\mathbf{1}) = -8.767390e - 17, \quad \|\hat{v}_{41} - v_{41}\| \leq 5.92e - 140$$

| $k$ $[v_{41}]_k$         | $k$ $[v_{41}]_k$         |
|--------------------------|--------------------------|
| 0 $-1.8121077708e - 18$  | 25 $-1.2024628014e - 01$ |
| 1 $-2.9948459538e - 16$  | 26 $-5.6986055656e - 02$ |
| 2 $-1.7989777380e - 14$  | 27 $+9.7717778387e - 02$ |
| 3 $-6.1957788797e - 13$  | 28 $+8.3455580036e - 02$ |
| 4 $-1.4488747047e - 11$  | 29 $-8.4516930151e - 02$ |
| 5 $-2.5075703089e - 10$  | 30 $-8.7744702462e - 02$ |
| 6 $-3.3805578679e - 09$  | 31 $+8.8676264693e - 02$ |
| 7 $-3.6697962435e - 08$  | 32 $+7.5217614033e - 02$ |
| 8 $-3.2812434047e - 07$  | 33 $-1.0579177374e - 01$ |
| 9 $-2.4549642085e - 06$  | 34 $-4.2386403130e - 02$ |
| 10 $-1.5540116643e - 05$ | 35 $+1.2217515511e - 01$ |
| 11 $-8.3845216439e - 05$ | 36 $-1.3868062831e - 02$ |
| 12 $-3.8727161271e - 04$ | 37 $-1.1480090200e - 01$ |
| 13 $-1.5337474767e - 03$ | 38 $+8.2130681757e - 02$ |
| 14 $-5.2014537978e - 03$ | 39 $+6.0848334221e - 02$ |
| 15 $-1.5034106638e - 02$ | 40 $-1.2564586897e - 01$ |
| 16 $-3.6690528965e - 02$ | 41 $+3.6079847711e - 02$ |
| 17 $-7.4362146081e - 02$ | 42 $+9.5876130279e - 02$ |
| 18 $-1.2146759467e - 01$ | 43 $-1.2000809351e - 01$ |
| 19 $-1.5047124589e - 01$ | 44 $+1.5010095318e - 02$ |
| 20 $-1.1983397666e - 01$ | 45 $+1.0542459452e - 01$ |
| 21 $-1.5006209557e - 02$ | 46 $-1.2193595304e - 01$ |
| 22 $+1.0201386270e - 01$ | 47 $+2.3417266541e - 02$ |
| 23 $+1.1619282771e - 01$ | 48 $+9.6267960414e - 02$ |
| 24 $-6.2323517485e - 03$ | 49 $-1.3285976766e - 01$ |

$$j = 42: \lambda_{42} = -3.284201e - 18, \quad \ell_{42}(\mathbf{1}) = +3.386778e - 17, \quad \|\hat{v}_{42} - v_{42}\| \leq 2.08e - 139$$

| $k$ $[v_{42}]_k$       | $k$ $[v_{42}]_k$       |
|------------------------|------------------------|
| 0 +6.8213316410e - 19  | 25 +7.7153596724e - 02 |
| 1 +1.1565662134e - 16  | 26 +1.1239760588e - 01 |
| 2 +7.1331906001e - 15  | 27 -2.3433251882e - 02 |
| 3 +2.5246644037e - 13  | 28 -1.2056555095e - 01 |
| 4 +6.0732012723e - 12  | 29 -4.9485371598e - 03 |
| 5 +1.0824220185e - 10  | 30 +1.1987038018e - 01 |
| 6 +1.5046046698e - 09  | 31 +7.9241056653e - 03 |
| 7 +1.6864254281e - 08  | 32 -1.2037194219e - 01 |
| 8 +1.5593217901e - 07  | 33 +1.1310626144e - 02 |
| 9 +1.2086313156e - 06  | 34 +1.1756782132e - 01 |
| 10 +7.9424832946e - 06 | 35 -4.9286824130e - 02 |
| 11 +4.4595633210e - 05 | 36 -9.7923549796e - 02 |
| 12 +2.1498385135e - 04 | 37 +9.5150954294e - 02 |
| 13 +8.9179011220e - 04 | 38 +4.6949830010e - 02 |
| 14 +3.1819052345e - 03 | 39 -1.2324865755e - 01 |
| 15 +9.7322157544e - 03 | 40 +3.4307252973e - 02 |
| 16 +2.5333962450e - 02 | 41 +9.8642711878e - 02 |
| 17 +5.5407953031e - 02 | 42 -1.1036462612e - 01 |
| 18 +9.9545961502e - 02 | 43 -7.7855754760e - 03 |
| 19 +1.4079513827e - 01 | 44 +1.1714816340e - 01 |
| 20 +1.4225183610e - 01 | 45 -1.0001944433e - 01 |
| 21 +7.0988802181e - 02 | 46 -2.0555494266e - 02 |
| 22 -5.1207344196e - 02 | 47 +1.2073984798e - 01 |
| 23 -1.2675318702e - 01 | 48 -1.0627392306e - 01 |
| 24 -6.5183047602e - 02 | 49 -4.8724871601e - 03 |

$$j = 43: \lambda_{43} = 1.252120e - 18, \quad \ell_{43}(\mathbf{1}) = -1.307948e - 17, \quad \|\hat{v}_{43} - v_{43}\| \leq 7.32e - 139$$

| $k$ $[v_{43}]_k$       | $k$ $[v_{43}]_k$       |
|------------------------|------------------------|
| 0 -2.5687208536e - 19  | 25 -7.3303783665e - 03 |
| 1 -4.4653697179e - 17  | 26 -1.1725529860e - 01 |
| 2 -2.8258139309e - 15  | 27 -5.8471106571e - 02 |
| 3 -1.0270787030e - 13  | 28 +9.1875226577e - 02 |
| 4 -2.5395931000e - 12  | 29 +8.7201878519e - 02 |
| 5 -4.6573604414e - 11  | 30 -7.4232050016e - 02 |
| 6 -6.6690552994e - 10  | 31 -9.4400039244e - 02 |
| 7 -7.7102842113e - 09  | 32 +7.4191444137e - 02 |
| 8 -7.3643696655e - 08  | 33 +8.7571218432e - 02 |
| 9 -5.9062756410e - 07  | 34 -8.9714563310e - 02 |
| 10 -4.0237293257e - 06 | 35 -6.4328756730e - 02 |
| 11 -2.3474033631e - 05 | 36 +1.1125507003e - 01 |
| 12 -1.1788891638e - 04 | 37 +1.8951252861e - 02 |
| 13 -5.1107936888e - 04 | 38 -1.2025107333e - 01 |
| 14 -1.9133192783e - 03 | 39 +4.6140945706e - 02 |
| 15 -6.1713299795e - 03 | 40 +9.2402012144e - 02 |
| 16 -1.7055351315e - 02 | 41 -1.0727480272e - 01 |
| 17 -3.9981516638e - 02 | 42 -1.5405798512e - 02 |
| 18 -7.8133817347e - 02 | 43 +1.1913292545e - 01 |
| 19 -1.2339864144e - 01 | 44 -8.2486919636e - 02 |
| 20 -1.4783048391e - 01 | 45 -4.7334541795e - 02 |
| 21 -1.1267042868e - 01 | 46 +1.2587379236e - 01 |
| 22 -8.1990408253e - 03 | 47 -7.3661960024e - 02 |
| 23 +1.0277823430e - 01 | 48 -5.1915464984e - 02 |
| 24 +1.1222576235e - 01 | 49 +1.2787631400e - 01 |

$$j = 44: \lambda_{44} = -4.774076e - 19, \quad \ell_{44}(\mathbf{1}) = +5.049939e - 18, \quad \|\hat{v}_{44} - v_{44}\| \leq 2.57e - 138$$

| $k$ $[v_{44}]_k$         | $k$ $[v_{44}]_k$         |
|--------------------------|--------------------------|
| 0 $+9.6765225049e - 20$  | 25 $-6.1703344125e - 02$ |
| 1 $+1.7236148126e - 17$  | 26 $+7.5771801027e - 02$ |
| 2 $+1.1184694903e - 15$  | 27 $+1.1051604318e - 01$ |
| 3 $+4.1718720253e - 14$  | 28 $-1.8987973470e - 02$ |
| 4 $+1.0595528951e - 12$  | 29 $-1.1786762446e - 01$ |
| 5 $+1.9978139206e - 11$  | 30 $-1.3663629541e - 02$ |
| 6 $+2.9444820474e - 10$  | 31 $+1.1547719083e - 01$ |
| 7 $+3.5081046822e - 09$  | 32 $+2.1797681456e - 02$ |
| 8 $+3.4577159451e - 08$  | 33 $-1.1593244631e - 01$ |
| 9 $+2.8661073314e - 07$  | 34 $-8.8796220830e - 03$ |
| 10 $+2.0216378896e - 06$ | 35 $+1.1761648314e - 01$ |
| 11 $+1.2236323699e - 05$ | 36 $-2.3206798360e - 02$ |
| 12 $+6.3910701110e - 05$ | 37 $-1.0953099413e - 01$ |
| 13 $+2.8898825552e - 04$ | 38 $+6.8881229825e - 02$ |
| 14 $+1.1324084682e - 03$ | 39 $+7.6192772508e - 02$ |
| 15 $+3.8401243373e - 03$ | 40 $-1.1052704182e - 01$ |
| 16 $+1.1222591137e - 02$ | 41 $-9.1013626576e - 03$ |
| 17 $+2.8042174968e - 02$ | 42 $+1.1655081860e - 01$ |
| 18 $+5.9103487027e - 02$ | 43 $-7.4654222673e - 02$ |
| 19 $+1.0264263590e - 01$ | 44 $-5.9001693870e - 02$ |
| 20 $+1.4053873591e - 01$ | 45 $+1.2304498805e - 01$ |
| 21 $+1.3698722329e - 01$ | 46 $-4.7791689677e - 02$ |
| 22 $+6.3259655630e - 02$ | 47 $-7.9382983459e - 02$ |
| 23 $-5.5335005413e - 02$ | 48 $+1.2375963113e - 01$ |
| 24 $-1.2442713148e - 01$ | 49 $-4.4239723203e - 02$ |

$$j = 45: \lambda_{45} = 1.820364e - 19, \quad \ell_{45}(\mathbf{1}) = -1.949302e - 18, \quad \|\hat{v}_{45} - v_{45}\| \leq 9.06e - 138$$

| $k$ $[v_{45}]_k$         | $k$ $[v_{45}]_k$         |
|--------------------------|--------------------------|
| 0 $-3.6464391843e - 20$  | 25 $+1.0830721750e - 01$ |
| 1 $-6.6515600370e - 18$  | 26 $-8.7695665814e - 03$ |
| 2 $-4.4232691798e - 16$  | 27 $-1.1460851863e - 01$ |
| 3 $-1.6920678118e - 14$  | 28 $-5.9314351637e - 02$ |
| 4 $-4.4110474581e - 13$  | 29 $+8.6724001163e - 02$ |
| 5 $-8.5449380907e - 12$  | 30 $+8.9818019020e - 02$ |
| 6 $-1.2952201681e - 10$  | 31 $-6.4843275114e - 02$ |
| 7 $-1.5888568426e - 09$  | 32 $-9.8912895933e - 02$ |
| 8 $-1.6144913664e - 08$  | 33 $+6.0356833291e - 02$ |
| 9 $-1.3816609766e - 07$  | 34 $+9.6150171387e - 02$ |
| 10 $-1.0078383088e - 06$ | 35 $-7.2840416950e - 02$ |
| 11 $-6.3203490854e - 06$ | 36 $-8.0802421022e - 02$ |
| 12 $-3.4278960456e - 05$ | 37 $+9.5933356903e - 02$ |
| 13 $-1.6137550135e - 04$ | 38 $+4.6449050159e - 02$ |
| 14 $-6.6045221973e - 04$ | 39 $-1.1569311707e - 01$ |
| 15 $-2.3484016825e - 03$ | 40 $+1.0318283601e - 02$ |
| 16 $-7.2326419947e - 03$ | 41 $+1.0997245139e - 01$ |
| 17 $-1.9174350563e - 02$ | 42 $-7.7461355722e - 02$ |
| 18 $-4.3290636323e - 02$ | 43 $-5.8337696270e - 02$ |
| 19 $-8.1746562389e - 02$ | 44 $+1.1942750203e - 01$ |
| 20 $-1.2501825496e - 01$ | 45 $-3.3680141764e - 02$ |
| 21 $-1.4495296918e - 01$ | 46 $-9.1826203942e - 02$ |
| 22 $-1.0557149576e - 01$ | 47 $+1.1315918646e - 01$ |
| 23 $-1.6270479417e - 03$ | 48 $-1.1177177539e - 02$ |
| 24 $+1.0349769628e - 01$ | 49 $-1.0250139563e - 01$ |

$$j = 46: \lambda_{46} = -6.941474e - 20, \quad \ell_{46}(\mathbf{1}) = +7.522695e - 19, \quad \|\hat{v}_{46} - v_{46}\| \leq 3.19e - 137$$

| $k$ | $[v_{46}]_k$        | $k$ | $[v_{46}]_k$        |
|-----|---------------------|-----|---------------------|
| 0   | +1.3745452013e - 20 | 25  | -1.2214247149e - 01 |
| 1   | +2.5663249160e - 18 | 26  | -5.8123807757e - 02 |
| 2   | +1.7479049676e - 16 | 27  | +7.4824912988e - 02 |
| 3   | +6.8532116748e - 15 | 28  | +1.0856499971e - 01 |
| 4   | +1.8325947748e - 13 | 29  | -1.5422327161e - 02 |
| 5   | +3.6447129041e - 12 | 30  | -1.1509012861e - 01 |
| 6   | +5.6773957589e - 11 | 31  | -2.0936959961e - 02 |
| 7   | +7.1648901251e - 10 | 32  | +1.1060672870e - 01 |
| 8   | +7.4989835133e - 09 | 33  | +3.3464624156e - 02 |
| 9   | +6.6190838468e - 08 | 34  | -1.0985340360e - 01 |
| 10  | +4.9875064610e - 07 | 35  | -2.6230916871e - 02 |
| 11  | +3.2366305514e - 06 | 36  | +1.1369077725e - 01 |
| 12  | +1.8202191561e - 05 | 37  | +6.1312602032e - 04 |
| 13  | +8.9067183950e - 05 | 38  | -1.1384127669e - 01 |
| 14  | +3.7997132017e - 04 | 39  | +4.1311124674e - 02 |
| 15  | +1.4133048222e - 03 | 40  | +9.5869907991e - 02 |
| 16  | +4.5733687766e - 03 | 41  | -8.8970089990e - 02 |
| 17  | +1.2813030823e - 02 | 42  | -4.6290081716e - 02 |
| 18  | +3.0816803386e - 02 | 43  | +1.1737985860e - 01 |
| 19  | +6.2731135266e - 02 | 44  | -3.2186508228e - 02 |
| 20  | +1.0548749864e - 01 | 45  | -9.4172376779e - 02 |
| 21  | +1.3997645756e - 01 | 46  | +1.0471536340e - 01 |
| 22  | +1.3162602902e - 01 | 47  | +8.5238957340e - 03 |
| 23  | +5.5719138175e - 02 | 48  | -1.1206289962e - 01 |
| 24  | -5.9284844754e - 02 | 49  | +9.3131256057e - 02 |

$$j = 47: \lambda_{47} = 2.647086e - 20, \quad \ell_{47}(\mathbf{1}) = -2.902510e - 19, \quad \|\hat{v}_{47} - v_{47}\| \leq 1.12e - 136$$

| $k$ | $[v_{47}]_k$        | $k$ | $[v_{47}]_k$        |
|-----|---------------------|-----|---------------------|
| 0   | -5.1830220205e - 21 | 25  | +1.0414460268e - 01 |
| 1   | -9.8993946689e - 19 | 26  | +1.0441826271e - 01 |
| 2   | -6.9018090391e - 17 | 27  | -1.0487694706e - 02 |
| 3   | -2.7719673785e - 15 | 28  | -1.1226241839e - 01 |
| 4   | -7.5986887043e - 14 | 29  | -5.9635347769e - 02 |
| 5   | -1.5505137057e - 12 | 30  | +8.2220879855e - 02 |
| 6   | -2.4802784531e - 11 | 31  | +9.1554027465e - 02 |
| 7   | -3.2176701874e - 10 | 32  | -5.6375011890e - 02 |
| 8   | -3.4658270624e - 09 | 33  | -1.0175168246e - 01 |
| 9   | -3.1522879339e - 08 | 34  | +4.7458547183e - 02 |
| 10  | -2.4510777951e - 07 | 35  | +1.0164632685e - 01 |
| 11  | -1.6440735660e - 06 | 36  | -5.6102762416e - 02 |
| 12  | -9.5746504520e - 06 | 37  | -9.2388369359e - 02 |
| 13  | -4.8622971565e - 05 | 38  | +7.8209611828e - 02 |
| 14  | -2.1583927654e - 04 | 39  | +6.8071712986e - 02 |
| 15  | -8.3799493378e - 04 | 40  | -1.0393196879e - 01 |
| 16  | -2.8416451525e - 03 | 41  | -2.2078504266e - 02 |
| 17  | -8.3849452961e - 03 | 42  | +1.1502800030e - 01 |
| 18  | -2.1383974222e - 02 | 43  | -4.2550912506e - 02 |
| 19  | -4.6605627229e - 02 | 44  | -8.8735650778e - 02 |
| 20  | -8.5193114486e - 02 | 45  | +1.0204809177e - 01 |
| 21  | -1.2633276449e - 01 | 46  | +1.5107531162e - 02 |
| 22  | -1.4184860887e - 01 | 47  | -1.1366848947e - 01 |
| 23  | -9.8532750955e - 02 | 48  | +7.7718289123e - 02 |
| 24  | +4.7140404403e - 03 | 49  | +4.6717100523e - 02 |

$$j = 48: \lambda_{48} = -1.009500e - 20, \quad \ell_{48}(\mathbf{1}) = +1.119653e - 19, \quad \|\hat{v}_{48} - v_{48}\| \leq 3.94e - 136$$

| $k$ | $[v_{48}]_k$        | $k$ | $[v_{48}]_k$        |
|-----|---------------------|-----|---------------------|
| 0   | +1.9549473828e - 21 | 25  | -6.3047389138e - 02 |
| 1   | +3.8178450845e - 19 | 26  | -1.1986801850e - 01 |
| 2   | +2.7232854922e - 17 | 27  | -5.4461567168e - 02 |
| 3   | +1.1197621309e - 15 | 28  | +7.4240673941e - 02 |
| 4   | +3.1448312568e - 14 | 29  | +1.0657469089e - 01 |
| 5   | +6.5795941258e - 13 | 30  | -1.2611937046e - 02 |
| 6   | +1.0801071412e - 11 | 31  | -1.1233348232e - 01 |
| 7   | +1.4393566375e - 10 | 32  | -2.6970434842e - 02 |
| 8   | +1.5942549582e - 09 | 33  | +1.0554019483e - 01 |
| 9   | +1.4928574072e - 08 | 34  | +4.3175615250e - 02 |
| 10  | +1.1966665388e - 07 | 35  | -1.0278152008e - 01 |
| 11  | +8.2874522910e - 07 | 36  | -4.0829647022e - 02 |
| 12  | +4.9918647475e - 06 | 37  | +1.0697863400e - 01 |
| 13  | +2.6272335774e - 05 | 38  | +2.1533866628e - 02 |
| 14  | +1.2115395913e - 04 | 39  | -1.1239592731e - 01 |
| 15  | +4.9004564081e - 04 | 40  | +1.4656163488e - 02 |
| 16  | +1.7372880195e - 03 | 41  | +1.0669003746e - 01 |
| 17  | +5.3830460372e - 03 | 42  | -6.2665851601e - 02 |
| 18  | +1.4499833943e - 02 | 43  | -7.4737356576e - 02 |
| 19  | +3.3647458961e - 02 | 44  | +1.0498442188e - 01 |
| 20  | +6.6279836883e - 02 | 45  | +9.5664138661e - 03 |
| 21  | +1.0807992113e - 01 | 46  | -1.1140292274e - 01 |
| 22  | +1.3911868905e - 01 | 47  | +7.0893792005e - 02 |
| 23  | +1.2617270160e - 01 | 48  | +5.6813250795e - 02 |
| 24  | +4.8359915560e - 02 | 49  | -1.1721657727e - 01 |

$$j = 49: \lambda_{49} = 3.850039e - 21, \quad \ell_{49}(\mathbf{1}) = -4.318241e - 20, \quad \|\hat{v}_{49} - v_{49}\| \leq 1.39e - 135$$

| $k$ | $[v_{49}]_k$        | $k$ | $[v_{49}]_k$        |
|-----|---------------------|-----|---------------------|
| 0   | -7.3758060019e - 22 | 25  | +1.0826823066e - 02 |
| 1   | -1.4721233018e - 19 | 26  | +1.0469640064e - 01 |
| 2   | -1.0737965942e - 17 | 27  | +1.0054312788e - 01 |
| 3   | -4.5178469510e - 16 | 28  | -1.2433779041e - 02 |
| 4   | -1.2992086239e - 14 | 29  | -1.1017605640e - 01 |
| 5   | -2.7853737158e - 13 | 30  | -5.9527721262e - 02 |
| 6   | -4.6893527300e - 12 | 31  | +7.8316082656e - 02 |
| 7   | -6.4146289312e - 11 | 32  | +9.2606704498e - 02 |
| 8   | -7.3005497636e - 10 | 33  | -4.8808728001e - 02 |
| 9   | -7.0323074730e - 09 | 34  | -1.0330045406e - 01 |
| 10  | -5.8060415150e - 08 | 35  | +3.5640825386e - 02 |
| 11  | -4.1473605420e - 07 | 36  | +1.0468366235e - 01 |
| 12  | -2.5808327752e - 06 | 37  | -4.0108724312e - 02 |
| 13  | -1.4058920144e - 05 | 38  | -9.9796635173e - 02 |
| 14  | -6.7250200388e - 05 | 39  | +5.9583692232e - 02 |
| 15  | -2.8289142450e - 04 | 40  | +8.3938310178e - 02 |
| 16  | -1.0462764988e - 03 | 41  | -8.7497834450e - 02 |
| 17  | -3.3954138064e - 03 | 42  | -4.9226783080e - 02 |
| 18  | -9.6273325470e - 03 | 43  | +1.0999198153e - 01 |
| 19  | -2.3676907698e - 02 | 44  | -7.4625644434e - 03 |
| 20  | -4.9914679595e - 02 | 45  | -1.0571458797e - 01 |
| 21  | -8.8466683314e - 02 | 46  | +7.3398323310e - 02 |
| 22  | -1.2734810290e - 01 | 47  | +5.6196323014e - 02 |
| 23  | -1.3852730907e - 01 | 48  | -1.1402183084e - 01 |
| 24  | -9.1552344183e - 02 | 49  | +3.1567831525e - 02 |

$$j = 50: \lambda_{50} = -1.468398e - 21, \quad \ell_{50}(\mathbf{1}) = +1.665125e - 20, \quad \|\hat{v}_{50} - v_{50}\| \leq 4.88e - 135$$

| $k$ | $[v_{50}]_k$          | $k$ | $[v_{50}]_k$          |
|-----|-----------------------|-----|-----------------------|
| 0   | $+2.7835629669e - 22$ | 25  | $+4.1177360547e - 02$ |
| 1   | $+5.6753106159e - 20$ | 26  | $-6.6614545461e - 02$ |
| 2   | $+4.2311862301e - 18$ | 27  | $-1.1757833392e - 01$ |
| 3   | $+1.8206570357e - 16$ | 28  | $-5.0730345707e - 02$ |
| 4   | $+5.3581796698e - 15$ | 29  | $+7.3957717244e - 02$ |
| 5   | $+1.1764542595e - 13$ | 30  | $+1.0456374951e - 01$ |
| 6   | $+2.0300126303e - 12$ | 31  | $-1.0451352936e - 02$ |
| 7   | $+2.8485674436e - 11$ | 32  | $-1.0966386661e - 01$ |
| 8   | $+3.3288442366e - 10$ | 33  | $-3.1942392723e - 02$ |
| 9   | $+3.2959293692e - 09$ | 34  | $+1.0047453126e - 01$ |
| 10  | $+2.8003675784e - 08$ | 35  | $+5.1183706820e - 02$ |
| 11  | $+2.0612860068e - 07$ | 36  | $-9.5196677880e - 02$ |
| 12  | $+1.3237690384e - 06$ | 37  | $-5.2883204656e - 02$ |
| 13  | $+7.4548749103e - 06$ | 38  | $+9.8437726306e - 02$ |
| 14  | $+3.6939313233e - 05$ | 39  | $+3.9324624158e - 02$ |
| 15  | $+1.6134225449e - 04$ | 40  | $-1.0665078190e - 01$ |
| 16  | $+6.2135557393e - 04$ | 41  | $-9.6781119087e - 03$ |
| 17  | $+2.1070097985e - 03$ | 42  | $+1.0994674614e - 01$ |
| 18  | $+6.2701608076e - 03$ | 43  | $-3.4856680135e - 02$ |
| 19  | $+1.6278920016e - 02$ | 44  | $-9.3744041071e - 02$ |
| 20  | $+3.6523884116e - 02$ | 45  | $+8.3673593441e - 02$ |
| 21  | $+6.9739111552e - 02$ | 46  | $+4.5625655594e - 02$ |
| 22  | $+1.1041937685e - 01$ | 47  | $-1.1225370696e - 01$ |
| 23  | $+1.3797537308e - 01$ | 48  | $+3.0294155178e - 02$ |
| 24  | $+1.2063280321e - 01$ | 49  | $+9.0312194250e - 02$ |

## Tail Bound for the Spectral Remainder

The spectral expansion (S1) has remainder

$$R_N(n) = L^n \mathbf{1} - \sum_{j=1}^N \lambda_j^n \ell_j(\mathbf{1}) v_j.$$

We bound  $\|R_N(n)\|$  by combining the Cauchy integral formula with a direct computation of the *tail projection*  $Q_N \mathbf{1}$ , where  $Q_N = I - \sum_{j=1}^N P_j$  is the tail spectral projector.

**Factored tail bound.** Since  $Q_N$  commutes with  $L$  (Riesz projectors commute with the operator, regardless of normality), we have the factorization

$$R_N(n) = Q_N L^n \mathbf{1} = (Q_N L^n)(Q_N \mathbf{1}),$$

using only  $Q_N^2 = Q_N$  (Riesz idempotency) and  $L$ -invariance of  $\text{range}(Q_N)$ . The Cauchy integral on a circle  $\Gamma = \{|z| = \rho\}$  in the eigenvalue gap  $|\lambda_{N+1}| < \rho < |\lambda_N|$  bounds the operator factor:

$$\|Q_N L^n\| = \left\| \frac{1}{2\pi i} \oint_{\Gamma} z^n R_L(z) dz \right\| \leq \rho^{n+1} \cdot M_{\infty},$$

where  $M_{\infty} = \sup_{z \in \Gamma} \|R_L(z)\|$  is obtained via the resolvent perturbation bound. The tail projection  $\|Q_N \mathbf{1}\| = \|\mathbf{1} - \sum_{j=1}^N P_j \mathbf{1}\|$  is computed directly from the rigorous spectral coefficients.

The combined bound is:

$$\|R_N(n)\| \leq \rho^{n+1} \cdot M_{\infty} \cdot \|Q_N \mathbf{1}\|.$$

**Tail bound at  $N = 50$ .** Using all  $N = 50$  certified eigenvalues, the separating contour  $\Gamma$  lies in the eigenvalue gap  $|\lambda_{51}| < \rho < |\lambda_{50}|$ , with  $|\lambda_{50}| \approx 1.47 \times 10^{-21}$  and  $|\lambda_{51}| \approx 5.60 \times 10^{-22}$ . The resolvent on this circle is certified via the block Schur method from the ordered Schur form at  $K = 256$  (Phase 3 of the full certification pipeline). The tail projection  $Q_{50} \mathbf{1}$  is computed at  $K = 1024$  (2048-bit precision) using the certified  $\ell_j(\mathbf{1})$  and Schur eigenvectors; the correction for the infinite-dimensional lift ( $N \cdot \varepsilon_{1024}/\text{sep}_{\min}$ ) is negligible compared to the Galerkin norm.

Table S7: Tail bound parameters for the spectral remainder  $R_{50}(n)$ . Resolvent certified at  $K = 256$ ; tail projection  $\|Q_{50} \mathbf{1}\|$  computed at  $K = 1024$ .

| Parameter                                              | Value                      |
|--------------------------------------------------------|----------------------------|
| $ \lambda_{50} $                                       | $1.468398 \times 10^{-21}$ |
| $ \lambda_{51} $                                       | $5.600685 \times 10^{-22}$ |
| Circle radius $\rho$                                   | $1.014211 \times 10^{-21}$ |
| $M_{\infty} = \ R_L\ $ on $\Gamma$                     | $6.0617 \times 10^{41}$    |
| $\ Q_{50} \mathbf{1}\ $                                | $6.1383 \times 10^{-21}$   |
| Prefactor $C = M_{\infty} \cdot \ Q_{50} \mathbf{1}\ $ | $3.7208 \times 10^{21}$    |

**Comparison with  $N = 20$ .** For comparison, the tail bound at  $N = 20$  (resolvent certified at  $K = 64$ , tail projection at  $K = 256$ ) gives  $\rho_{20} = 3.81 \times 10^{-9}$ ,  $M_{\infty} = 3.61 \times 10^9$ ,  $\|Q_{20} \mathbf{1}\| = 3.64 \times 10^{-1}$ , and prefactor  $C_{20} = 1.32 \times 10^9$ . The  $N = 50$  tail circle is  $10^{12}$  times smaller in radius, yielding bounds that are stronger by a factor of  $\sim 10^{12(n+1)}$ .

Table S8: Rigorous upper bounds on  $\|R_{50}(n)\| \leq \rho^{n+1} \cdot M_\infty \cdot \|Q_{50}\mathbf{1}\|$ .

| $n$ | $\ R_{50}(n)\  \leq$ |
|-----|----------------------|
| 1   | $< 10^{-20}$         |
| 2   | $< 10^{-41}$         |
| 5   | $< 10^{-104}$        |
| 10  | $< 10^{-209}$        |
| 20  | $< 10^{-419}$        |
| 50  | $< 10^{-1049}$       |
| 100 | $< 10^{-2099}$       |

## Integrated Spectral Expansion

The tail bound provides a rigorous  $L^\infty$  certificate for the integrated spectral expansion. Define

$$F_n^{(j_0)}(x) = \int_0^x \sum_{j=j_0}^N \lambda_j^n \ell_j(\mathbf{1}) v_j(t) dt,$$

which represents the contribution of modes  $j \geq j_0$  to the antiderivative of  $L^n \mathbf{1}$ . For  $j_0 = 2$ , this measures the integrated deviation of  $L^n \mathbf{1}$  from its equilibrium  $\ell_1(\mathbf{1}) v_1$ . Removing additional dominant eigenfunctions reveals progressively finer structure linked to the Gauss map's Markov partition.

The integration  $\int_0^x$  can be computed exactly in the shifted monomial basis:  $\int_0^x (t-1)^k dt = ((x-1)^{k+1} - (-1)^{k+1})/(k+1)$ . The  $L^\infty$  error bound follows from Cauchy–Schwarz and the Gram matrix of the shifted monomial basis  $\{(x-1)^k\}$  on  $[0, 1]$  (whose spectral norm equals that of the Hilbert matrix,  $\leq \pi$ ):

$$\left| F_n^{(j_0)}(x) - \int_0^x \left( L^n \mathbf{1}(t) - \sum_{j=1}^{j_0-1} \lambda_j^n P_j \mathbf{1}(t) \right) dt \right| \leq \sqrt{\pi} \|R_N(n)\| \leq \sqrt{\pi} \rho^{n+1} \cdot C.$$

Table S9: Signal amplitude  $\max_x |F_n^{(j_0)}(x)|$  by mode cutoff  $j_0$  and iterate  $n$ , with rigorous  $L^\infty$  error bounds.

| $j_0$                  | Dominant $\lambda_{j_0}$ | $n = 1$              | $n = 2$              | $n = 5$               |
|------------------------|--------------------------|----------------------|----------------------|-----------------------|
| 2                      | -0.3037                  | $3.0 \times 10^{-2}$ | $8.7 \times 10^{-3}$ | $2.5 \times 10^{-4}$  |
| 3                      | 0.1009                   | $1.8 \times 10^{-3}$ | $1.7 \times 10^{-4}$ | $1.8 \times 10^{-7}$  |
| 4                      | -0.0355                  | $1.6 \times 10^{-4}$ | $5.0 \times 10^{-6}$ | $2.3 \times 10^{-10}$ |
| 5                      | 0.0128                   | $1.6 \times 10^{-5}$ | $1.8 \times 10^{-7}$ | $4.0 \times 10^{-13}$ |
| 6                      | -0.0047                  | $1.8 \times 10^{-6}$ | $7.2 \times 10^{-9}$ | $7.9 \times 10^{-16}$ |
| $L^\infty$ error bound |                          | $\leq 10^{-21}$      | $\leq 10^{-42}$      | $\leq 10^{-105}$      |

Figure S14 shows  $F_n^{(j_0)}$  for  $j_0 = 2, \dots, 6$  and  $n = 1, 2, 5$ . As more dominant eigenfunctions are removed, the Markov partition structure of the Gauss map becomes increasingly visible: for  $j_0 \geq 4$ , the peaks of  $F_n^{(j_0)}$  concentrate near  $x \approx 1/k$ , reflecting the cylinder boundaries  $I_k = [1/(k+1), 1/k]$ . The amplitude decreases by roughly a factor of  $|\lambda_{j_0}/\lambda_{j_0-1}| \approx 1/3$  per removed mode. Even at the

smallest amplitudes ( $\sim 10^{-16}$  for  $j_0 = 6$ ,  $n = 5$ ), the  $L^\infty$  error bound ( $\leq 10^{-105}$ ) remains more than 80 orders of magnitude below the signal, confirming that the plotted curves are rigorous to plotting accuracy.

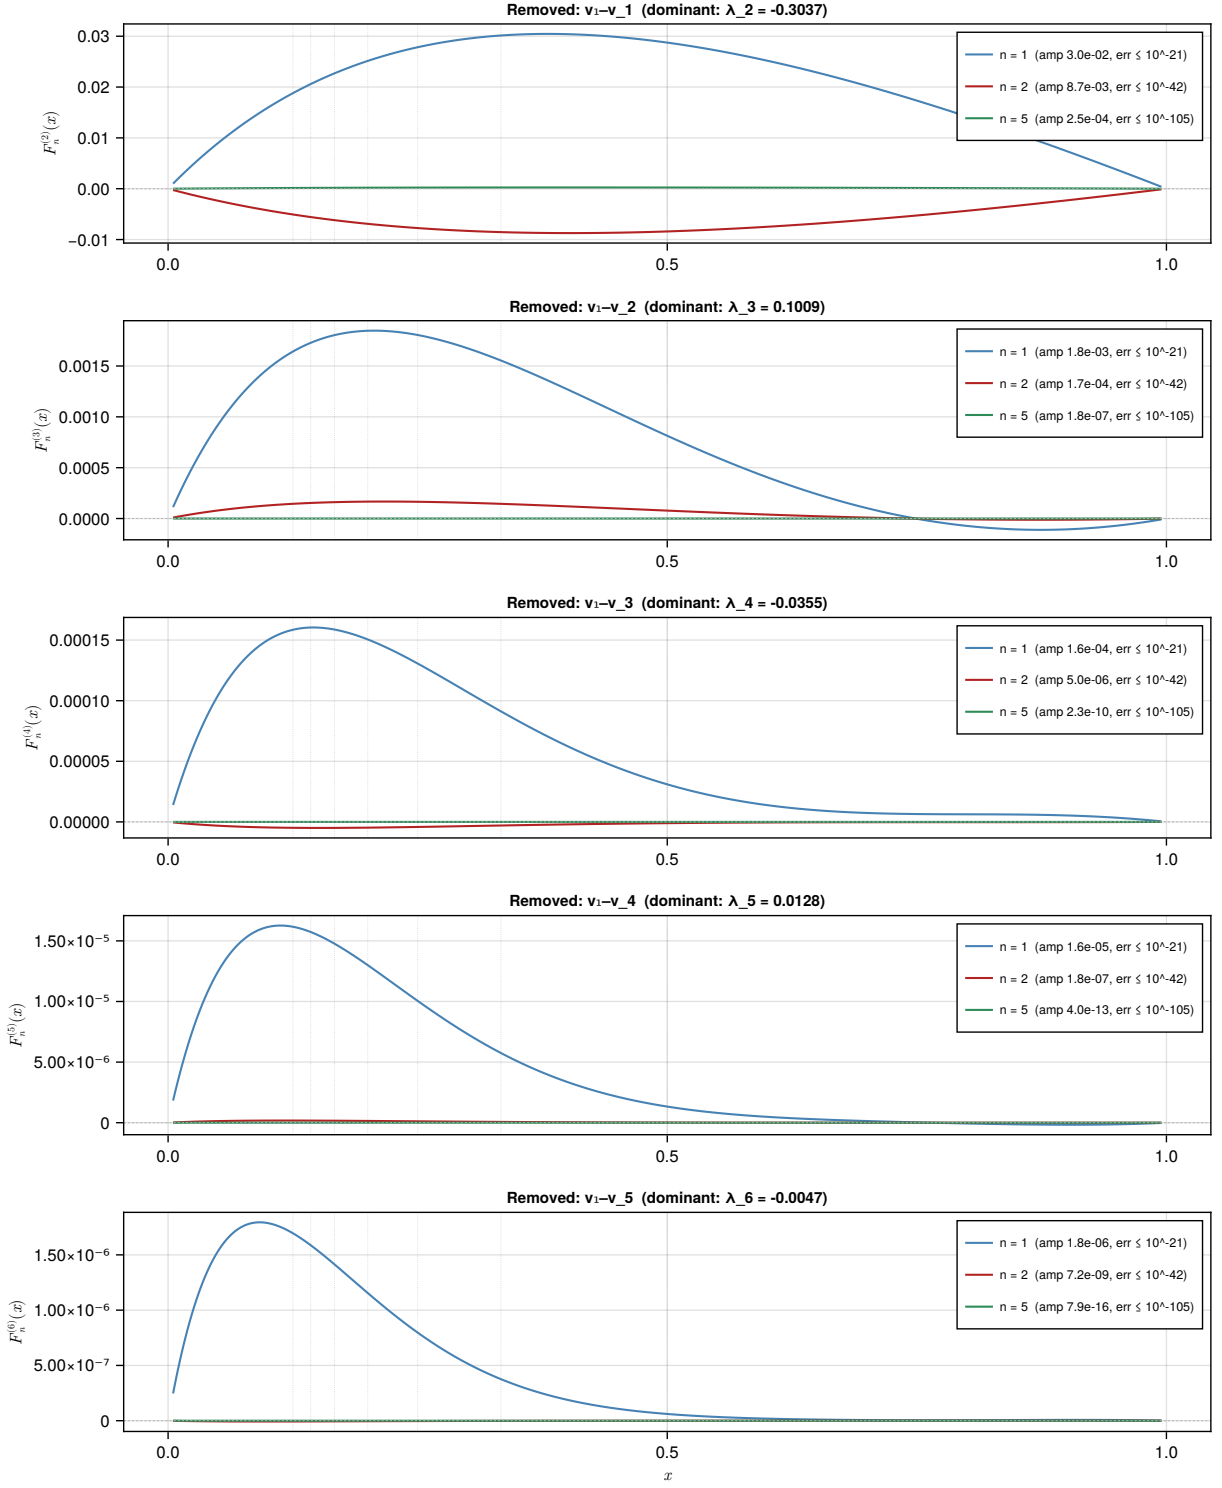

Figure S14: Integrated spectral expansion  $F_n^{(j_0)}(x) = \int_0^x \sum_{j \geq j_0} \lambda_j^n \ell_j(\mathbf{1}) v_j(t) dt$  with the first  $j_0 - 1$  eigenfunctions cumulatively removed. Each panel shows  $n = 1$  (blue),  $n = 2$  (red),  $n = 5$  (green). Dotted vertical lines mark the Markov partition boundaries  $x = 1/k$ .

## Eigenfunction Structure and the Markov Partition

The Gauss map  $G(x) = \{1/x\}$  admits a countable Markov partition into cylinders  $I_n = [1/(n+1), 1/n]$  for  $n = 1, 2, 3, \dots$ . We investigate the relationship between the eigenfunctions  $v_j$  and this partition by analysing zero crossings and local extrema.

**Zero crossings.** The invariant density  $v_1$  is strictly positive on  $(0, 1)$ , as expected. For  $j \geq 2$ , the eigenfunction  $v_j$  has a small number of zero crossings: odd-indexed eigenfunctions typically have 2 zeros, even-indexed have 1 or 3. The first zero of  $v_j$  sits near  $x \approx 1/j$ , matching the left endpoint of the cylinder  $I_{j-1}$ . For  $j \gtrsim 40$ , the polynomial representation in the shifted monomial basis  $\{(x-1)^k\}$  develops spurious Runge-type oscillations at Float64 precision, producing artificially many zero crossings (e.g.,  $\sim 2900$  for  $v_{50}$ ).

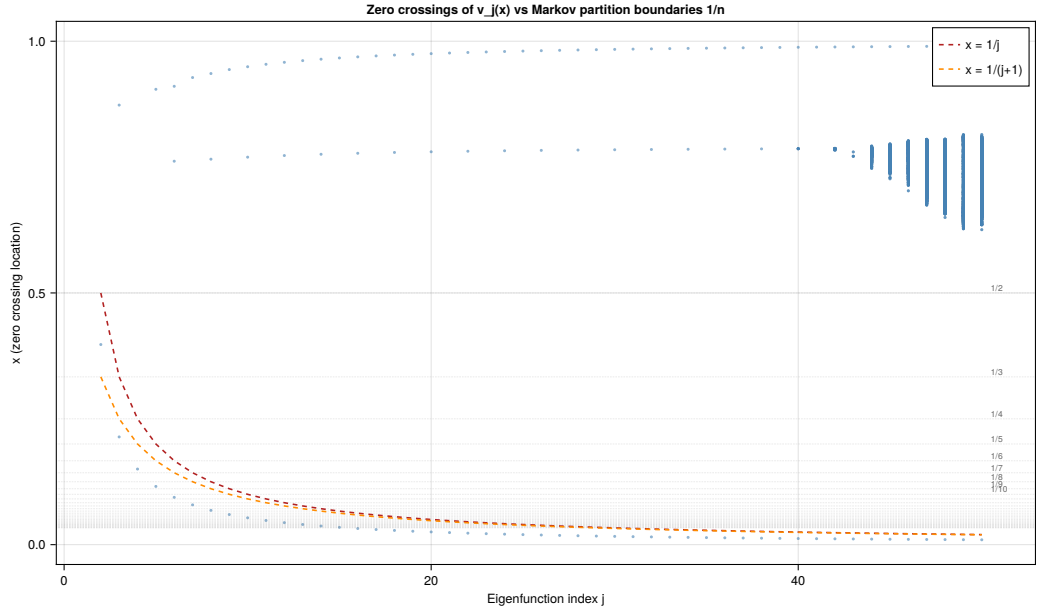

Figure S15: Zero crossing locations of  $v_j(x)$  (blue dots) versus Markov partition boundaries  $x = 1/n$  (dotted grey). The reference curves  $x = 1/j$  (red dashed) and  $x = 1/(j+1)$  (orange dashed) are shown.

**Dominant local extremum.** For each  $j \geq 3$ , the largest local extremum (in absolute value) of  $v_j$  is located near the Markov boundary  $x = 1/j$ :

$$x_{\max}(v_j) \approx \frac{1}{j}.$$

For  $j = 3, \dots, 24$ , the extremum lies slightly above  $1/j$ , inside  $I_{j-1} = [1/j, 1/(j-1)]$ ; for  $j \geq 25$ , it drifts slightly below  $1/j$ , into  $I_j = [1/(j+1), 1/j]$ . The relative error  $|x_{\max}(v_j) - 1/j|/(1/j)$  is tabulated below for selected  $j$ :

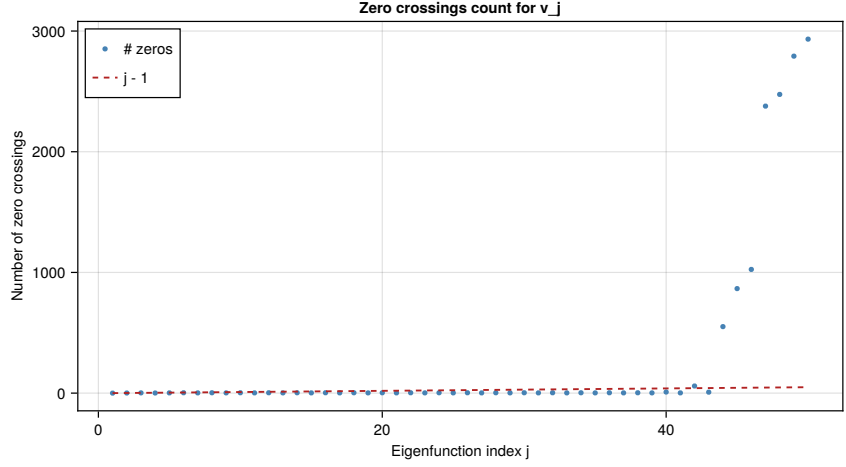

Figure S16: Number of zero crossings of  $v_j$  versus  $j$ . For  $j \leq 39$  the count stays at 1–3; the explosion for  $j \geq 40$  is a Runge artefact of the polynomial basis at Float64 precision.

| $j$ | $x_{\max}(v_j)$ | $1/j$   | rel. error | cylinder |
|-----|-----------------|---------|------------|----------|
| 3   | 0.45498         | 0.33333 | 36.5%      | $I_2$    |
| 5   | 0.23258         | 0.20000 | 16.3%      | $I_4$    |
| 10  | 0.10663         | 0.10000 | 6.6%       | $I_9$    |
| 20  | 0.05056         | 0.05000 | 1.1%       | $I_{19}$ |
| 30  | 0.03296         | 0.03333 | 1.1%       | $I_{30}$ |
| 40  | 0.02439         | 0.02500 | 2.4%       | $I_{40}$ |
| 50  | 0.01932         | 0.02000 | 3.4%       | $I_{51}$ |

For  $j \geq 10$  the mean relative error is 2.3% (std. dev. 1.5%); for  $j \geq 20$  it is 1.8% (std. dev. 1.1%). Each eigenfunction is thus “tuned” to the Markov boundary  $x = 1/j$ , confirming that higher eigenmodes encode progressively finer partition structure.

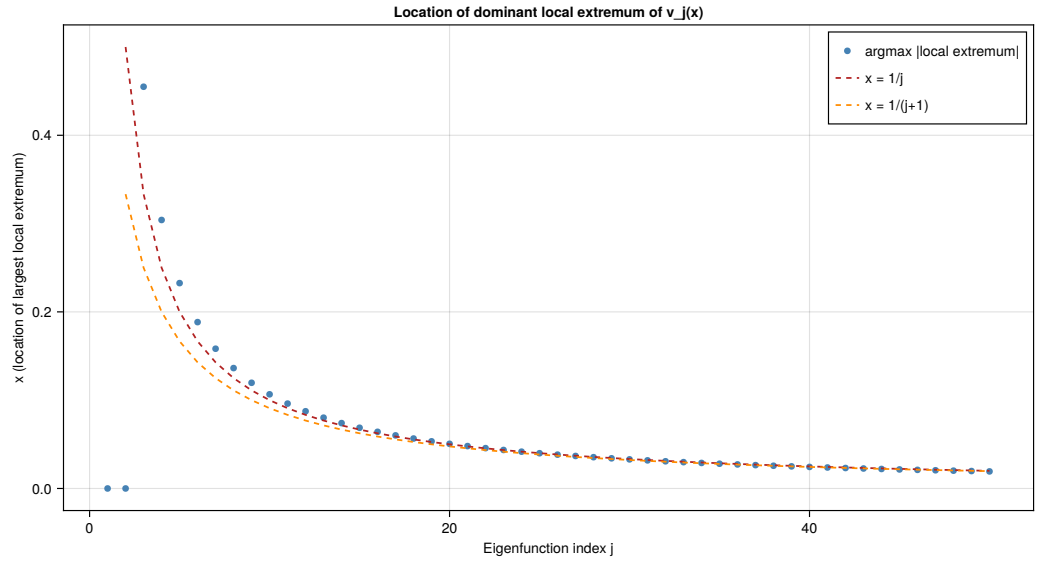

Figure S17: Location of the dominant local extremum of  $v_j(x)$  (blue dots) compared with  $x = 1/j$  (red dashed) and  $x = 1/(j + 1)$  (orange dashed). For  $j \geq 10$  the extremum tracks  $1/j$  with  $\sim 2\%$  relative error.

## Non-Normality of the Transfer Operator

The GKW transfer operator is not normal, so its Schur decomposition  $A = QTQ^*$  has a non-trivial strictly upper triangular part. We quantify this non-normality using the ordered Schur form with eigenvalues sorted by decreasing  $|\lambda_j|$  on the diagonal ( $K = 1024$ ,  $n = 1025$ ).

**Henrici departure from normality.** The Henrici number

$$\delta_H = \frac{\|T - \text{diag}(T)\|_F}{\|T\|_F} = 3.82 \times 10^{-1}$$

indicates that roughly 38% of the Frobenius norm of  $T$  resides in the off-diagonal entries, confirming significant non-normality.

**Coupling structure.** For fixed row  $i$ , the entry  $T_{ij}$  with  $j > i$  quantifies the coupling from Schur mode  $j$  (smaller  $|\lambda_j|$ ) back into mode  $i$  (larger  $|\lambda_i|$ ). Figure S18 shows the full  $80 \times 80$  heatmap of  $\log_{10} |T_{ij}|$ ; Figure S19 displays the row profiles  $|T_{i,j}|$  for selected  $i$ .

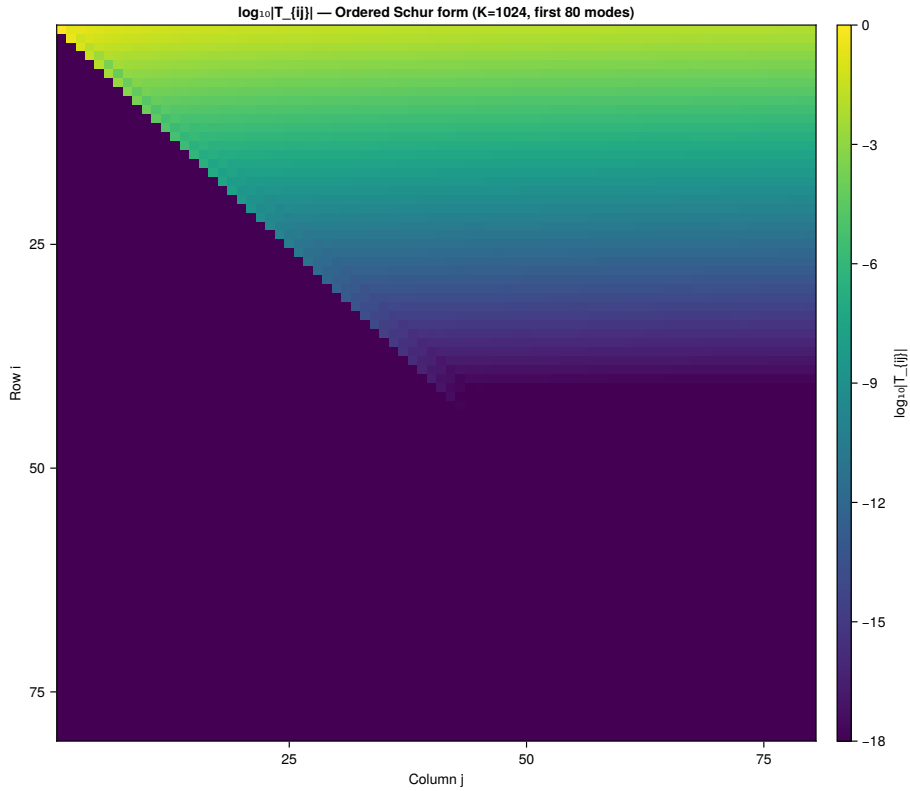

Figure S18: Heatmap of  $\log_{10} |T_{ij}|$  in the ordered Schur form (eigenvalues sorted by decreasing  $|\lambda|$ , first 80 modes). The diagonal contains the eigenvalues; the upper triangular entries encode non-normal coupling between modes.

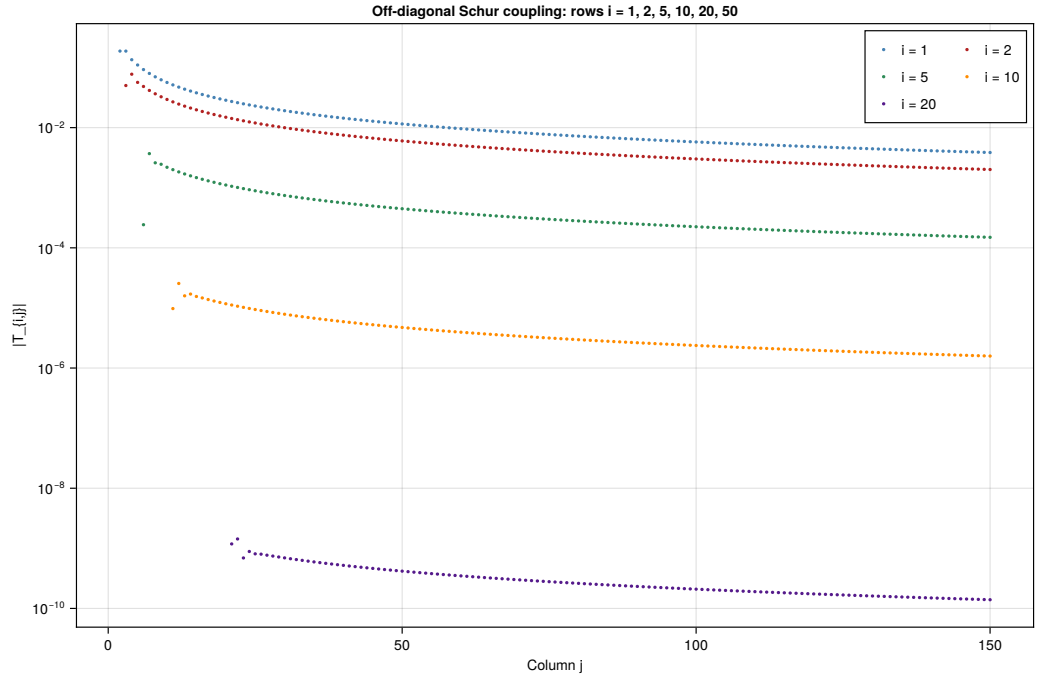

Figure S19: Off-diagonal Schur coupling  $|T_{i,j}|$  for rows  $i = 1, 2, 5, 10, 20, 50$  (log scale). Mode  $j$  feeds back into mode  $i$  with strength  $|T_{i,j}|$ .

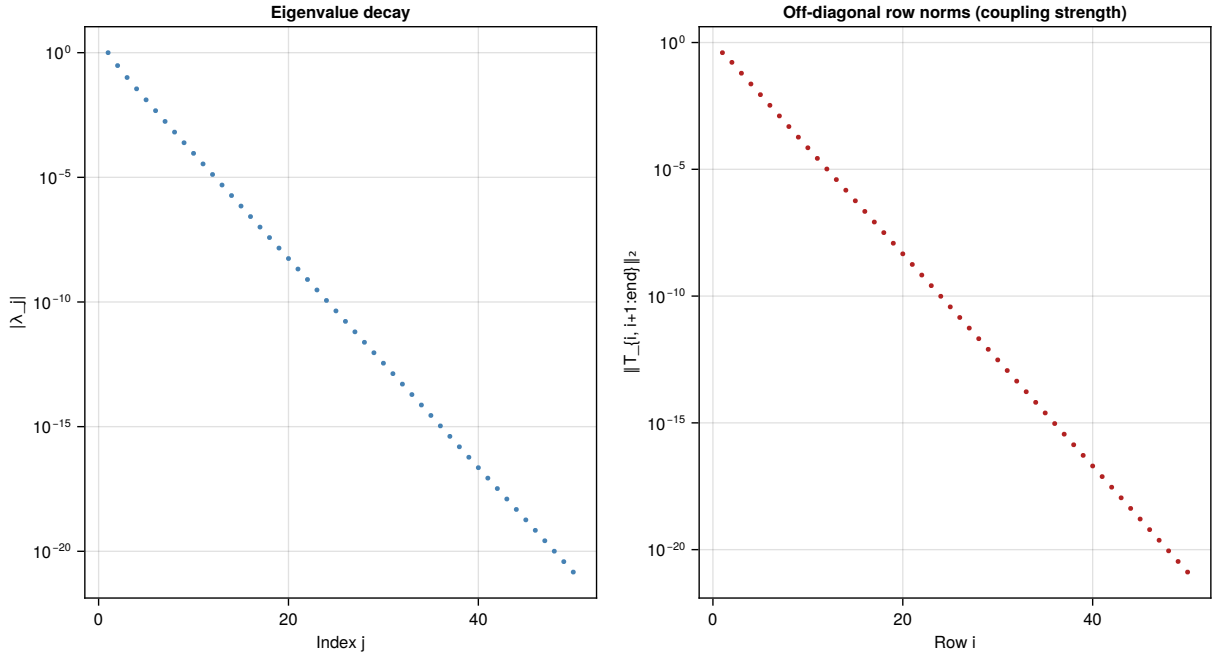

Figure S20: Left: eigenvalue decay  $|\lambda_j|$  versus index  $j$ . Right: off-diagonal row norms  $\|T_{i,i+1:n}\|_2$  measuring the total coupling strength from all higher modes into mode  $i$ .
